# Supplementary material for: HISS, a new tool for H I stacking: application to NIBLES spectra
Source: arXiv:1908.00517 source file (2019-08-01)
Supplement: Supplementary file 1 [file SupplementaryMatrial.pdf]

## Supplementary Material: The H I non-detected catalogue

Table 1: Data for the H I non-detections in the stacking sample.

| Source | RA          | Dec          | Name                    | $V_{\text{opt}}$   | $u - r$ | $M_r$  | $M_{\star}$<br>[log]<br>$M_{\odot}$ |
|--------|-------------|--------------|-------------------------|--------------------|---------|--------|-------------------------------------|
|        | (J2000)     |              |                         | $\text{km s}^{-1}$ | mag     | mag    |                                     |
| 1926   | 11 23 18.84 | 03 57 18.78  | CGCG 039-161            | $1582 \pm 19$      | 1.91    | -16.18 | 8.23                                |
| 1954   | 11 49 12.79 | -03 39 34.64 | PGC 1068442             | $1572 \pm 3$       | 1.57    | -15.78 | 8.04                                |
| 2012   | 12 19 21.12 | 04 46 24.49  | ASK 173829              | $2065 \pm 2$       | 1.61    | -15.87 | 8.09                                |
| 2244   | 14 04 15.84 | 04 06 43.85  | UGC 08986               | $1239 \pm 3$       | 2.19    | -17.79 | 9.08                                |
| 2272   | 14 25 08.99 | -01 06 48.52 | CGCG 019-019            | $2643 \pm 3$       | 2.11    | -17.94 | 9.21                                |
| 2442   | 15 17 29.45 | 03 35 07.94  | PGC 3124577             | $1882 \pm 2$       | 1.62    | -15.69 | 8.03                                |
| 2525   | 09 35 44.04 | 31 42 19.68  | NGC 2918                | $6756 \pm 2$       | 2.65    | -22.64 | 11.28                               |
| 2533   | 10 06 07.44 | 47 15 45.53  | NGC 3111                | $7437 \pm 2$       | 2.68    | -22.52 | 11.19                               |
| 2535   | 14 30 25.58 | 11 55 40.77  | NGC 5644                | $7649 \pm 2$       | 2.72    | -22.87 | 11.33                               |
| 2541   | 13 53 38.43 | 36 08 02.57  | NGC 5352                | $7956 \pm 3$       | 2.81    | -22.64 | 11.26                               |
| 2565   | 00 35 59.83 | -10 07 18.07 | NGC 0163                | $5917 \pm 4$       | 2.70    | -22.05 | 11.01                               |
| 2574   | 11 00 35.40 | 12 09 41.65  | NGC 3491                | $6351 \pm 2$       | 2.72    | -21.98 | 11.06                               |
| 2589   | 12 19 32.09 | 49 48 56.71  | UGC 07367               | $4093 \pm 2$       | 2.60    | -21.45 | 10.78                               |
| 2597   | 12 19 32.59 | 56 44 11.69  | NGC 4271                | $4756 \pm 2$       | 2.82    | -21.84 | 10.93                               |
| 2606   | 14 41 32.96 | 38 51 04.95  | UGC 09473               | $4669 \pm 2$       | 2.17    | -21.54 | 10.80                               |
| 2614   | 12 12 17.27 | 13 12 18.72  | NGC 4168                | $2273 \pm 2$       | 2.44    | -21.43 | 10.63                               |
| 2615   | 12 32 47.65 | 63 56 21.18  | NGC 4512                | $2516 \pm 1$       | 2.72    | -20.75 | 10.60                               |
| 2661   | 10 36 38.44 | 14 10 15.97  | NGC 3300                | $3017 \pm 1$       | 2.54    | -21.02 | 10.53                               |
| 2675   | 12 08 09.62 | 10 22 43.96  | NGC 4119                | $1651 \pm 2$       | 2.28    | -19.74 | 10.05                               |
| 2682   | 12 27 13.34 | 12 44 05.22  | NGC 4425                | $1891 \pm 1$       | 2.39    | -20.42 | 10.22                               |
| 2688   | 12 24 05.01 | 11 13 05.04  | NGC 4352                | $2083 \pm 1$       | 2.36    | -20.12 | 10.08                               |
| 2710   | 12 27 02.54 | 15 27 41.34  | NGC 4421                | $1551 \pm 1$       | 2.58    | -20.15 | 10.04                               |
| 2715   | 14 05 12.42 | 55 44 30.67  | NGC 5475                | $1647 \pm 1$       | 2.54    | -19.58 | 9.98                                |
| 2731   | 12 37 48.38 | 05 22 06.69  | NGC 4580                | $1035 \pm 2$       | 2.37    | -19.23 | 9.75                                |
| 2742   | 12 15 59.87 | 66 13 51.00  | NGC 4221                | $1314 \pm 1$       | 2.51    | -19.48 | 9.83                                |
| 2743   | 10 12 41.25 | 03 07 45.79  | NGC 3156                | $1266 \pm 29$      | 1.99    | -19.14 | 9.42                                |
| 2744   | 11 06 32.10 | 11 23 07.51  | NGC 3524                | $1357 \pm 1$       | 2.36    | -19.08 | 9.71                                |
| 2756   | 11 08 40.38 | 57 13 48.71  | NGC 3530                | $1876 \pm 1$       | 2.42    | -18.95 | 9.69                                |
| 2769   | 12 25 18.78 | 64 56 00.52  | NGC 4391                | $1320 \pm 1$       | 2.52    | -18.73 | 9.58                                |
| 2770   | 13 00 10.57 | 12 28 59.92  | NGC 4880                | $1362 \pm 3$       | 2.24    | -19.29 | 9.51                                |
| 2775   | 12 22 04.11 | 12 47 14.95  | NGC 4306                | $1520 \pm 3$       | 2.21    | -18.70 | 9.35                                |
| 2789   | 11 21 24.99 | 03 00 50.23  | NGC 3643                | $1742 \pm 2$       | 2.28    | -18.67 | 9.53                                |
| 2790   | 12 38 17.87 | 13 06 35.64  | NGC 4584                | $1715 \pm 3$       | 2.01    | -18.96 | 9.46                                |
| 2795   | 12 41 59.35 | 12 56 34.27  | NGC 4620                | $1125 \pm 3$       | 2.09    | -18.63 | 9.24                                |
| 2798   | 15 06 35.03 | 02 00 18.38  | NGC 5841                | $1256 \pm 1$       | 2.34    | -18.19 | 9.13                                |
| 2805   | 12 48 55.36 | 14 54 28.40  | IC 3806                 | $1401 \pm 5$       | 2.14    | -18.21 | 9.31                                |
| 2831   | 12 32 14.21 | 10 15 05.18  | IC 3468                 | $1300 \pm 4$       | 2.18    | -18.52 | 9.15                                |
| 2890   | 12 11 07.76 | 14 16 29.33  | IC 3032                 | $1184 \pm 5$       | 2.02    | -16.83 | 8.55                                |
| 2891   | 13 55 38.75 | 04 59 06.18  | NGC 5360                | $1180 \pm 3$       | 1.72    | -16.84 | 8.32                                |
| 2899   | 12 17 01.11 | 09 24 27.19  | IC 3097                 | $1253 \pm 7$       | 1.94    | -16.88 | 8.63                                |
| 2906   | 12 16 52.36 | 14 30 52.50  | IC 3096                 | $1264 \pm 3$       | 1.84    | -17.03 | 8.57                                |
| 2910   | 12 10 12.57 | 64 45 38.33  | MCG +11-15-032          | $1349 \pm 5$       | 1.89    | -16.76 | 8.44                                |
| 2914   | 12 33 13.43 | 09 23 50.50  | IC 3487                 | $1074 \pm 4$       | 1.78    | -16.45 | 8.34                                |
| 2915   | 12 16 09.06 | 12 41 28.68  | IC 3081                 | $1103 \pm 4$       | 2.01    | -16.34 | 8.50                                |
| 2961   | 12 32 39.01 | 10 05 31.46  | VCC 1446                | $1196 \pm 13$      | 2.00    | -15.83 | 8.19                                |
| 2962   | 12 12 18.99 | 15 28 59.14  | VCC 0050                | $1209 \pm 12$      | 1.85    | -15.87 | 8.13                                |
| 2979   | 12 16 02.22 | 46 43 58.32  | MCG +08-22-086          | $1061 \pm 7$       | 1.96    | -15.62 | 8.04                                |
| 2984   | 12 52 33.75 | -01 43 48.75 | ASK 14845               | $1129 \pm 3$       | 1.74    | -15.77 | 8.04                                |
| 2985   | 12 22 50.85 | 13 35 34.31  | VCC 0592                | $1102 \pm 8$       | 2.09    | -15.43 | 8.08                                |
| 2996   | 12 24 05.26 | 10 04 03.89  | PGC 40315               | $1370 \pm 29$      | 2.15    | -16.05 | 8.13                                |
| 3306   | 23 20 28.21 | 15 04 20.91  | 2MASX J23202822+1504211 | $3828 \pm 2$       | 2.30    | -18.77 | 9.57                                |
| 3346   | 00 25 52.49 | -09 39 42.37 | 2MASXJ00255209-0939420  | $5201 \pm 2$       | 2.65    | -20.78 | 10.54                               |

Table 1: continued from previous page

| Source | RA          | Dec          | Name                    | $V_{\text{opt}}$   | $u - r$ | $M_r$  | $M_{\star}$          |
|--------|-------------|--------------|-------------------------|--------------------|---------|--------|----------------------|
|        | (J2000)     |              |                         | $\text{km s}^{-1}$ | mag     | mag    | [log]<br>$M_{\odot}$ |
| 3348   | 00 12 06.10 | 00 24 54.76  | IC 0003                 | $5447 \pm 2$       | 2.63    | -21.14 | 10.61                |
| 3371   | 03 34 17.75 | -06 15 53.99 | NGC 1361                | $5254 \pm 2$       | 2.60    | -21.44 | 10.73                |
| 3381   | 07 36 16.80 | 33 07 21.76  | IC 2201                 | $4694 \pm 1$       | 2.79    | -20.54 | 10.59                |
| 3387   | 08 25 17.47 | 03 56 00.90  | CGCG 032-022            | $4169 \pm 2$       | 2.45    | -20.26 | 10.19                |
| 3388   | 04 06 14.72 | -05 39 06.84 | IC 2031                 | $4823 \pm 3$       | 1.68    | -20.01 | 10.05                |
| 3406   | 00 04 35.22 | 00 50 54.98  | 2MASX J00043518+0050549 | $6392 \pm 4$       | 2.17    | -18.54 | 9.57                 |
| 3407   | 00 09 40.24 | -10 25 02.71 | 2MASX J00094023-1025027 | $5415 \pm 2$       | 1.46    | -18.43 | 9.12                 |
| 3411   | 00 13 45.42 | -09 56 03.67 | ASK 126038              | $3822 \pm 2$       | 1.38    | -16.79 | 8.24                 |
| 3423   | 00 51 49.41 | 00 33 53.22  | UM 283                  | $4629 \pm 0$       | 1.08    | -18.05 | 8.53                 |
| 3434   | 04 10 51.37 | -05 13 19.97 | ASK 57849               | $4868 \pm 3$       | 1.37    | -17.48 | 8.39                 |
| 3439   | 07 40 22.74 | 23 16 29.95  | UGC 03960               | $2255 \pm 2$       | 2.31    | -19.36 | 9.77                 |
| 3459   | 08 47 21.99 | 42 23 55.65  | ASK 191682              | $2980 \pm 1$       | 1.26    | -16.13 | 8.03                 |
| 3461   | 08 47 59.49 | 19 02 56.44  | PGC 1578852             | $3844 \pm 2$       | 1.86    | -17.20 | 8.50                 |
| 3478   | 13 36 20.08 | 38 06 53.60  | ASK 508595              | $5157 \pm 2$       | 1.40    | -17.37 | 8.53                 |
| 3483   | 13 39 03.16 | 43 33 58.60  | CGCG 218-031            | $2740 \pm 2$       | 2.41    | -18.94 | 9.71                 |
| 3491   | 09 08 54.37 | 01 25 57.21  | CGCG 006-006            | $4918 \pm 3$       | 1.68    | -19.00 | 9.30                 |
| 3495   | 14 13 21.79 | 54 40 06.27  | MCG +09-23-057          | $2059 \pm 8$       | 1.70    | -16.58 | 8.28                 |
| 3498   | 14 19 29.09 | 35 34 01.11  | ASK 392553              | $3207 \pm 1$       | 1.36    | -16.81 | 8.39                 |
| 3506   | 00 29 33.17 | -09 04 50.74 | IC 0022                 | $6049 \pm 2$       | 2.53    | -21.22 | 10.66                |
| 3510   | 00 15 00.08 | -11 08 03.79 | ASK 125926              | $3351 \pm 2$       | 1.27    | -16.03 | 8.05                 |
| 3520   | 13 52 53.20 | 37 41 22.28  | 2MASX J13525317+3741219 | $5317 \pm 2$       | 2.55    | -20.18 | 10.24                |
| 3527   | 13 56 55.58 | 05 09 06.83  | CGCG 046-013            | $1517 \pm 10$      | 2.11    | -16.85 | 8.60                 |
| 3542   | 08 19 24.29 | 21 00 12.82  | 2MASX J08192430+2100125 | $3906 \pm 4$       | 2.54    | -18.79 | 9.67                 |
| 3546   | 07 45 01.45 | 43 55 52.36  | 2MASX J07450145+4355525 | $3736 \pm 1$       | 1.30    | -17.01 | 8.43                 |
| 3556   | 08 51 56.67 | 16 56 41.32  | UGC 04639               | $8549 \pm 2$       | 2.70    | -22.44 | 11.18                |
| 3565   | 09 14 13.07 | 43 08 05.97  | KUG 0910+433            | $4232 \pm 2$       | 1.90    | -20.15 | 10.09                |
| 3572   | 03 30 17.18 | 00 55 12.71  | CGCG 390-096            | $6412 \pm 2$       | 2.75    | -21.50 | 10.87                |
| 3581   | 03 37 10.37 | -05 35 05.09 | 2MASX J03371039-0535055 | $8347 \pm 2$       | 2.61    | -21.77 | 10.90                |
| 3622   | 22 51 43.16 | 00 24 54.98  | 2MASX J22514319+0024547 | $7807 \pm 2$       | 2.84    | -21.33 | 10.84                |
| 3650   | 01 29 43.99 | -01 14 29.10 | UGC 01072               | $5190 \pm 2$       | 2.59    | -21.23 | 10.61                |
| 3654   | 03 58 19.35 | -04 43 49.56 | ASK 57478               | $5294 \pm 2$       | 1.60    | -18.21 | 8.93                 |
| 3663   | 07 29 45.06 | 43 44 45.15  | ASK 476339              | $3183 \pm 4$       | 1.65    | -15.76 | 8.10                 |
| 3665   | 07 22 46.74 | 41 39 29.65  | UGC 03818               | $7002 \pm 2$       | 2.44    | -21.19 | 10.67                |
| 3666   | 07 26 35.39 | 43 17 46.85  | UGC 03844               | $3130 \pm 2$       | 2.70    | -20.57 | 10.42                |
| 3668   | 07 24 33.15 | 41 57 02.18  | 2MASX J07243311+4157021 | $7960 \pm 3$       | 2.30    | -19.49 | 9.96                 |
| 3669   | 07 24 19.58 | 38 45 38.73  | 2MASX J07241961+3845387 | $7244 \pm 2$       | 2.46    | -19.19 | 9.80                 |
| 3670   | 07 21 00.79 | 41 03 06.58  | 2MASX J07210079+4103065 | $6903 \pm 2$       | 1.43    | -18.69 | 9.22                 |
| 3673   | 07 27 28.08 | 43 27 50.08  | ASK 476000              | $6623 \pm 1$       | 1.13    | -17.60 | 8.70                 |
| 3691   | 12 28 08.61 | 12 05 35.85  | IC 0794                 | $1921 \pm 3$       | 2.37    | -19.16 | 9.64                 |
| 3698   | 01 26 42.25 | -01 05 16.00 | ASK 32676               | $4370 \pm 8$       | 2.29    | -17.32 | 9.19                 |
| 3706   | 03 11 17.74 | -08 04 48.04 | 2MASX J03111772-0804486 | $3978 \pm 1$       | 1.26    | -17.96 | 8.75                 |
| 3710   | 14 01 57.67 | 46 18 42.90  | NGC 5439                | $1895 \pm 4$       | 2.02    | -18.59 | 9.42                 |
| 3711   | 14 29 14.46 | 44 41 56.37  | CGCG 247-032            | $2409 \pm 2$       | 2.48    | -18.94 | 9.71                 |
| 3716   | 11 52 24.07 | 32 24 13.96  | NGC 3935                | $3066 \pm 2$       | 2.19    | -20.30 | 10.22                |
| 3721   | 07 21 23.42 | 41 41 59.03  | ASK 475472              | $7001 \pm 2$       | 1.05    | -17.45 | 8.48                 |
| 3735   | 00 19 47.33 | 00 35 26.86  | 2MASXJ00194732+0035273  | $5306 \pm 3$       | 1.94    | -19.65 | 9.75                 |
| 3762   | 00 39 55.98 | -08 51 11.54 | ASK 127226              | $4122 \pm 1$       | 1.18    | -16.61 | 8.26                 |
| 3779   | 01 28 59.57 | 00 33 42.93  | UGC 01062               | $5464 \pm 2$       | 2.60    | -21.76 | 10.85                |
| 3783   | 01 13 41.83 | 00 06 09.76  | UGC 00771               | $5152 \pm 2$       | 2.55    | -20.84 | 10.54                |
| 3784   | 01 15 54.29 | 13 21 12.05  | CGCG 436-016            | $4184 \pm 2$       | 2.59    | -20.14 | 10.24                |
| 3795   | 00 25 17.31 | 14 34 40.89  | ASK 147884              | $5224 \pm 1$       | 1.06    | -16.86 | 8.11                 |
| 3801   | 01 03 01.72 | -01 06 39.54 | CGCG 384-061            | $5237 \pm 2$       | 2.51    | -20.12 | 10.21                |
| 3805   | 01 22 46.01 | 00 25 35.09  | 2MASX J01224599-0025343 | $5182 \pm 3$       | 2.22    | -18.95 | 9.61                 |
| 3808   | 01 15 22.22 | 00 09 30.44  | 2MASX J01152220-0009299 | $5196 \pm 4$       | 2.32    | -18.15 | 9.30                 |
| 3813   | 01 04 25.32 | -09 22 59.33 | PGC 991736              | $4653 \pm 1$       | 1.41    | -17.36 | 8.51                 |
| 3832   | 01 38 47.38 | 01 04 18.45  | UGC 01169               | $4964 \pm 2$       | 3.14    | -20.34 | 10.58                |

Table 1: continued from previous page

| Source | RA          | Dec          | Name                    | $V_{\text{opt}}$   | $u - r$ | $M_r$  | $M_{\star}$          |
|--------|-------------|--------------|-------------------------|--------------------|---------|--------|----------------------|
|        | (J2000)     |              |                         | $\text{km s}^{-1}$ | mag     | mag    | [log]<br>$M_{\odot}$ |
| 3841   | 01 48 53.13 | 13 25 26.20  | 2MASXi J0148531+132526  | $4659 \pm 2$       | 2.17    | -18.29 | 9.41                 |
| 3842   | 01 49 53.83 | 12 58 33.74  | 2MASX J01495381+1258340 | $4691 \pm 6$       | 2.48    | -18.14 | 9.35                 |
| 3846   | 01 55 16.26 | -08 51 15.39 | KUG 0152-090            | $3950 \pm 2$       | 1.56    | -17.30 | 8.60                 |
| 3848   | 01 55 59.75 | 00 11 08.04  | PGC 3111971             | $3637 \pm 1$       | 1.16    | -17.01 | 8.19                 |
| 3906   | 02 31 41.35 | -09 18 01.60 | NGC 0960                | $4867 \pm 1$       | 2.81    | -20.85 | 10.71                |
| 3946   | 03 20 40.80 | -07 23 39.89 | NGC 1303                | $5461 \pm 1$       | 2.41    | -21.33 | 10.59                |
| 3947   | 03 17 48.53 | -07 37 00.65 | NGC 1286                | $4312 \pm 1$       | 2.51    | -20.80 | 10.45                |
| 3951   | 03 17 06.67 | -06 30 07.76 | 2MASX J03170667-0630082 | $4008 \pm 4$       | 2.06    | -19.74 | 9.91                 |
| 3956   | 03 15 38.62 | -07 04 43.75 | KUG 0313-072            | $3947 \pm 1$       | 1.58    | -18.83 | 9.24                 |
| 3986   | 03 39 07.13 | -06 27 02.88 | 2MASX J03390711-0627028 | $5381 \pm 4$       | 2.16    | -20.03 | 10.08                |
| 3997   | 03 38 04.15 | -05 21 09.07 | ASK 56542               | $4019 \pm 1$       | 1.48    | -17.25 | 8.56                 |
| 4020   | 04 12 11.55 | -04 52 27.14 | ASK 57882               | $9047 \pm 4$       | 1.39    | -18.88 | 9.19                 |
| 4026   | 04 01 33.54 | -06 20 12.46 | PGC 1034032             | $5722 \pm 1$       | 1.50    | -17.56 | 8.77                 |
| 4030   | 07 27 19.37 | 44 25 38.37  | 2MASX J07271936+4425388 | $9742 \pm 2$       | 2.58    | -20.87 | 10.89                |
| 4031   | 07 26 24.68 | 43 02 54.78  | ASK 475844              | $7583 \pm 2$       | 1.70    | -18.64 | 9.30                 |
| 4032   | 07 26 20.04 | 42 02 46.22  | ASK 475860              | $7994 \pm 4$       | 1.82    | -18.98 | 9.21                 |
| 4033   | 07 20 02.10 | 41 08 11.21  | ASK 475444              | $7026 \pm 4$       | 1.50    | -17.37 | 8.53                 |
| 4060   | 07 41 54.78 | 38 29 53.74  | 2MASX J07415484+3829537 | $3507 \pm 1$       | 1.06    | -17.27 | 8.31                 |
| 4061   | 07 44 05.51 | 46 42 34.21  | ASK 476552              | $3105 \pm 1$       | 1.15    | -16.46 | 8.00                 |
| 4088   | 08 17 35.00 | 20 54 11.06  | NGC 2553                | $4670 \pm 1$       | 2.61    | -21.18 | 10.64                |
| 4093   | 08 18 08.76 | 23 02 51.31  | IC 2269                 | $3980 \pm 2$       | 3.01    | -19.38 | 10.18                |
| 4094   | 08 19 32.11 | 21 23 39.50  | IC 2293                 | $4090 \pm 3$       | 1.89    | -20.00 | 9.98                 |
| 4101   | 08 05 47.84 | 30 13 52.35  | CGCG 148-111            | $2306 \pm 3$       | 1.71    | -17.62 | 9.17                 |
| 4106   | 08 17 15.93 | 24 53 56.81  | 2MASXJ08171594+2453569  | $1898 \pm 7$       | 2.17    | -16.08 | 8.42                 |
| 4109   | 08 23 24.07 | 22 16 00.45  | ASK 484591              | $2055 \pm 13$      | 2.46    | -16.06 | 8.31                 |
| 4110   | 08 26 28.81 | 26 04 29.10  | ASK 364075              | $1968 \pm 17$      | 2.05    | -15.75 | 8.16                 |
| 4129   | 08 37 26.59 | 40 02 08.11  | UGC 04498               | $7091 \pm 2$       | 2.48    | -21.61 | 10.81                |
| 4151   | 08 33 12.72 | 39 30 49.82  | ASK 191177              | $2026 \pm 1$       | 1.27    | -16.29 | 8.00                 |
| 4170   | 09 14 34.33 | 30 08 27.06  | UGC 04869               | $6852 \pm 2$       | 2.81    | -22.16 | 11.17                |
| 4175   | 09 10 11.89 | 50 24 04.75  | NGC 2767                | $4925 \pm 2$       | 2.79    | -20.98 | 10.71                |
| 4177   | 09 01 28.62 | 03 43 14.13  | NGC 2729                | $3819 \pm 1$       | 2.71    | -20.61 | 10.44                |
| 4184   | 09 12 44.37 | 34 55 32.04  | NGC 2780                | $1954 \pm 2$       | 1.91    | -18.84 | 9.58                 |
| 4197   | 09 14 48.80 | 33 01 15.30  | 2MASX J09144880+3301148 | $1819 \pm 2$       | 1.26    | -16.59 | 8.12                 |
| 4214   | 09 39 34.69 | 48 25 18.56  | UGC 05145               | $7378 \pm 3$       | 2.62    | -21.97 | 11.21                |
| 4222   | 09 57 35.59 | 45 13 47.69  | UGC 05345               | $3696 \pm 2$       | 2.53    | -20.18 | 10.30                |
| 4224   | 09 46 48.95 | 09 44 10.08  | CGCG 063-066            | $2997 \pm 2$       | 2.41    | -19.66 | 9.95                 |
| 4225   | 09 38 34.45 | 08 53 16.44  | 2MASX J09383447+0853159 | $3228 \pm 2$       | 2.38    | -19.46 | 9.95                 |
| 4229   | 09 35 05.80 | 09 38 57.22  | 2MASX J09350578+0938566 | $3408 \pm 2$       | 2.32    | -18.81 | 9.61                 |
| 4231   | 09 48 41.60 | 59 15 39.59  | 2MASX J09484156+5915394 | $2231 \pm 2$       | 1.84    | -18.19 | 9.31                 |
| 4271   | 10 20 43.35 | 65 10 19.61  | UGC 05576               | $3288 \pm 2$       | 2.43    | -20.14 | 10.14                |
| 4274   | 10 12 48.57 | 43 08 43.91  | IC 0598                 | $2245 \pm 1$       | 2.26    | -19.76 | 9.92                 |
| 4309   | 10 37 37.91 | 37 27 20.30  | NGC 3304                | $6937 \pm 2$       | 2.71    | -21.97 | 11.11                |
| 4316   | 10 58 37.57 | 09 03 01.62  | UGC 06062               | $2623 \pm 2$       | 2.59    | -19.98 | 10.18                |
| 4319   | 10 35 04.85 | 46 33 41.23  | UGC 05744               | $3356 \pm 3$       | 1.58    | -19.85 | 9.66                 |
| 4374   | 11 24 06.48 | 38 51 23.09  | 2MASX J11240641+3851226 | $1979 \pm 3$       | 2.45    | -17.29 | 9.03                 |
| 4407   | 11 51 28.06 | 35 26 03.72  | UGC 06827               | $3095 \pm 2$       | 2.47    | -20.18 | 10.13                |
| 4414   | 11 51 13.43 | 50 09 24.84  | NGC 3922                | $930 \pm 3$        | 2.21    | -18.20 | 9.25                 |
| 4448   | 12 05 59.46 | 02 29 53.63  | CGCG 041-039            | $6098 \pm 2$       | 2.68    | -21.29 | 10.96                |
| 4458   | 12 12 11.80 | 13 14 47.46  | NGC 4165                | $1868 \pm 4$       | 2.07    | -18.87 | 9.49                 |
| 4459   | 12 11 02.73 | 12 06 14.40  | IC 0767                 | $1877 \pm 2$       | 2.05    | -18.82 | 9.41                 |
| 4462   | 12 08 55.08 | 41 44 27.12  | UGC 07129               | $925 \pm 2$        | 1.85    | -17.43 | 8.97                 |
| 4465   | 12 22 19.53 | 14 45 38.81  | UGC 07436               | $982 \pm 4$        | 2.29    | -17.13 | 8.76                 |
| 4514   | 12 51 41.53 | 13 05 41.88  | CGCG 071-059            | $1487 \pm 5$       | 1.72    | -16.48 | 8.30                 |
| 4516   | 12 41 39.41 | 12 14 50.61  | IC 3663                 | $927 \pm 10$       | 1.99    | -15.90 | 8.11                 |
| 4541   | 13 08 42.15 | 52 01 00.69  | CGCG 271-017            | $4705 \pm 2$       | 2.62    | -20.96 | 10.63                |
| 4542   | 13 14 46.04 | 53 49 13.27  | CGCG 271-026            | $4711 \pm 2$       | 2.61    | -20.77 | 10.53                |

Table 1: continued from previous page

| Source | RA          | Dec          | Name                    | $V_{\text{opt}}$   | $u - r$ | $M_r$  | $M_{\star}$          |
|--------|-------------|--------------|-------------------------|--------------------|---------|--------|----------------------|
|        | (J2000)     |              |                         | $\text{km s}^{-1}$ | mag     | mag    | [log]<br>$M_{\odot}$ |
| 4546   | 13 17 07.56 | 57 32 22.17  | IC 0875                 | $2760 \pm 2$       | 2.40    | -20.10 | 10.01                |
| 4595   | 13 56 58.06 | 45 58 23.61  | UGC 08876               | $2059 \pm 1$       | 2.56    | -19.28 | 9.88                 |
| 4598   | 13 48 56.27 | 59 50 08.64  | UGC 08741               | $2019 \pm 6$       | 2.00    | -18.70 | 9.44                 |
| 4609   | 13 53 19.84 | 05 46 17.93  | UGC 08799               | $1046 \pm 16$      | 2.14    | -15.71 | 8.26                 |
| 4634   | 14 03 47.16 | 35 44 30.04  | UGC 08984               | $3805 \pm 1$       | 2.58    | -20.61 | 10.42                |
| 4640   | 14 07 39.28 | 54 47 40.60  | CGCG 272-032            | $2315 \pm 1$       | 2.33    | -19.11 | 9.68                 |
| 4644   | 14 09 54.94 | 56 49 21.36  | CGCG 295-037            | $1790 \pm 4$       | 2.17    | -17.85 | 9.18                 |
| 4648   | 14 04 42.99 | 55 26 06.72  | 2MASX J14044299+5526064 | $1537 \pm 2$       | 1.86    | -16.96 | 8.63                 |
| 4668   | 14 57 11.25 | 52 20 45.82  | UGC 09629               | $7822 \pm 2$       | 2.78    | -21.82 | 11.05                |
| 4680   | 14 58 48.72 | 02 01 24.62  | CGCG 020-039            | $1804 \pm 1$       | 2.31    | -18.60 | 9.50                 |
| 4687   | 14 48 58.97 | 33 11 34.95  | CGCG 193-002            | $1700 \pm 2$       | 1.45    | -16.89 | 8.33                 |
| 4696   | 14 54 19.38 | 38 48 29.91  | CGCG 221-008            | $8685 \pm 3$       | 2.75    | -21.76 | 11.03                |
| 4698   | 14 31 49.74 | 27 53 30.30  | PGC 4553986             | $4415 \pm 4$       | 1.76    | -16.91 | 8.32                 |
| 4720   | 15 11 48.38 | 46 15 13.90  | CGCG 249-011            | $5454 \pm 2$       | 2.20    | -20.41 | 10.31                |
| 4728   | 15 13 29.18 | 58 30 33.56  | Mrk 0847                | $2543 \pm 3$       | 1.60    | -18.96 | 9.41                 |
| 4732   | 15 00 16.58 | 02 18 02.57  | CGCG 020-042            | $1818 \pm 3$       | 1.98    | -17.72 | 9.09                 |
| 4734   | 15 01 03.11 | 00 42 27.44  | Mrk 1390                | $1724 \pm 3$       | 1.77    | -17.08 | 8.75                 |
| 4736   | 15 12 31.74 | 00 48 45.30  | PGC 1176138             | $1844 \pm 4$       | 1.67    | -16.76 | 8.53                 |
| 4806   | 16 02 16.34 | 49 12 11.42  | UGC 10150               | $6135 \pm 6$       | 2.12    | -20.36 | 10.16                |
| 4808   | 16 02 11.63 | 07 05 09.97  | CGCG 051-021            | $2654 \pm 2$       | 2.24    | -19.45 | 9.98                 |
| 4838   | 16 58 50.69 | 40 07 16.18  | CGCG 225-021            | $8658 \pm 2$       | 2.73    | -22.04 | 11.06                |
| 4846   | 16 41 06.57 | 46 00 14.63  | IC 1226                 | $5312 \pm 4$       | 2.35    | -20.32 | 10.26                |
| 4855   | 16 35 20.71 | 17 45 55.19  | Mrk 0886                | $2740 \pm 1$       | 1.12    | -18.21 | 8.94                 |
| 4861   | 16 34 39.88 | 46 57 37.26  | 2MASXi J1634398+465736  | $2452 \pm 1$       | 1.24    | -16.74 | 8.26                 |
| 4898   | 17 01 12.98 | 60 15 05.25  | Ark 514                 | $3743 \pm 2$       | 1.47    | -18.70 | 9.02                 |
| 4908   | 17 01 29.63 | 22 43 52.46  | ASK 406590              | $2820 \pm 1$       | 2.22    | -15.79 | 8.11                 |
| 4960   | 20 54 12.19 | -05 11 31.60 | 2MASX J20541219-0511314 | $6134 \pm 5$       | 2.44    | -18.59 | 9.63                 |
| 4989   | 21 16 24.75 | 10 16 24.07  | CGCG 426-029            | $5175 \pm 2$       | 2.29    | -20.22 | 10.15                |
| 4990   | 21 04 51.97 | 00 26 52.75  | CGCG 374-042            | $4129 \pm 2$       | 2.45    | -19.62 | 9.95                 |
| 4997   | 21 28 29.09 | 10 04 52.52  | 2MASX J21282910+1004527 | $4929 \pm 2$       | 2.03    | -18.16 | 9.10                 |
| 4999   | 21 13 07.73 | 01 13 47.13  | 2MASX J21130776+0113480 | $4157 \pm 2$       | 1.30    | -18.41 | 8.97                 |
| 5004   | 21 18 06.61 | -07 42 56.84 | 2MASX J21180656-0742566 | $2516 \pm 2$       | 1.41    | -16.62 | 8.17                 |
| 5015   | 21 31 37.56 | 11 49 53.90  | CGCG 426-062            | $8643 \pm 3$       | 2.92    | -21.99 | 11.15                |
| 5020   | 21 50 38.41 | 13 17 17.48  | CGCG 427-027            | $6045 \pm 2$       | 2.59    | -21.61 | 10.88                |
| 5025   | 21 50 27.56 | 12 38 10.37  | 2MASX J21502753+1238103 | $6507 \pm 2$       | 2.48    | -19.53 | 9.98                 |
| 5040   | 21 52 22.47 | -01 10 15.96 | ASK 21400               | $4770 \pm 1$       | 1.15    | -16.83 | 8.14                 |
| 5048   | 22 01 41.64 | 11 51 24.41  | CGCG 428-014            | $8944 \pm 3$       | 3.13    | -21.95 | 11.33                |
| 5061   | 22 24 44.13 | 12 21 40.68  | 2MASX J22244417+1221410 | $5127 \pm 3$       | 2.09    | -19.23 | 9.80                 |
| 5063   | 22 20 19.83 | -08 46 17.13 | 2MASXi J2220198-084617  | $7288 \pm 1$       | 1.11    | -18.81 | 8.97                 |
| 5070   | 22 04 08.80 | 00 55 31.78  | ASK 22153               | $4825 \pm 16$      | 2.28    | -17.21 | 8.66                 |
| 5096   | 22 40 17.46 | 14 29 56.90  | 2MASX J22401742+1429556 | $6384 \pm 1$       | 1.20    | -18.96 | 9.20                 |
| 5105   | 22 33 49.80 | 00 28 58.47  | ASK 23755               | $4642 \pm 1$       | 1.09    | -17.02 | 8.22                 |
| 5117   | 23 18 08.39 | 00 23 25.63  | CGCG 380-023            | $8775 \pm 2$       | 2.71    | -22.40 | 11.17                |
| 5118   | 23 20 29.08 | -01 00 08.81 | CGCG 380-035            | $9370 \pm 2$       | 2.75    | -22.03 | 11.08                |
| 5120   | 23 23 27.04 | 14 19 33.09  | CGCG 431-053            | $7651 \pm 2$       | 2.78    | -21.40 | 10.86                |
| 5133   | 23 04 04.16 | 00 46 50.41  | 2MASX J23040415+0046511 | $4903 \pm 3$       | 1.80    | -18.56 | 9.27                 |
| 5164   | 23 33 27.02 | 14 20 06.86  | CGCG 432-002            | $5735 \pm 3$       | 2.16    | -20.74 | 10.37                |
| 5165   | 23 43 55.95 | 00 13 05.01  | CGCG 381-031            | $6627 \pm 1$       | 2.48    | -20.28 | 10.25                |
| 5168   | 23 36 34.41 | -09 31 32.06 | PGC 989944              | $6845 \pm 4$       | 1.86    | -19.87 | 9.77                 |
| 5170   | 23 56 11.28 | 00 01 45.24  | 2MASX J23561127-0001452 | $6739 \pm 4$       | 2.52    | -19.07 | 9.76                 |
| 5177   | 23 38 26.05 | 15 23 11.07  | ASK 145449              | $3984 \pm 3$       | 1.80    | -17.25 | 8.78                 |
| 5195   | 13 28 33.04 | 32 04 09.73  | NGC 5166B               | $4838 \pm 3$       | 2.40    | -19.96 | 10.09                |
| 5210   | 23 47 03.79 | 14 50 30.38  | CGCG 432-030            | $6622 \pm 2$       | 2.19    | -20.79 | 10.39                |
| 5215   | 23 40 42.68 | -09 23 36.54 | 2MASXi J2340427-092336  | $5160 \pm 2$       | 1.25    | -18.71 | 9.01                 |
| 5216   | 23 51 14.64 | 15 22 23.88  | ASK 146293              | $5994 \pm 1$       | 1.31    | -17.45 | 8.55                 |
| 5217   | 23 52 42.63 | -11 00 53.07 | ASK 124704              | $5374 \pm 1$       | 1.31    | -17.20 | 8.38                 |

Table 1: continued from previous page

| Source | RA          | Dec          | Name                    | $V_{\text{opt}}$   | $u - r$ | $M_r$  | $M_{\star}$             |
|--------|-------------|--------------|-------------------------|--------------------|---------|--------|-------------------------|
|        | (J2000)     |              |                         | km s <sup>-1</sup> | mag     | mag    | [log]<br>M <sub>⊙</sub> |
| 5226   | 11 58 56.19 | 31 25 10.84  | ASK 527351              | 3021 ± 4           | 1.45    | -17.20 | 8.55                    |
| 5241   | 12 10 32.83 | 58 18 14.90  | NGC 4149                | 3057 ± 3           | 2.35    | -20.07 | 10.37                   |
| 5252   | 00 00 47.89 | 14 16 39.17  | 2MASX J00004789+1416390 | 10847 ± 3          | 2.45    | -20.82 | 10.71                   |
| 5256   | 00 21 35.29 | 01 09 56.33  | CGCG 383-002            | 5465 ± 1           | 2.45    | -20.01 | 10.15                   |
| 5258   | 00 15 05.37 | 15 03 59.70  | 2MASX J00150533+1503597 | 5428 ± 2           | 2.13    | -19.86 | 10.00                   |
| 5260   | 00 10 25.49 | 14 17 23.06  | KUG 0007+140            | 5452 ± 4           | 1.71    | -19.34 | 9.50                    |
| 5268   | 00 22 20.33 | 15 56 30.30  | ASK 148040              | 5213 ± 2           | 1.34    | -17.74 | 8.68                    |
| 5279   | 00 31 36.55 | -10 53 17.43 | 2MASXJ00313653-1053178  | 5075 ± 2           | 2.56    | -20.52 | 10.37                   |
| 5286   | 00 40 26.90 | 00 02 43.53  | 2MASX J00402686-0002431 | 5847 ± 2           | 1.68    | -19.11 | 9.46                    |
| 5292   | 00 53 19.64 | -10 24 11.85 | 2MASX J00531961-1024115 | 4403 ± 1           | 1.04    | -18.33 | 8.80                    |
| 5296   | 00 37 59.82 | 00 42 35.95  | ASK 29753               | 4167 ± 1           | 1.44    | -16.69 | 8.39                    |
| 5305   | 01 12 57.42 | 00 20 41.94  | NGC 0429                | 5628 ± 2           | 2.66    | -21.28 | 10.76                   |
| 5309   | 01 18 44.86 | 00 54 22.80  | CGCG 385-063            | 5251 ± 3           | 2.52    | -20.08 | 10.09                   |
| 5310   | 01 26 25.91 | -08 33 51.12 | 2MASXJ01262589-0833510  | 5336 ± 1           | 2.35    | -20.50 | 10.18                   |
| 5321   | 01 26 49.69 | 00 58 31.08  | Mrk 0570                | 4853 ± 3           | 1.68    | -19.27 | 8.91                    |
| 5323   | 01 13 02.84 | 00 40 40.62  | ASK 31963               | 4500 ± 2           | 1.20    | -16.71 | 8.59                    |
| 5326   | 01 09 42.67 | 00 57 13.29  | ASK 31197               | 5203 ± 3           | 1.48    | -16.83 | 8.24                    |
| 5334   | 01 40 53.63 | -10 16 41.56 | 2MASXJ01405362-1016415  | 5296 ± 1           | 2.57    | -20.75 | 10.50                   |
| 5335   | 01 31 04.76 | 13 38 58.79  | CGCG 436-067            | 5889 ± 2           | 2.76    | -20.40 | 10.49                   |
| 5337   | 01 51 57.52 | -08 31 03.44 | IC 0170                 | 5192 ± 2           | 2.49    | -20.45 | 10.31                   |
| 5340   | 01 42 30.89 | 00 49 10.03  | CGCG 386-032            | 5189 ± 2           | 1.58    | -19.35 | 9.43                    |
| 5344   | 01 34 37.53 | -01 03 08.03 | ASK 33113               | 4787 ± 7           | 1.89    | -17.99 | 9.25                    |
| 5353   | 01 54 41.85 | 00 36 41.71  | PGC 1170628             | 4618 ± 5           | 1.50    | -16.79 | 8.24                    |
| 5369   | 02 20 42.04 | -08 08 26.66 | 2MASX J02204200-0808252 | 4710 ± 3           | 1.77    | -18.94 | 9.44                    |
| 5437   | 03 02 35.01 | -07 21 45.38 | ASK 55199               | 5986 ± 3           | 1.21    | -16.96 | 8.29                    |
| 5440   | 03 02 11.39 | -01 09 59.60 | ASK 37576               | 4079 ± 2           | 1.40    | -16.36 | 8.13                    |
| 5463   | 03 35 34.54 | -05 44 30.75 | ASK 56318               | 5398 ± 1           | 1.18    | -17.48 | 8.44                    |
| 5473   | 04 06 44.26 | -04 26 50.54 | 2MASX J04064426-0426510 | 11300 ± 2          | 1.40    | -19.98 | 9.69                    |
| 5481   | 07 19 51.50 | 41 24 58.04  | 2MASX J07195149+4124585 | 10470 ± 6          | 2.31    | -19.70 | 10.05                   |
| 5483   | 07 25 04.45 | 40 35 37.61  | ASK 475402              | 10200 ± 1          | 0.96    | -18.91 | 8.84                    |
| 5507   | 07 35 24.17 | 36 38 36.47  | ASK 44962               | 3902 ± 1           | 1.08    | -17.11 | 8.23                    |
| 5508   | 07 46 19.80 | 39 51 26.07  | ASK 45258               | 3895 ± 2           | 1.56    | -17.09 | 8.57                    |
| 5522   | 08 03 28.94 | 33 27 44.59  | KUG 0800+336            | 11794 ± 2          | 1.74    | -22.64 | 11.17                   |
| 5525   | 08 20 09.90 | 27 05 36.51  | UGC 04341               | 5869 ± 2           | 2.64    | -21.54 | 10.92                   |
| 5526   | 08 26 18.06 | 27 50 24.47  | IC 2365                 | 6019 ± 1           | 2.55    | -21.66 | 10.77                   |
| 5528   | 08 19 51.89 | 20 59 05.90  | NGC 2560                | 4883 ± 2           | 2.65    | -21.37 | 10.78                   |
| 5536   | 08 16 57.57 | 20 30 44.19  | CGCG 119-027            | 4334 ± 4           | 1.81    | -19.39 | 9.62                    |
| 5547   | 08 22 15.81 | 46 41 30.00  | 2MASX J08221577+4641309 | 2179 ± 1           | 1.41    | -16.36 | 8.26                    |
| 5575   | 08 58 30.48 | 02 55 31.74  | IC 2426                 | 3887 ± 1           | 2.34    | -19.75 | 9.96                    |
| 5586   | 08 34 20.18 | 50 27 08.94  | 2MASX J08342016+5027088 | 3433 ± 2           | 1.61    | -17.13 | 8.63                    |
| 5618   | 09 00 58.50 | 47 47 43.36  | KUG 0857+479            | 3127 ± 2           | 2.41    | -19.29 | 9.99                    |
| 5656   | 09 46 45.58 | 09 15 51.71  | CGCG 063-065            | 4030 ± 2           | 2.53    | -19.34 | 9.85                    |
| 5667   | 09 52 35.11 | 08 11 56.62  | ASK 277328              | 2725 ± 3           | 1.35    | -17.32 | 8.53                    |
| 5668   | 09 46 28.57 | 00 26 03.56  | ASK 51                  | 1810 ± 1           | 1.45    | -16.92 | 8.34                    |
| 5689   | 10 21 21.12 | 24 20 29.04  | UGC 05591               | 11118 ± 2          | 2.71    | -22.33 | 11.21                   |
| 5690   | 10 22 06.03 | 21 03 54.37  | CGCG 124-015            | 11738 ± 3          | 2.77    | -22.63 | 11.33                   |
| 5694   | 10 01 31.06 | 37 12 14.20  | IC 2530                 | 6559 ± 2           | 2.64    | -21.55 | 10.76                   |
| 5696   | 10 25 47.70 | 26 34 14.63  | CGCG 154-013            | 5023 ± 2           | 2.56    | -21.12 | 10.62                   |
| 5699   | 10 00 45.21 | 04 44 03.56  | UGC 05383               | 3968 ± 2           | 2.64    | -20.20 | 10.33                   |
| 5701   | 10 04 31.75 | 60 06 28.71  | NGC 3102                | 3038 ± 2           | 2.44    | -20.01 | 10.15                   |
| 5703   | 10 02 00.95 | 59 15 08.32  | CGCG 289-027            | 2802 ± 4           | 2.09    | -19.12 | 9.60                    |
| 5715   | 10 12 52.79 | 22 43 19.22  | CGCG 123-024            | 1281 ± 3           | 1.51    | -16.49 | 8.16                    |
| 5735   | 10 47 26.58 | 06 02 53.24  | NGC 3376                | 5816 ± 2           | 2.72    | -21.42 | 10.76                   |
| 5743   | 10 35 09.41 | 25 02 17.11  | CGCG 124-039            | 5244 ± 2           | 2.29    | -20.00 | 10.02                   |
| 5816   | 11 38 36.24 | 33 52 04.62  | CGCG 186-015            | 10844 ± 3          | 2.87    | -22.59 | 11.37                   |
| 5821   | 11 57 42.90 | 57 33 57.00  | UGC 06939               | 4915 ± 2           | 2.56    | -21.20 | 10.63                   |

Table 1: continued from previous page

| Source | RA          | Dec         | Name                    | $V_{\text{opt}}$   | $u - r$ | $M_r$  | $M_{\star}$          |
|--------|-------------|-------------|-------------------------|--------------------|---------|--------|----------------------|
|        | (J2000)     |             |                         | $\text{km s}^{-1}$ | mag     | mag    | [log]<br>$M_{\odot}$ |
| 5822   | 11 39 03.33 | 00 12 21.67 | IC 0716                 | $5413 \pm 2$       | 2.59    | -20.79 | 10.68                |
| 5825   | 11 34 11.68 | 12 30 44.33 | NGC 3731                | $3195 \pm 2$       | 2.62    | -20.35 | 10.31                |
| 5828   | 11 59 49.61 | 30 50 39.92 | IC 2986                 | $3108 \pm 2$       | 2.46    | -19.65 | 10.00                |
| 5839   | 11 56 56.36 | 60 19 45.89 | CGCG 292-051            | $1391 \pm 2$       | 1.33    | -16.76 | 8.40                 |
| 5841   | 11 44 24.49 | 60 53 02.67 | 2MASX J11442453+6053022 | $1497 \pm 1$       | 1.45    | -16.42 | 8.41                 |
| 5843   | 11 56 07.08 | 64 21 02.64 | 2MASXi J1156072+642102  | $1410 \pm 1$       | 1.77    | -16.34 | 8.14                 |
| 5883   | 12 09 22.26 | 13 59 32.74 | IC 3019                 | $1675 \pm 14$      | 2.17    | -18.16 | 9.07                 |
| 5884   | 12 20 24.30 | 05 34 22.14 | NGC 4282                | $937 \pm 3$        | 2.50    | -17.14 | 9.11                 |
| 5885   | 12 15 12.56 | 14 25 58.37 | IC 3065                 | $995 \pm 3$        | 2.09    | -17.39 | 8.94                 |
| 5888   | 12 21 04.81 | 11 45 16.56 | IC 3192                 | $1446 \pm 11$      | 2.03    | -16.33 | 8.41                 |
| 5889   | 12 07 12.13 | 63 53 26.64 | MCG +11-15-024          | $1425 \pm 3$       | 1.81    | -16.43 | 8.39                 |
| 5913   | 12 51 16.52 | 53 41 46.66 | IC 0830                 | $4847 \pm 2$       | 2.56    | -21.30 | 10.67                |
| 5921   | 12 35 20.23 | 06 06 54.33 | NGC 4543                | $2374 \pm 1$       | 2.41    | -19.48 | 9.87                 |
| 5923   | 12 30 10.32 | 10 46 46.12 | NGC 4482                | $1835 \pm 3$       | 2.10    | -19.42 | 9.57                 |
| 5926   | 12 36 54.85 | 12 31 12.27 | IC 3586                 | $1723 \pm 4$       | 2.00    | -18.55 | 9.17                 |
| 5931   | 12 40 13.38 | 12 52 29.19 | IC 3635                 | $1560 \pm 8$       | 2.26    | -16.87 | 8.69                 |
| 5936   | 12 39 37.71 | 10 58 32.68 | VCC 1803                | $1355 \pm 21$      | 2.48    | -15.88 | 8.24                 |
| 5999   | 13 48 34.66 | 37 06 47.91 | CGCG 190-059            | $10255 \pm 2$      | 2.54    | -22.49 | 11.11                |
| 6016   | 13 50 41.47 | 40 16 45.63 | CGCG 218-060            | $2300 \pm 2$       | 2.57    | -18.66 | 9.62                 |
| 6025   | 13 58 42.89 | 61 51 45.53 | MCG +10-20-057          | $1795 \pm 2$       | 1.51    | -16.24 | 8.16                 |
| 6060   | 14 01 24.02 | 36 48 00.32 | Mrk 0465                | $2693 \pm 2$       | 1.75    | -18.99 | 9.39                 |
| 6070   | 14 00 58.24 | 55 34 05.19 | ASK 301537              | $1842 \pm 10$      | 1.68    | -16.23 | 8.22                 |
| 6086   | 14 54 32.75 | 02 57 59.13 | NGC 5776                | $8165 \pm 3$       | 2.74    | -22.65 | 11.22                |
| 6107   | 14 45 15.84 | 00 09 34.17 | ASK 8160                | $1664 \pm 4$       | 1.60    | -16.87 | 8.40                 |
| 6111   | 14 42 16.49 | 60 52 22.36 | 2MASX J14421771+6052290 | $2292 \pm 2$       | 1.15    | -16.87 | 8.33                 |
| 6128   | 15 23 35.25 | 09 20 46.14 | CGCG 077-110            | $10703 \pm 2$      | 2.69    | -22.45 | 11.22                |
| 6157   | 15 12 24.05 | 02 04 48.23 | ASK 84838               | $1682 \pm 10$      | 2.00    | -16.04 | 8.32                 |
| 6392   | 21 15 16.19 | 09 53 47.21 | ASK 138334              | $5239 \pm 1$       | 0.97    | -17.38 | 8.38                 |
| 6422   | 21 45 22.59 | 12 16 06.34 | ASK 139520              | $5777 \pm 4$       | 1.35    | -17.12 | 8.21                 |
| 6483   | 23 24 23.54 | 15 26 36.37 | 2MASX J23242356+1526362 | $7658 \pm 2$       | 2.59    | -20.49 | 10.41                |
| 6494   | 23 19 09.42 | 15 43 37.30 | LSBC F677-02            | $4429 \pm 1$       | 1.31    | -18.26 | 8.82                 |
| 6498   | 23 16 03.79 | 13 47 05.74 | ASK 143916              | $4504 \pm 6$       | 1.63    | -16.81 | 8.38                 |
| 6508   | 23 41 25.92 | 00 39 43.89 | 2MASX J23412592-0039437 | $10864 \pm 2$      | 2.77    | -20.93 | 10.68                |
| 6510   | 23 53 31.01 | 00 44 24.61 | CGCG 381-058            | $6925 \pm 3$       | 2.72    | -20.51 | 10.57                |
| 6512   | 23 48 45.08 | 15 55 43.45 | KUG 2346+156            | $7848 \pm 10$      | 1.73    | -20.20 | 9.93                 |
| 6513   | 23 40 32.70 | 00 33 03.84 | 2MASXJ23403276-0033029  | $6928 \pm 3$       | 1.52    | -20.07 | 9.57                 |
| 6546   | 07 40 42.64 | 23 37 34.47 | CGCG 117-065            | $7343 \pm 2$       | 2.76    | -21.17 | 10.76                |
| 6555   | 07 36 44.69 | 42 26 37.39 | 2MASX J07364472+4226376 | $6971 \pm 2$       | 2.51    | -20.21 | 10.31                |
| 6562   | 07 33 27.72 | 41 53 08.78 | 2MASX J07332776+4153084 | $5888 \pm 2$       | 2.30    | -19.35 | 9.82                 |
| 6572   | 07 37 59.17 | 33 56 27.05 | ASK 85066               | $7108 \pm 2$       | 1.62    | -17.83 | 8.87                 |
| 6573   | 07 36 59.47 | 30 29 53.49 | PGC 1906163             | $4546 \pm 2$       | 1.35    | -17.25 | 8.54                 |
| 6607   | 11 23 01.61 | 38 31 11.97 | 2MASXJ11230157+3831120  | $1858 \pm 3$       | 2.07    | -17.05 | 8.70                 |
| 6735   | 08 33 55.25 | 47 08 03.99 | CGCG 237-006            | $4474 \pm 2$       | 2.25    | -19.67 | 9.95                 |
| 6741   | 08 39 00.68 | 40 20 45.98 | UGC 04513               | $7410 \pm 2$       | 2.74    | -21.74 | 10.88                |
| 6747   | 08 46 45.23 | 06 57 35.86 | UGC 04594               | $8732 \pm 3$       | 2.60    | -21.91 | 11.01                |
| 6748   | 08 47 49.73 | 18 54 42.83 | IC 2399                 | $4225 \pm 7$       | 1.98    | -18.87 | 9.44                 |
| 6759   | 13 57 29.53 | 09 57 03.24 | CGCG 074-017            | $6969 \pm 2$       | 2.39    | -20.53 | 10.29                |

## Optical images and H I spectra of non-detected sample

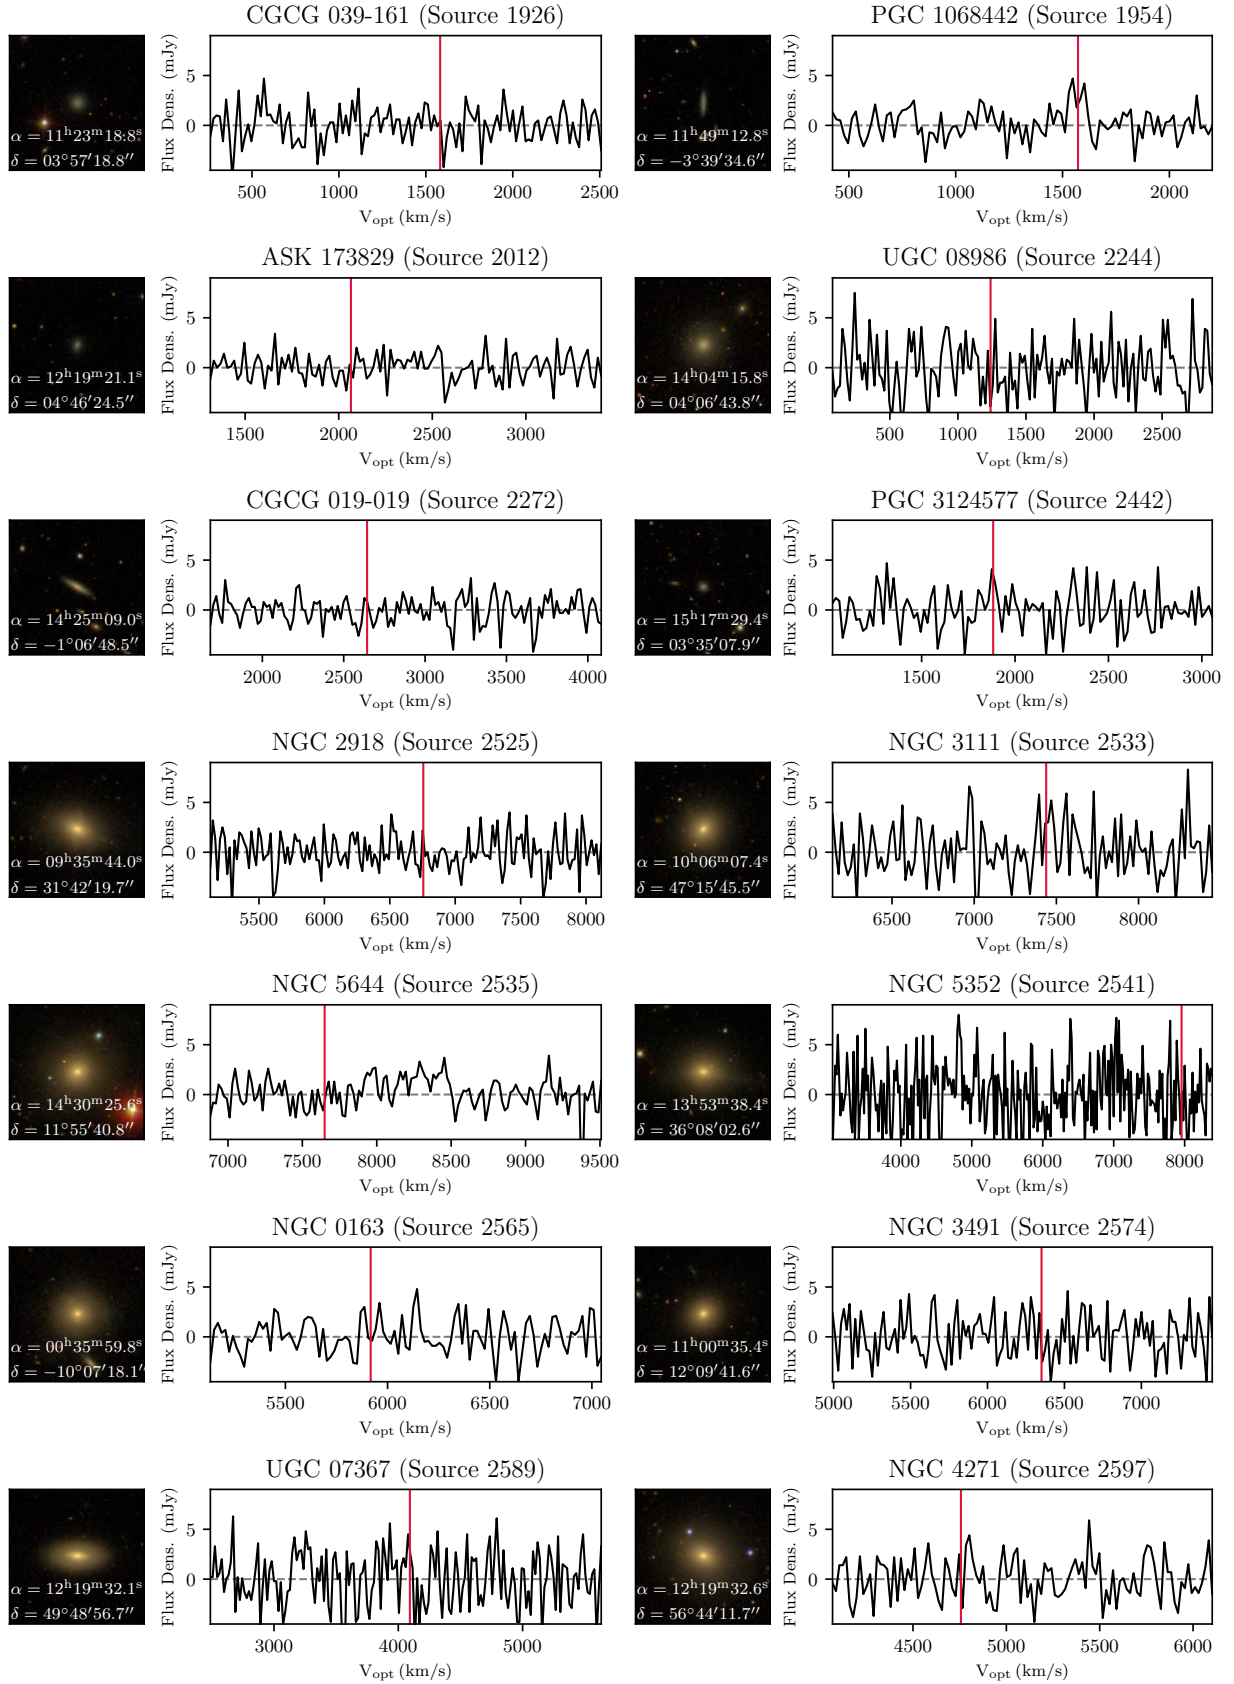

Figure 1: Optical images and H I spectra for all 323 galaxies classified as H I non-detections from the final NIBLES stacking sample. The SDSS redshift of each galaxy is represented by the red line in each spectrum.

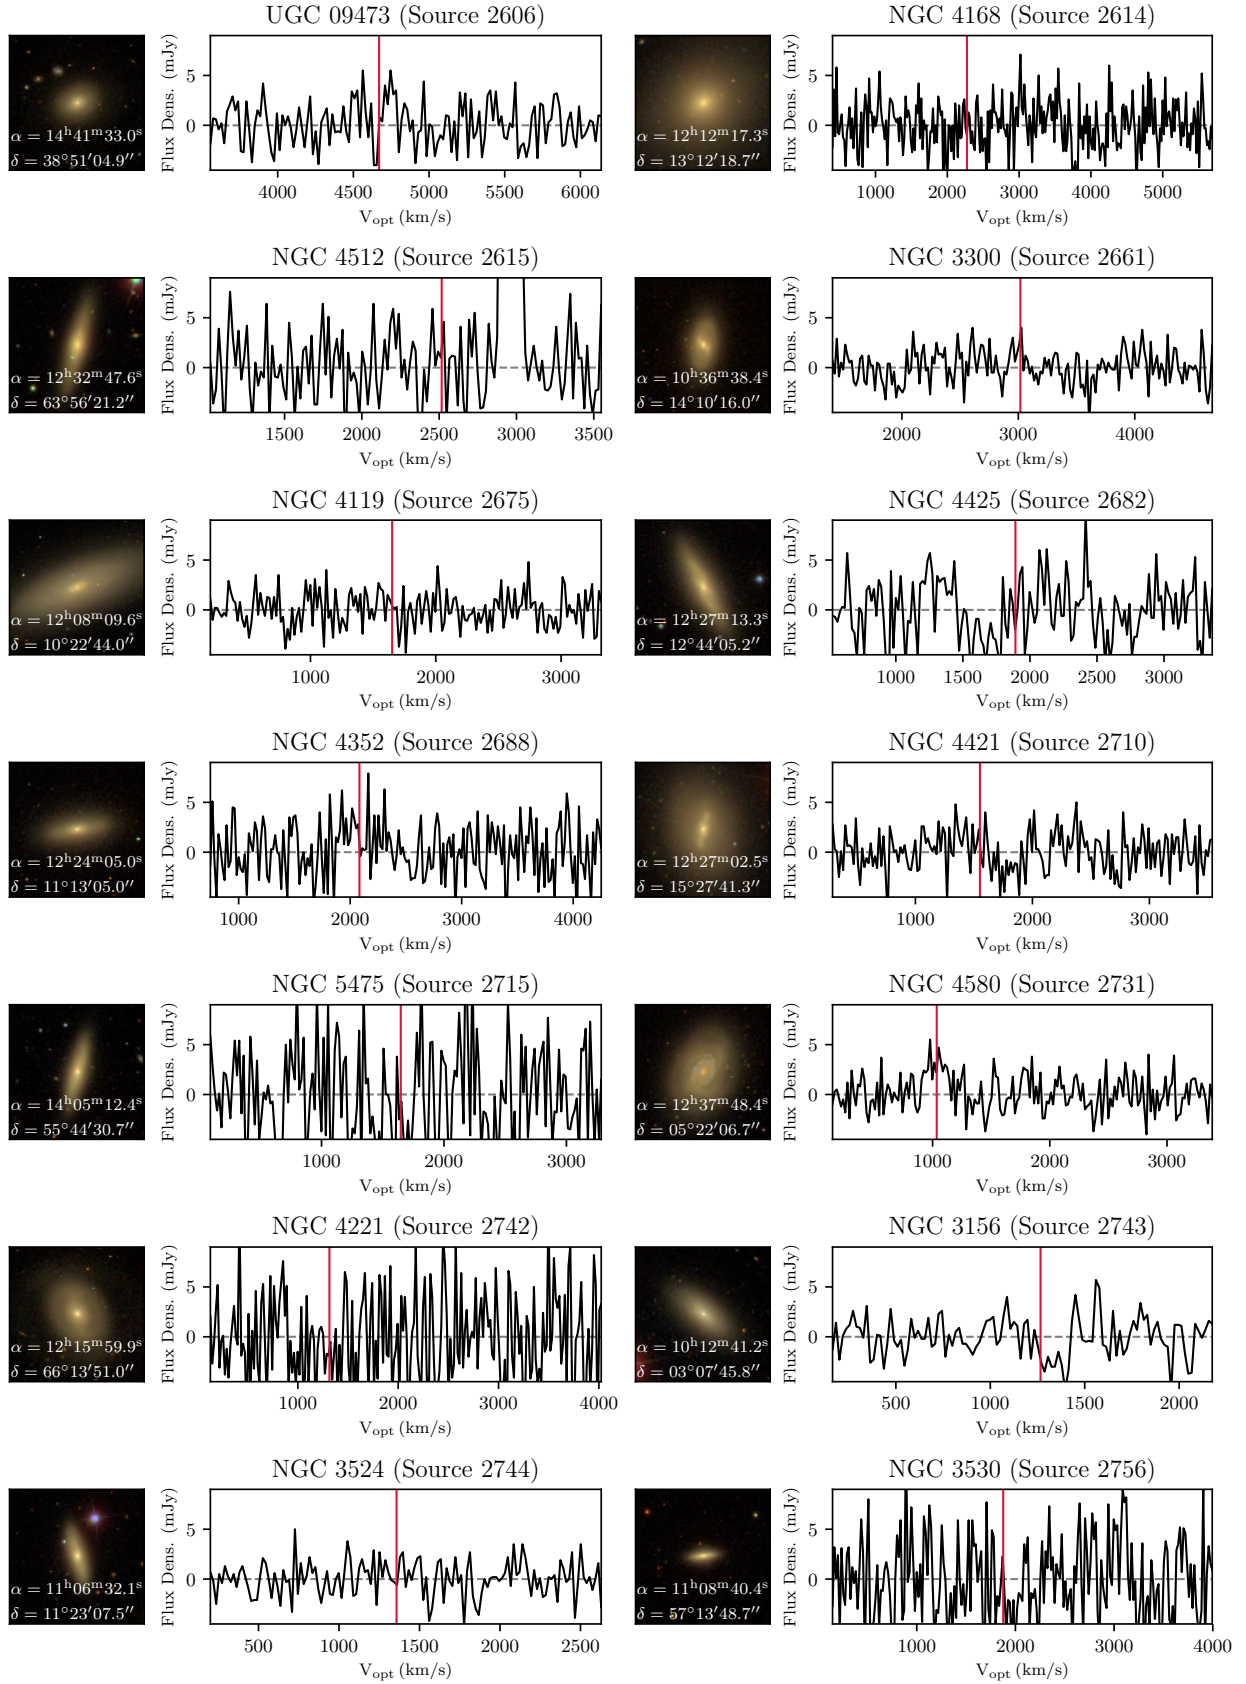

**Figure 1:** (continued) H I non-detected sample.



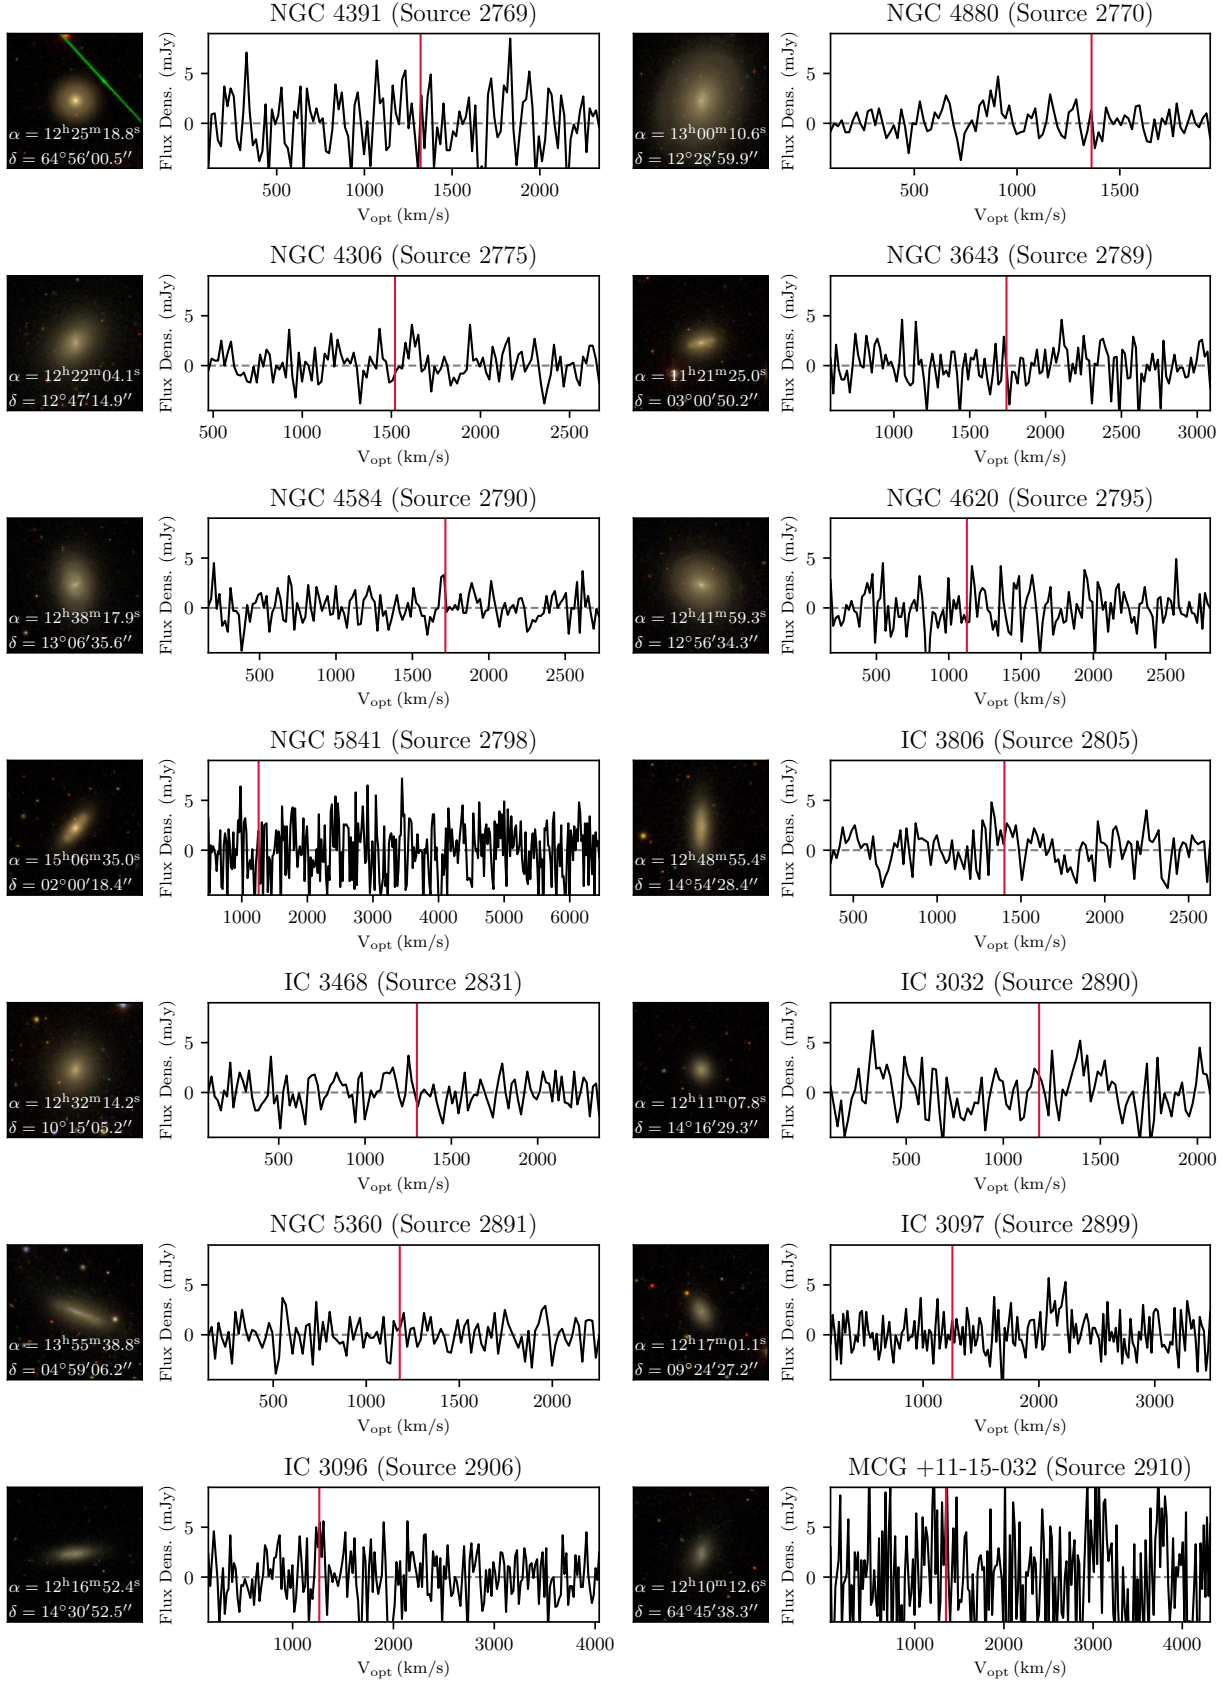

**Figure 1:** (continued) H I non-detected sample.

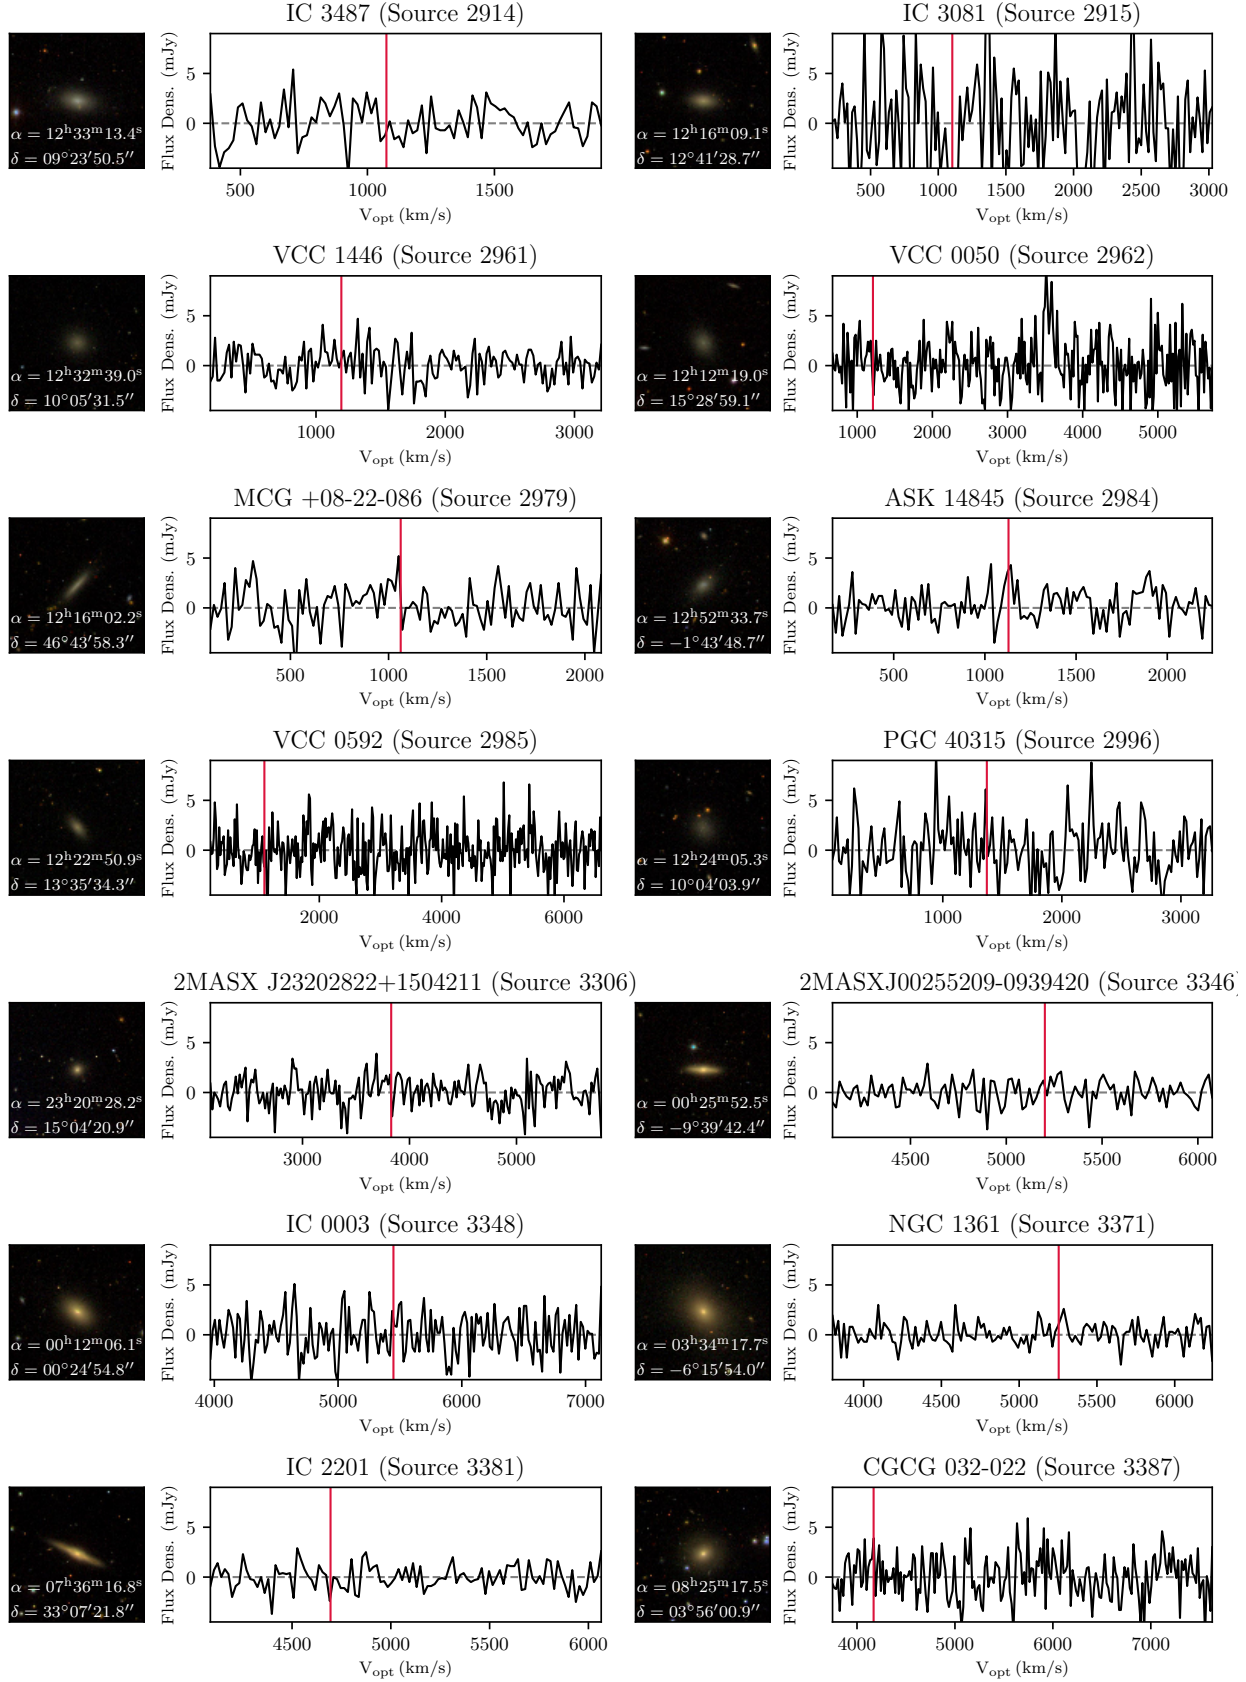

**Figure 1:** (continued) H I non-detected sample.

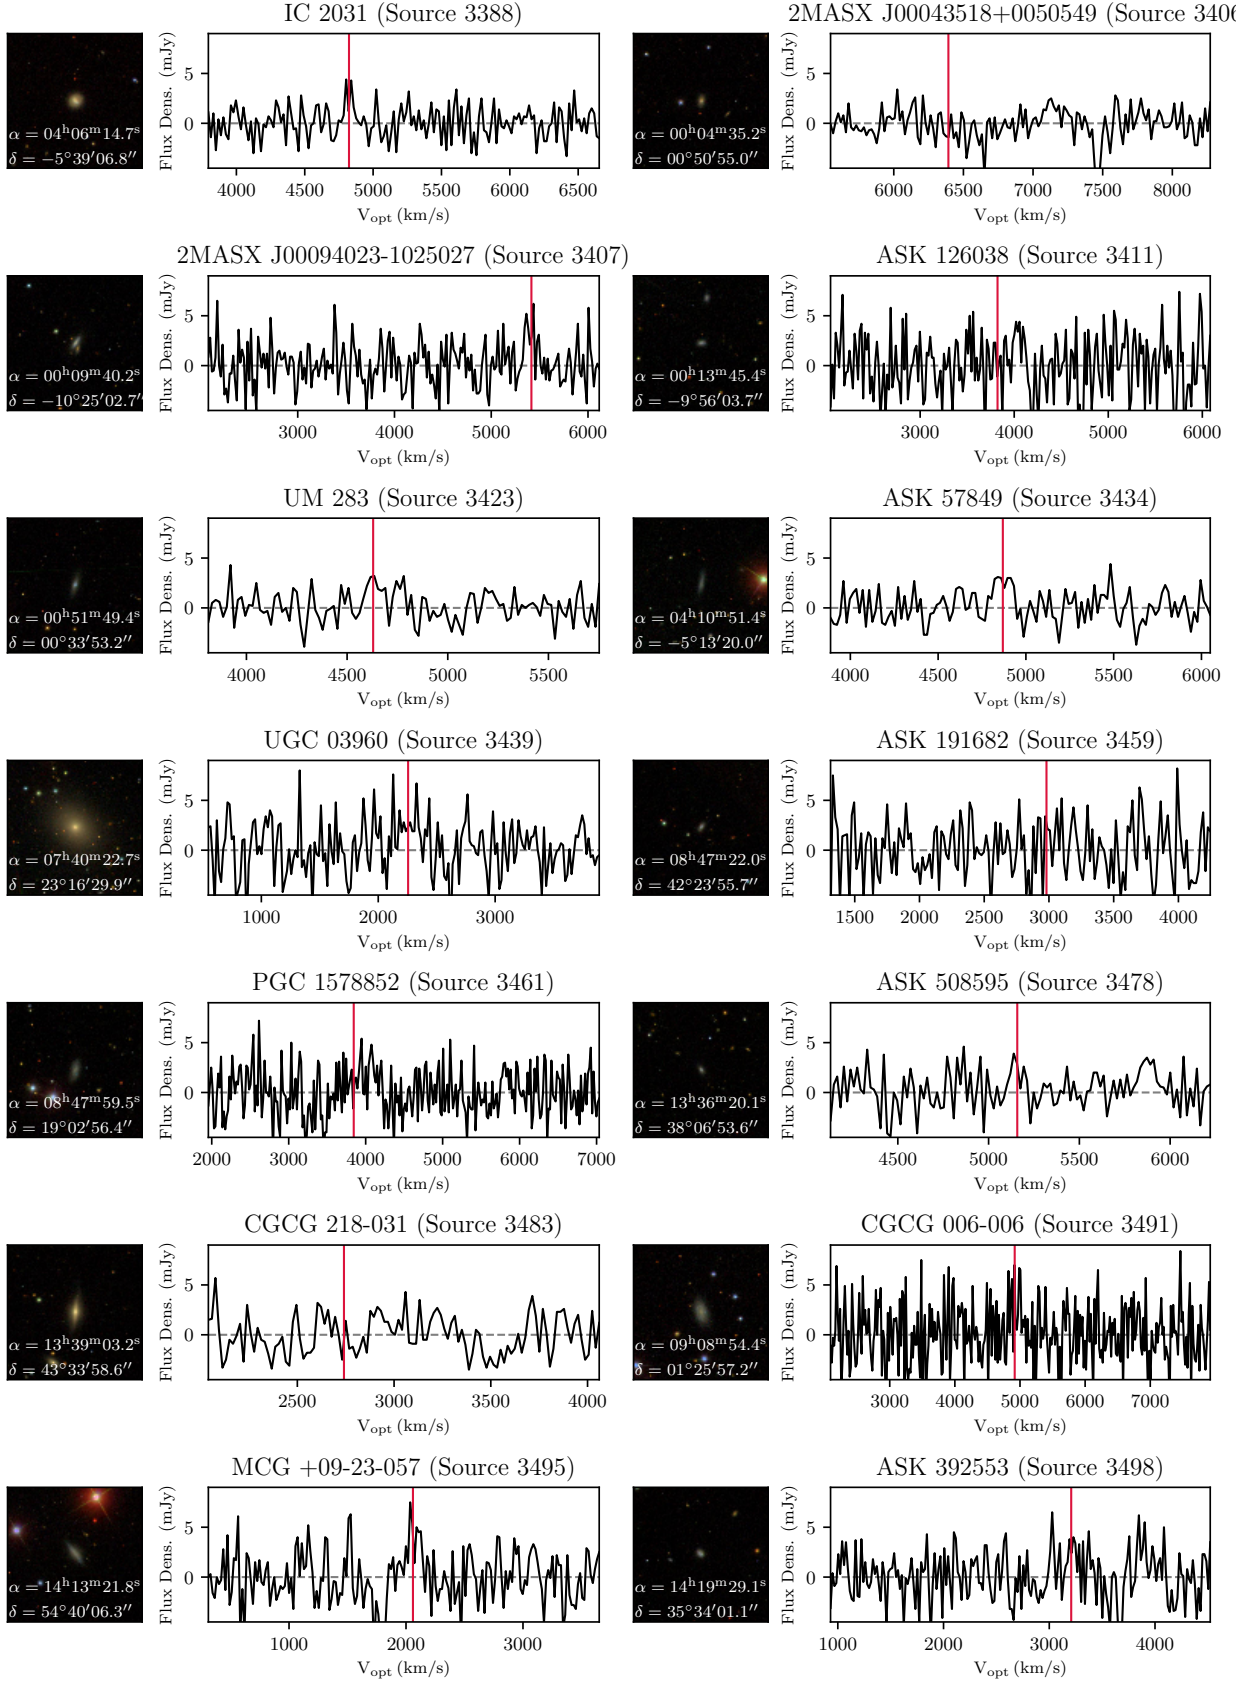

**Figure 1:** (continued) H I non-detected sample.

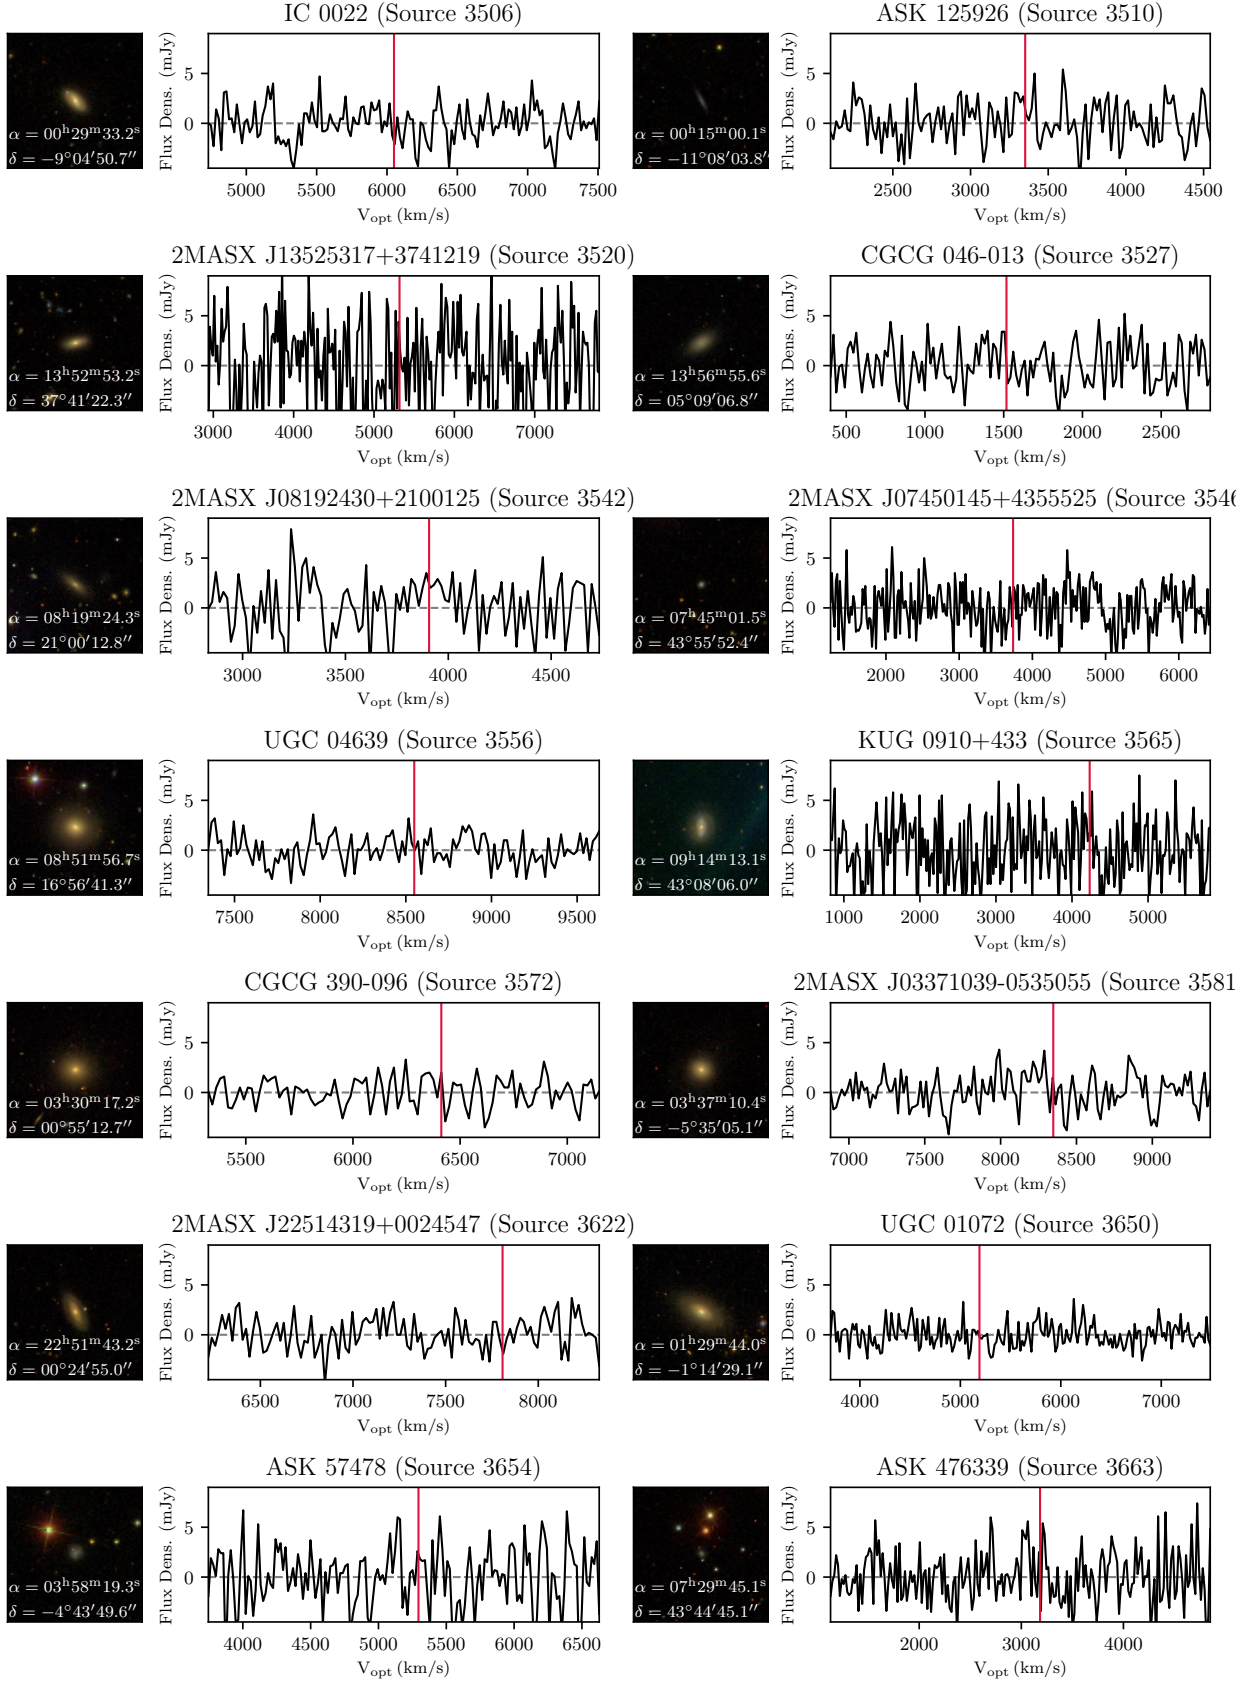

**Figure 1:** (continued) H I non-detected sample.



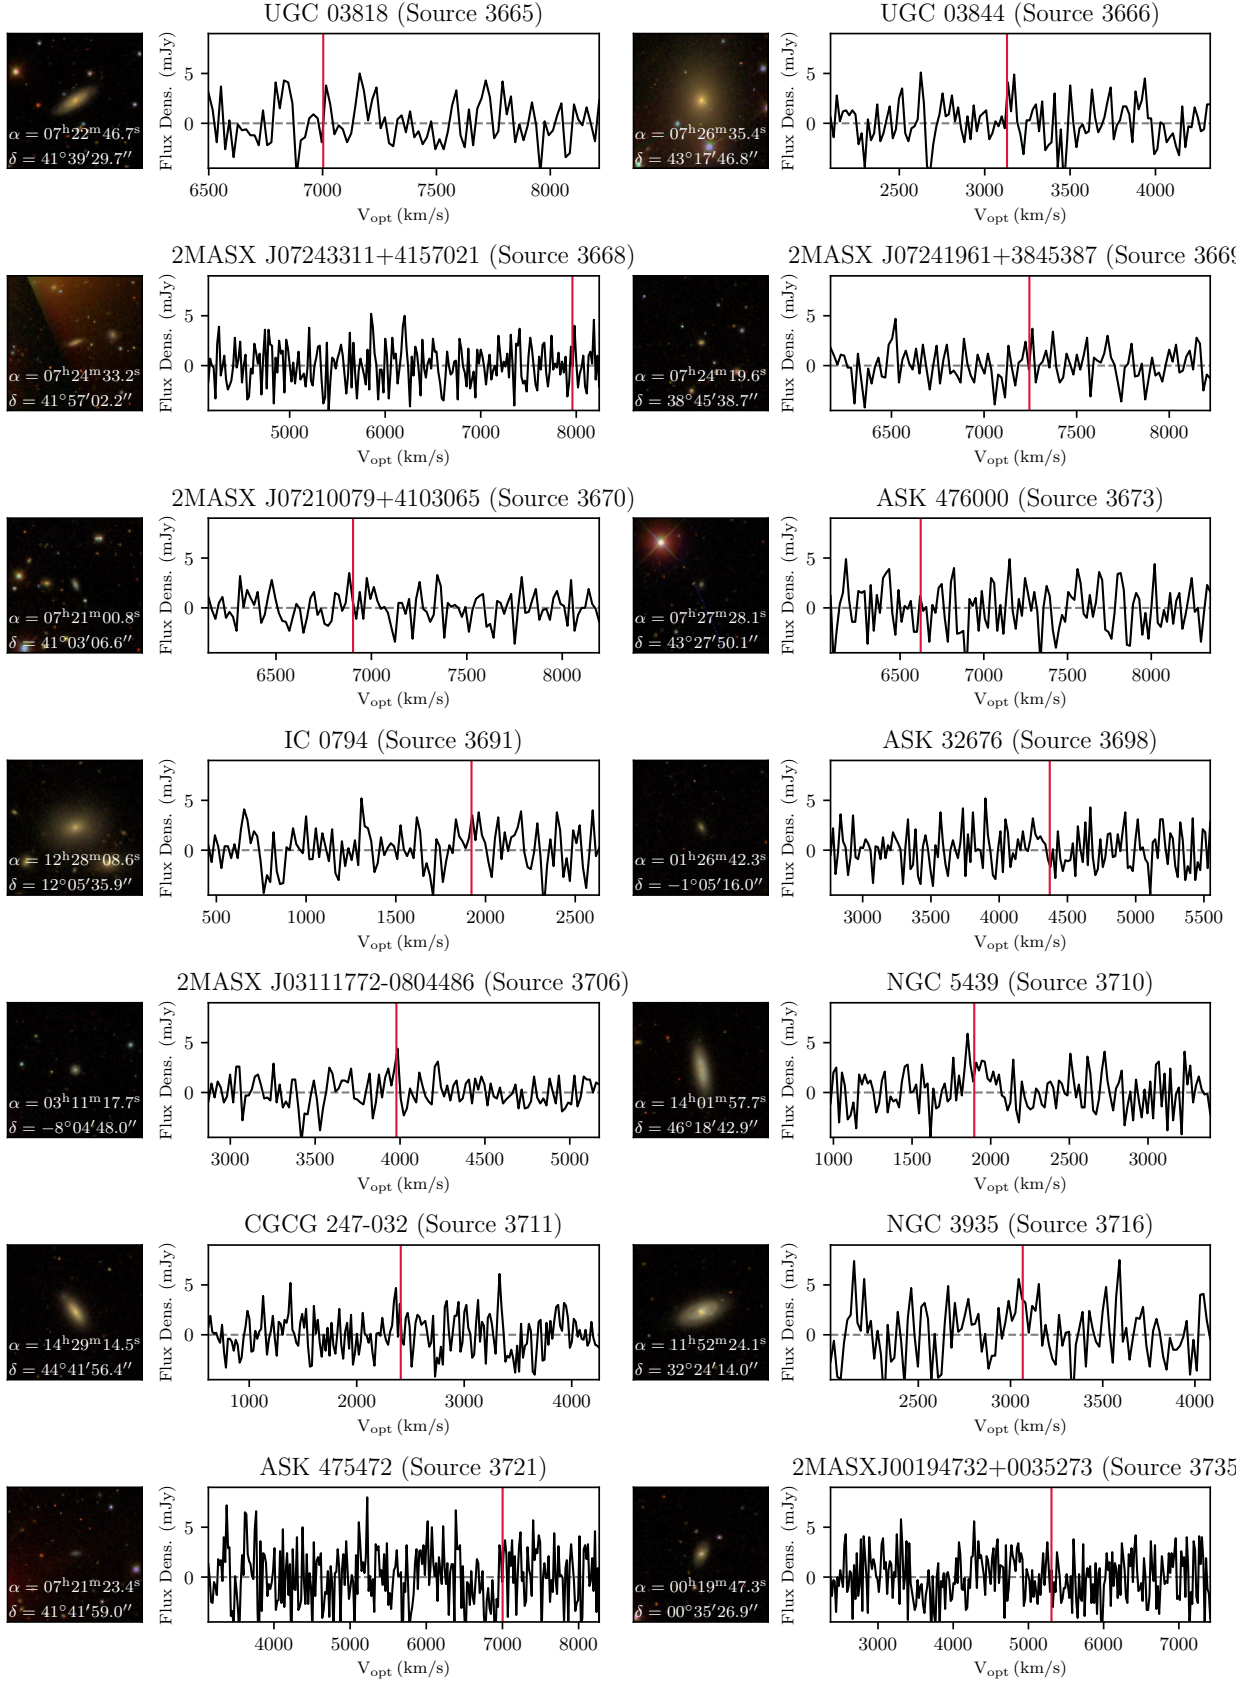

**Figure 1:** (continued) H I non-detected sample.

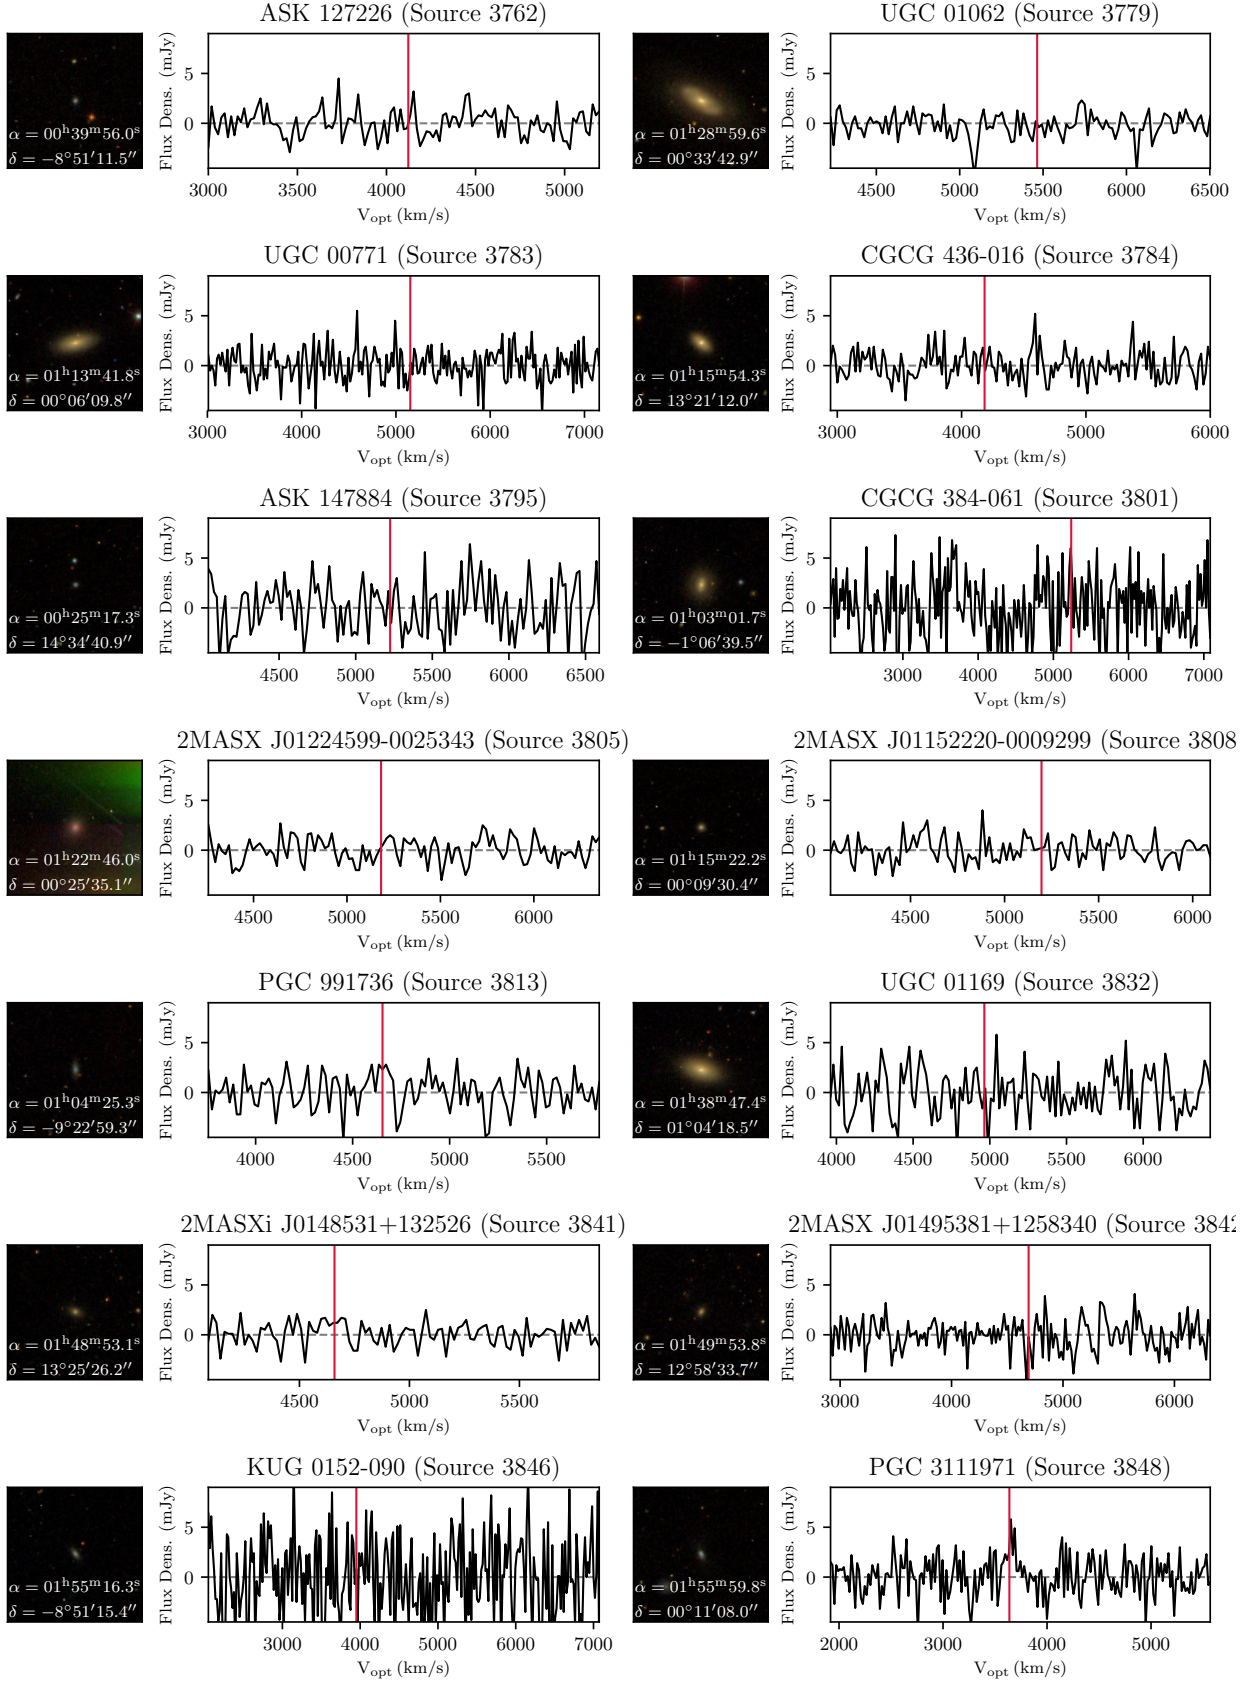

**Figure 1:** (continued) H I non-detected sample.

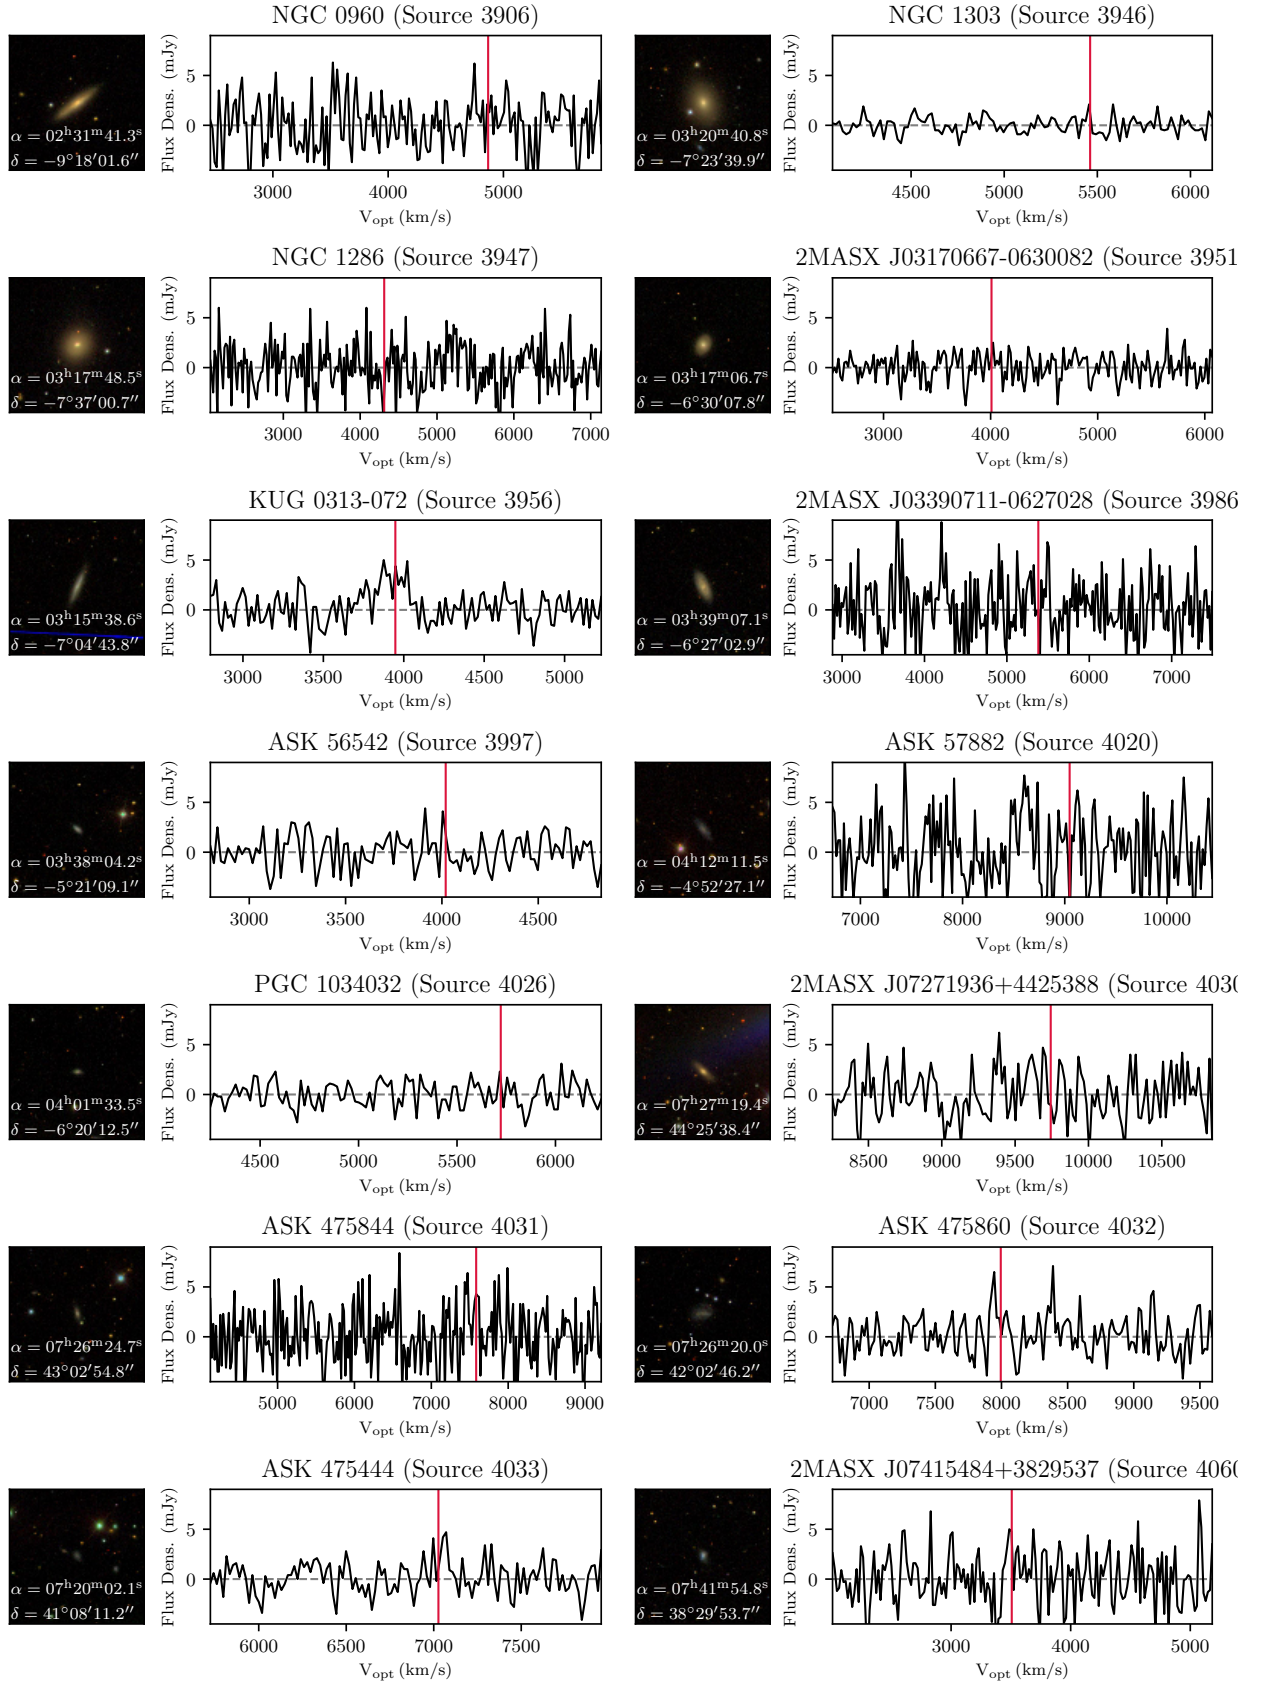

**Figure 1:** (continued) H I non-detected sample.

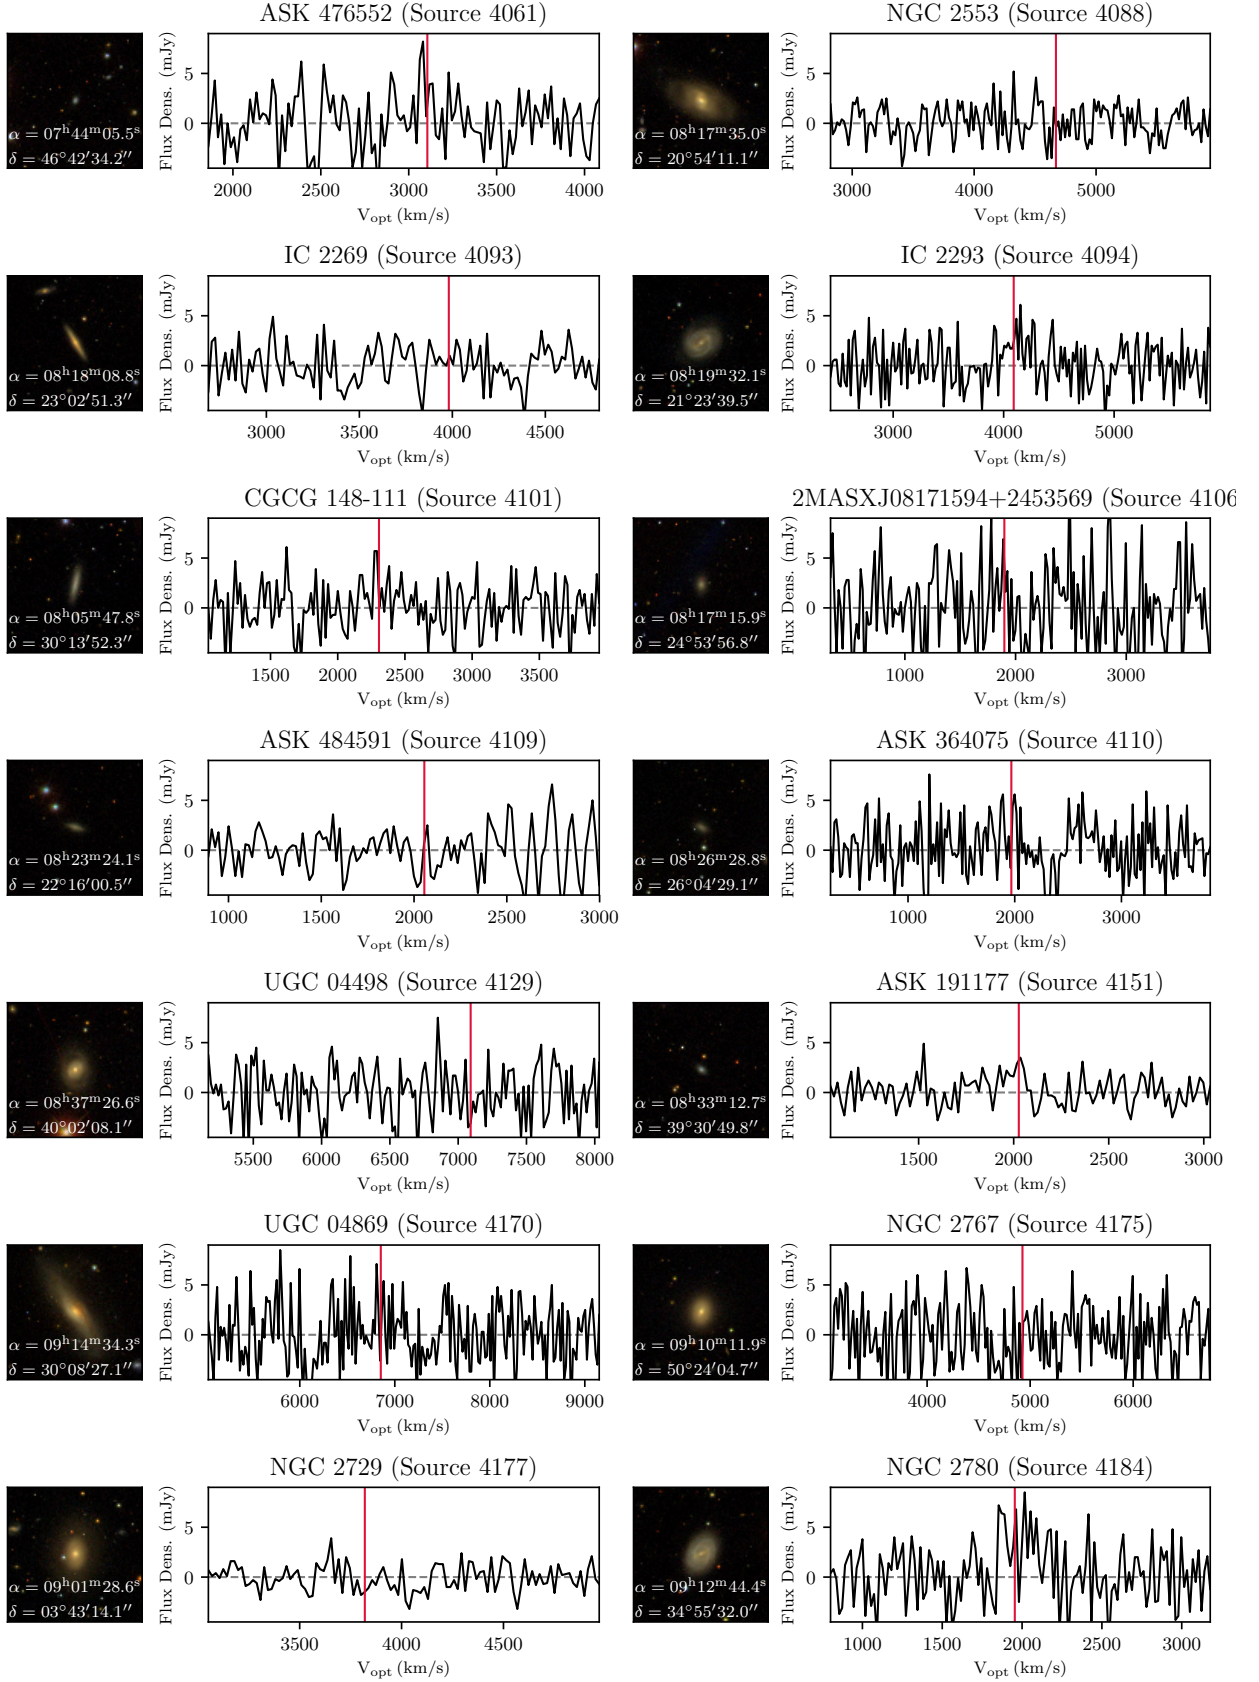

**Figure 1:** (continued) H I non-detected sample.



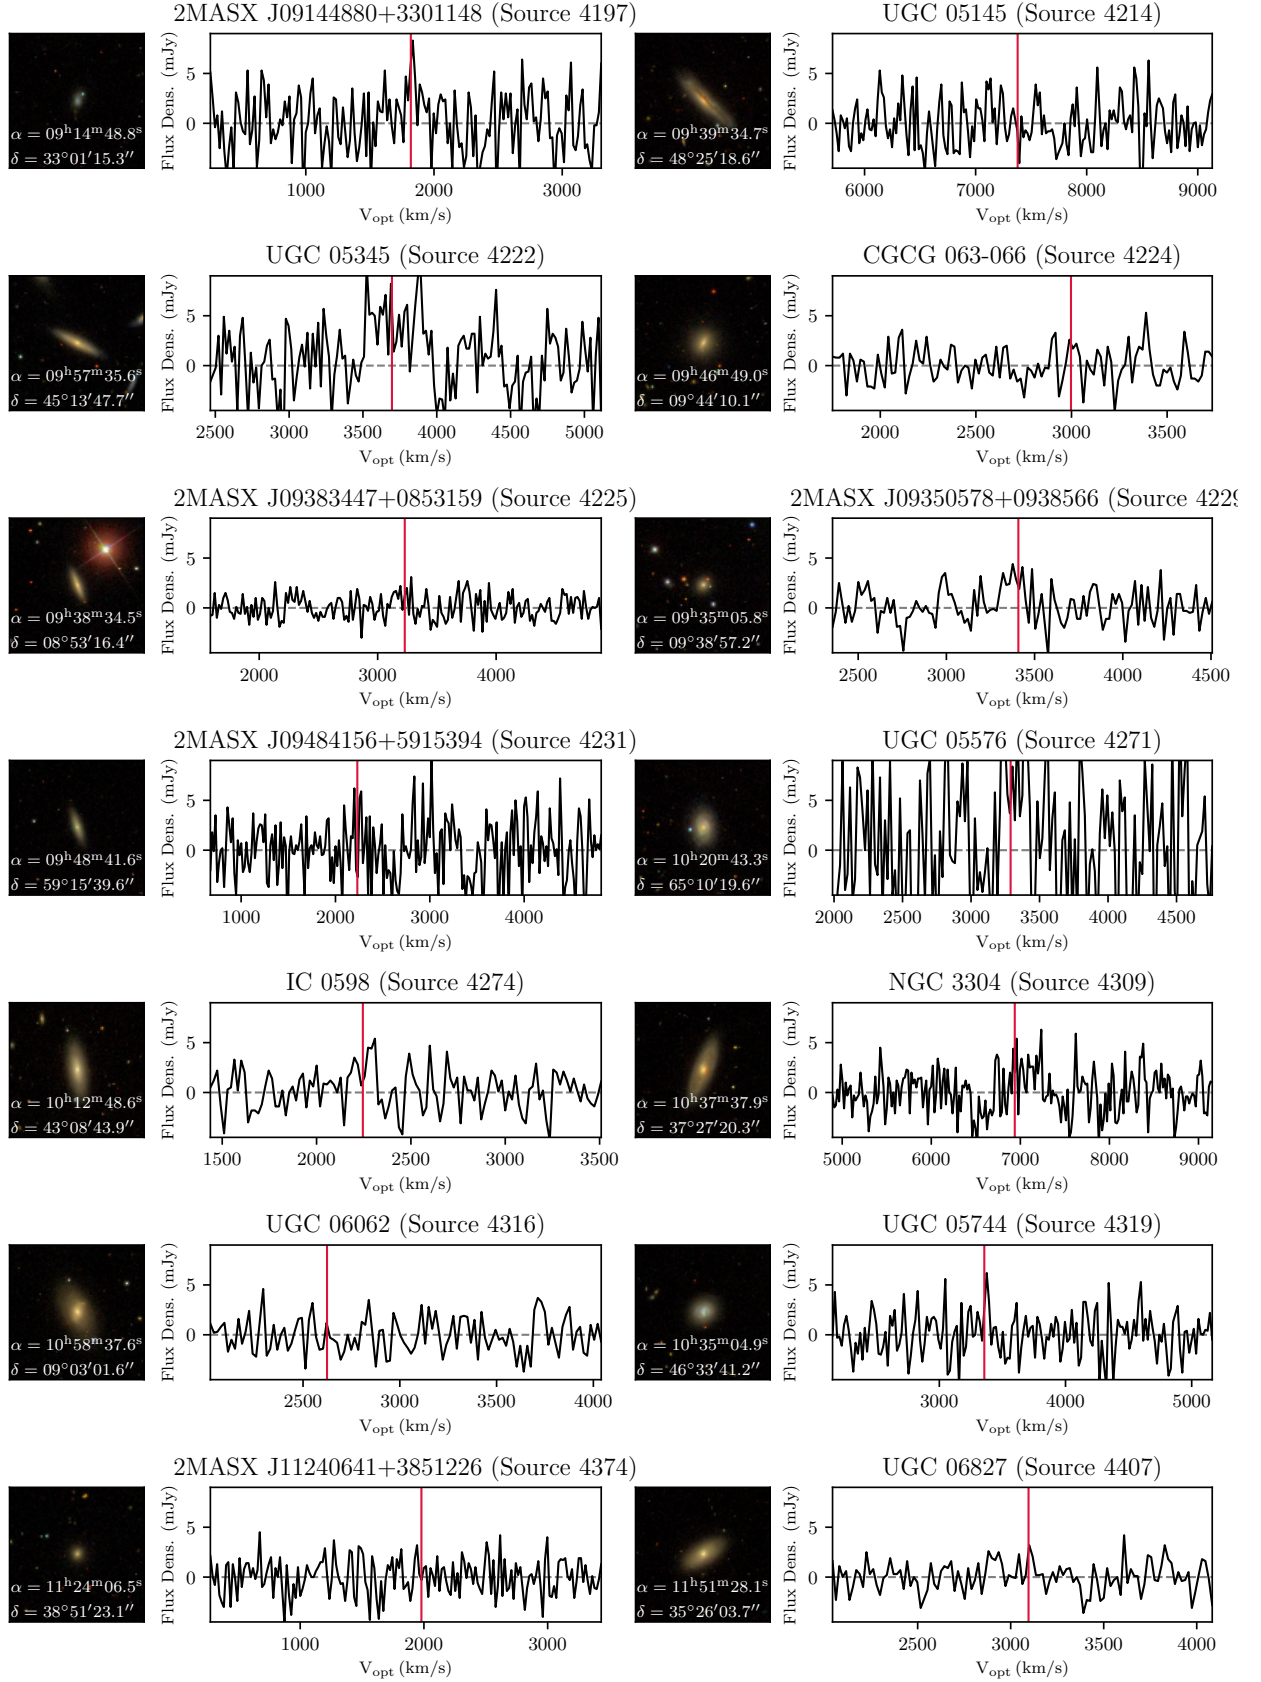

**Figure 1:** (continued) H I non-detected sample.

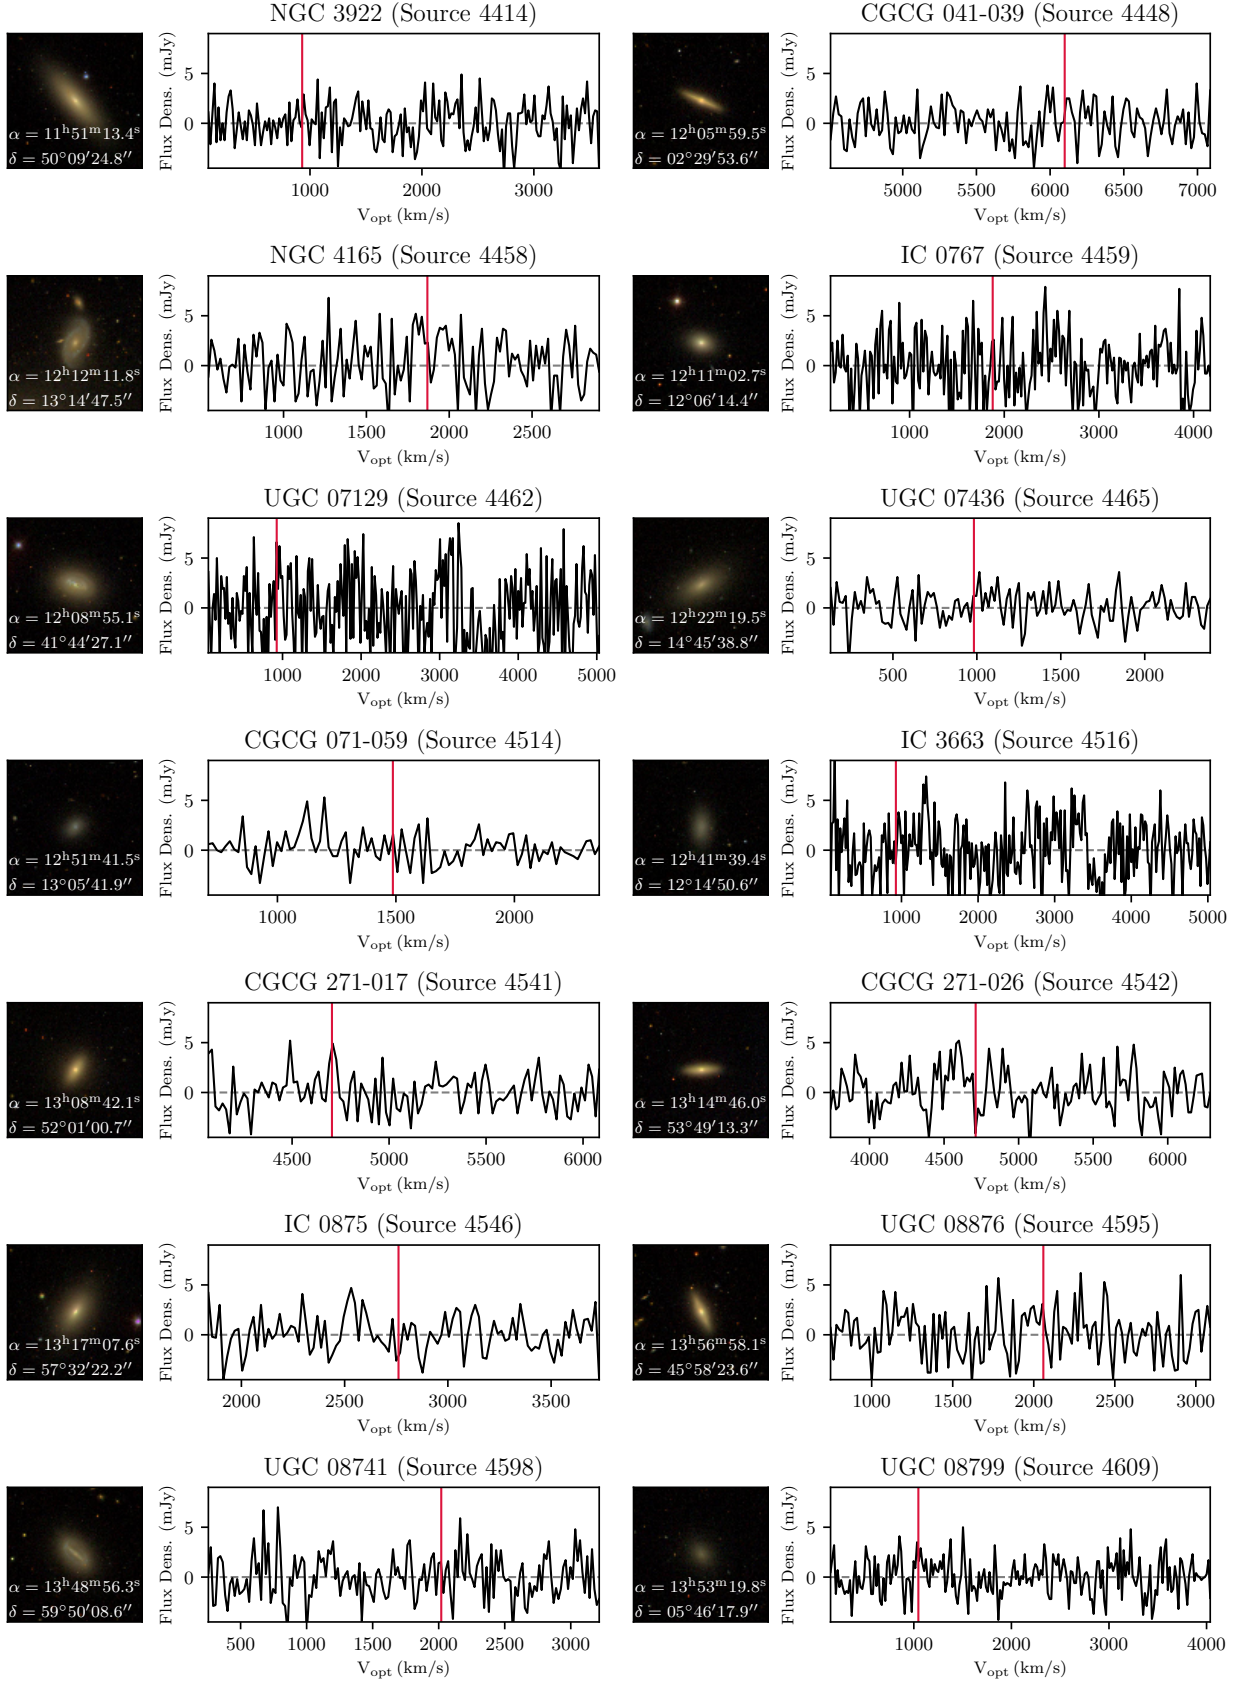

**Figure 1:** (continued) H I non-detected sample.

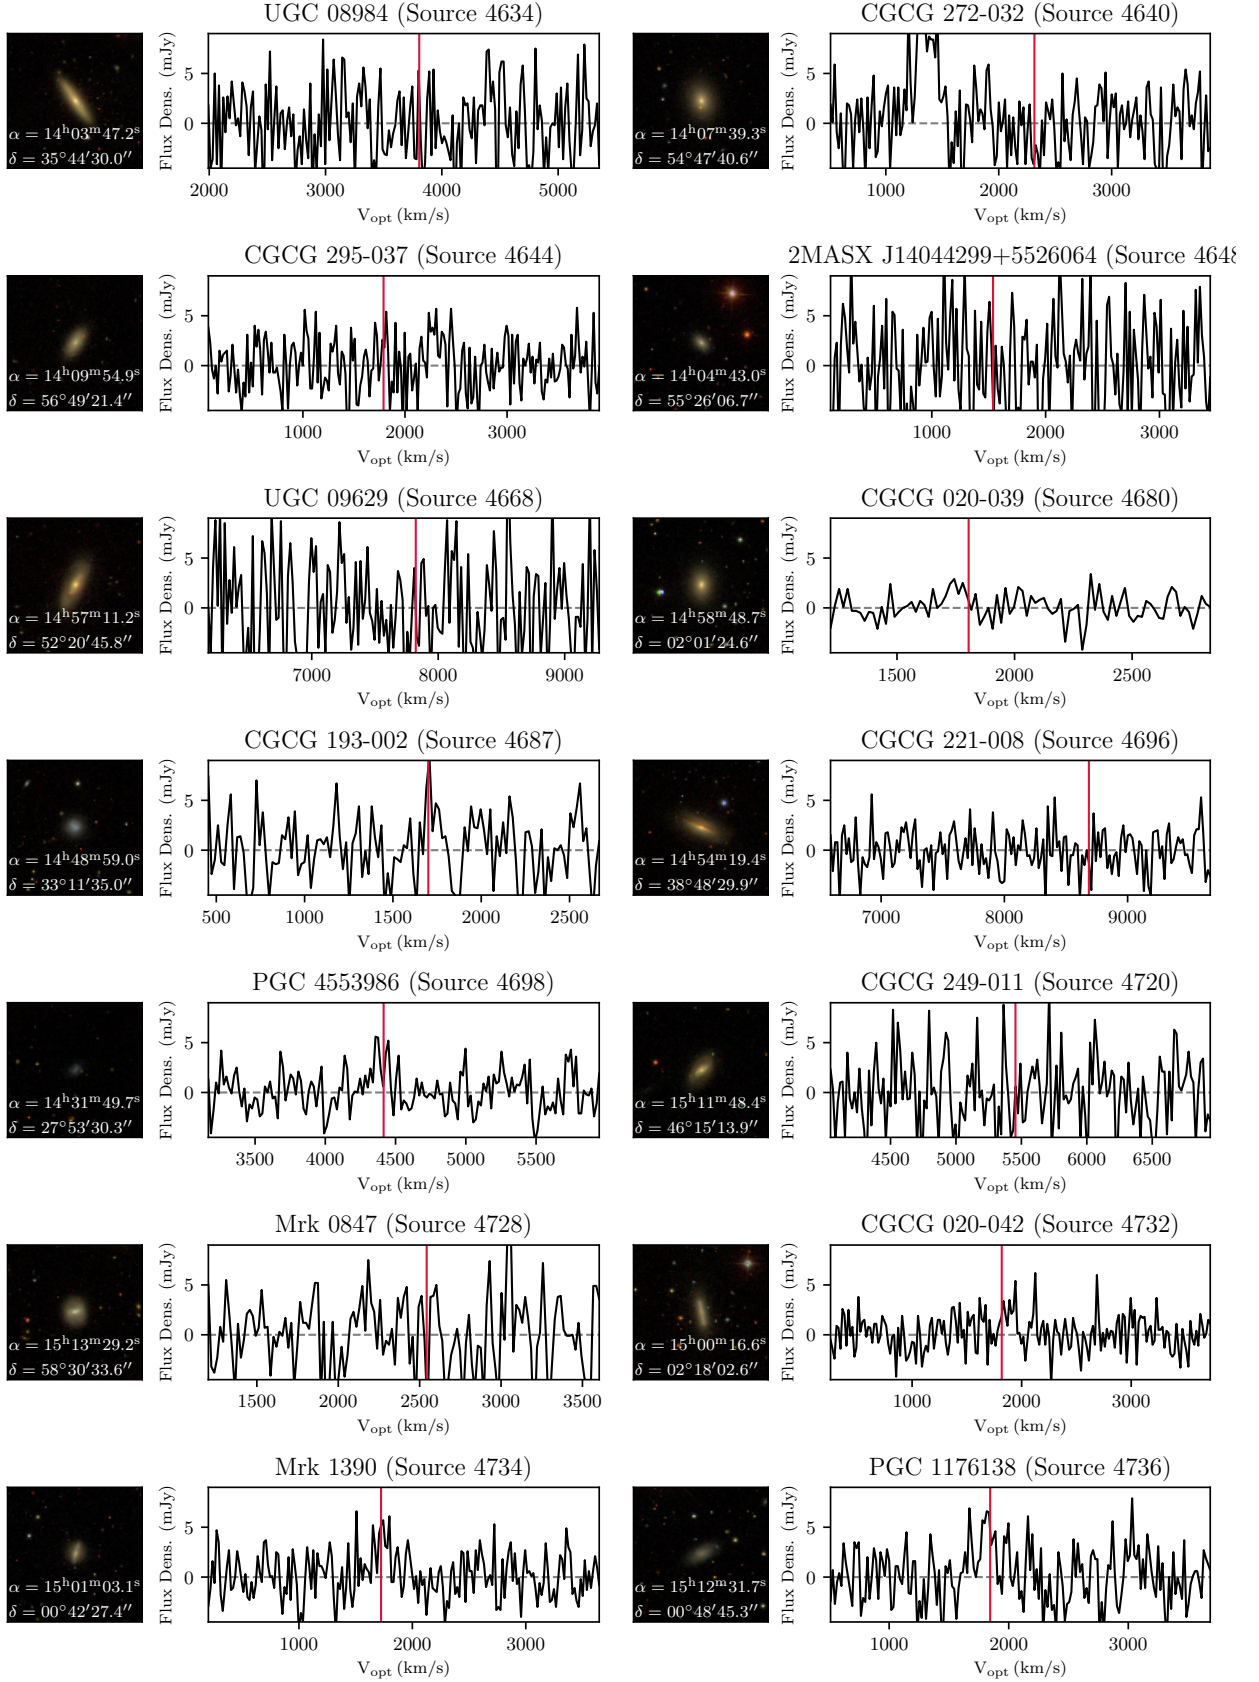

**Figure 1:** (continued) H I non-detected sample.

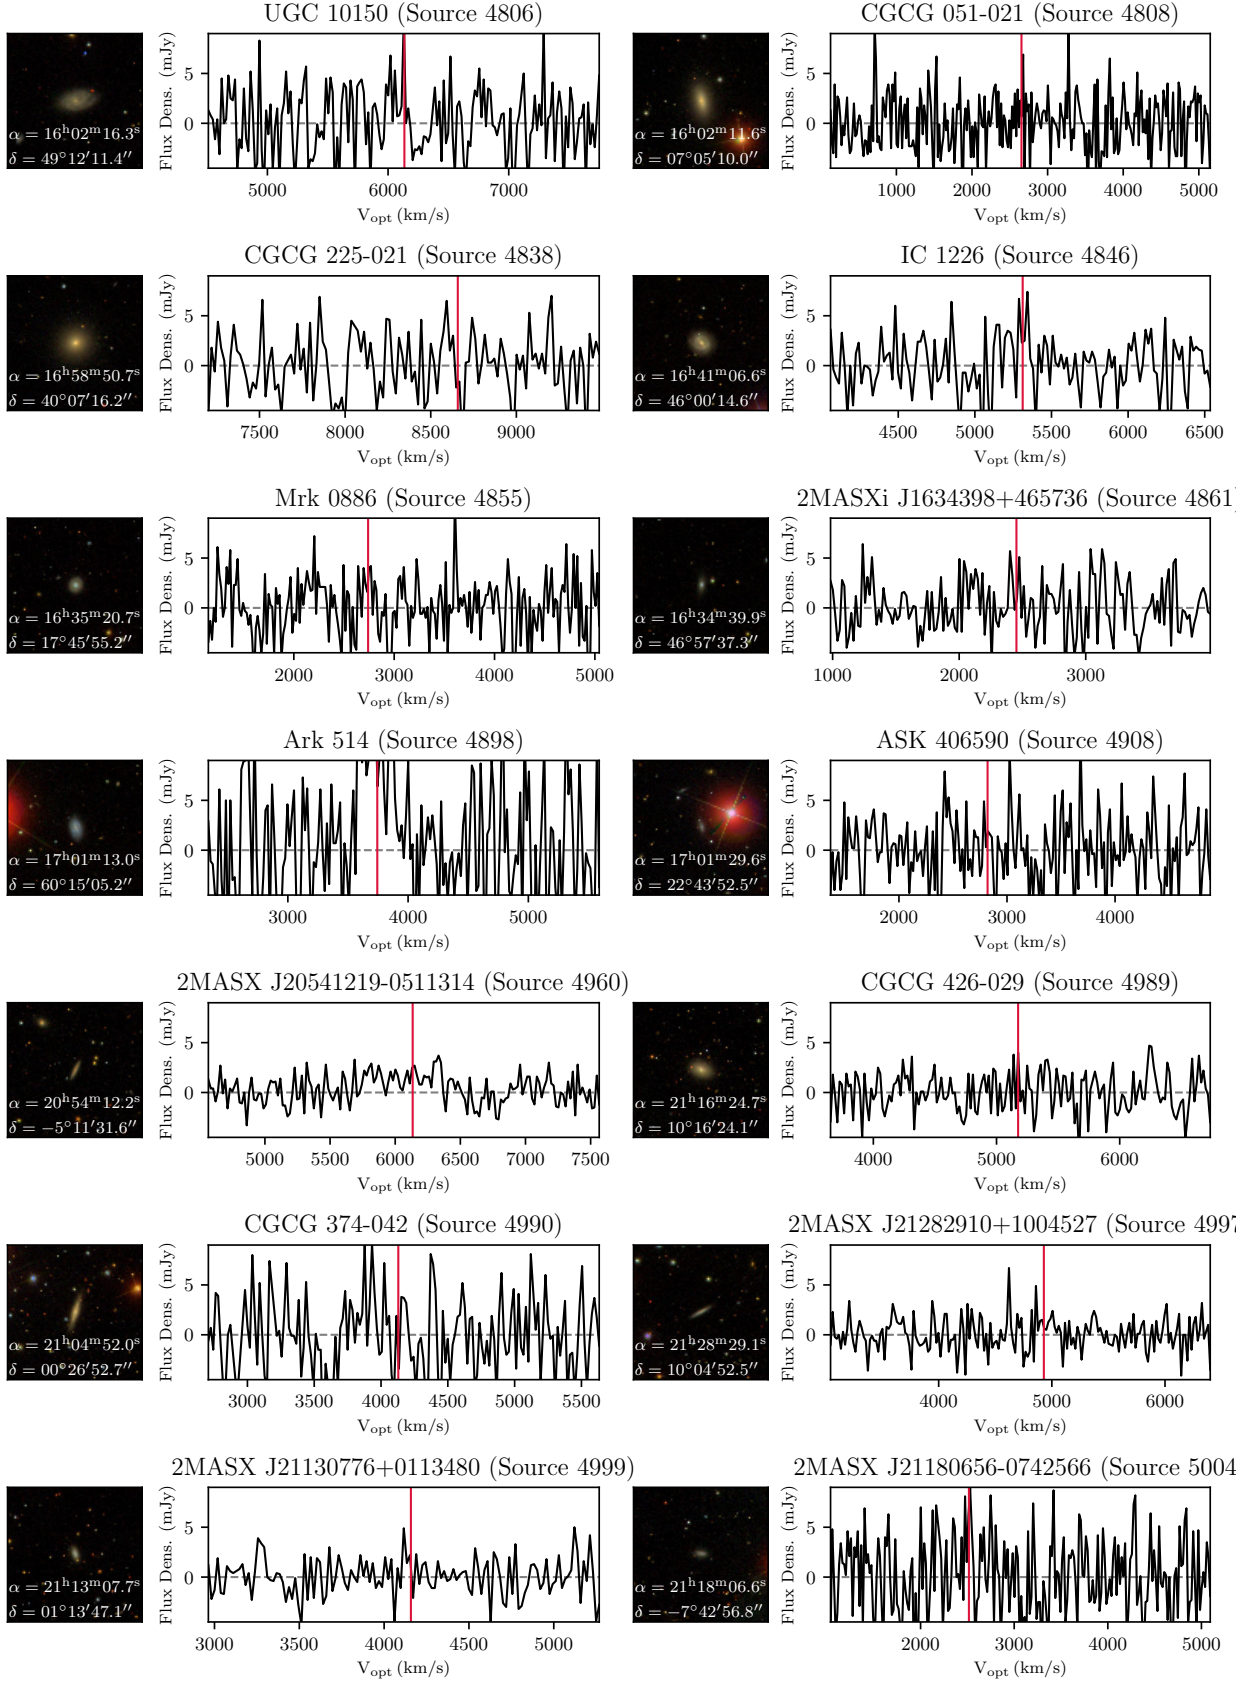

**Figure 1:** (continued) H I non-detected sample.



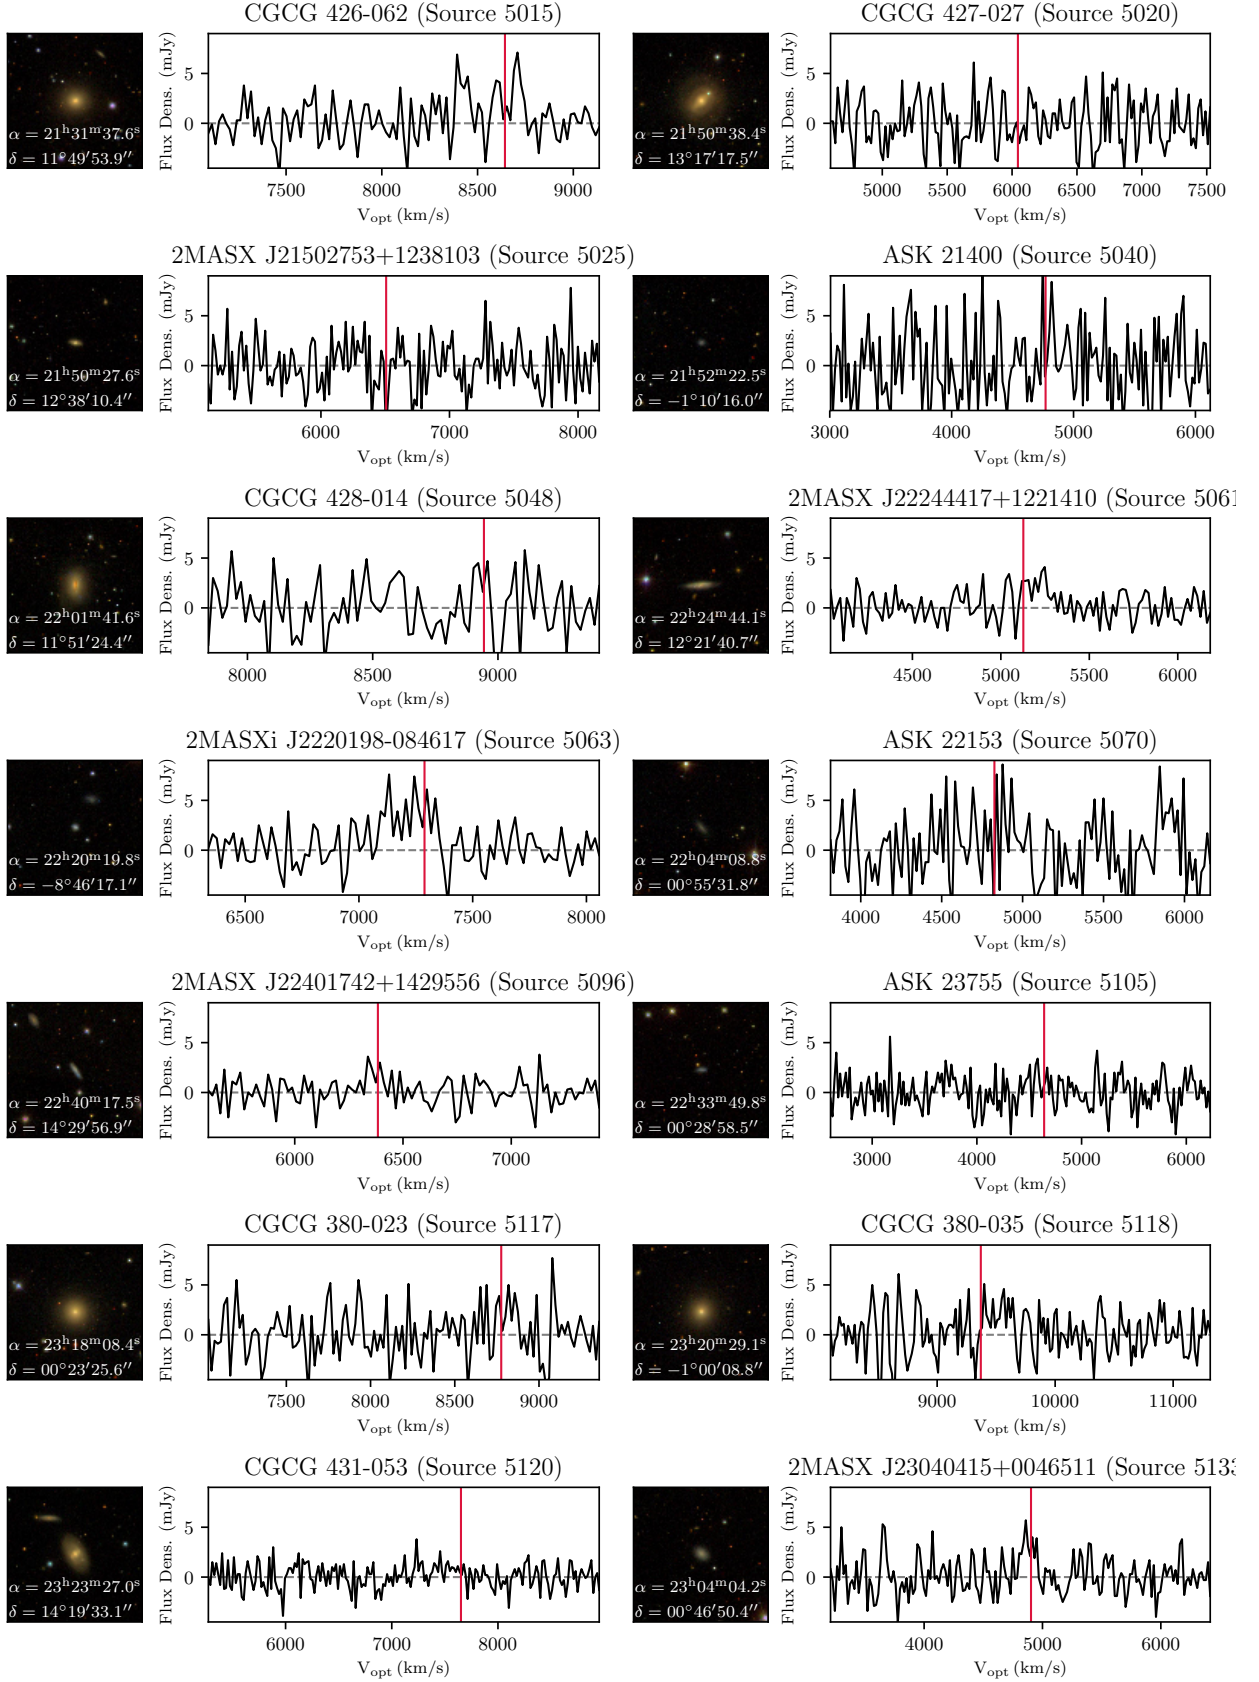

**Figure 1:** (continued) H I non-detected sample.

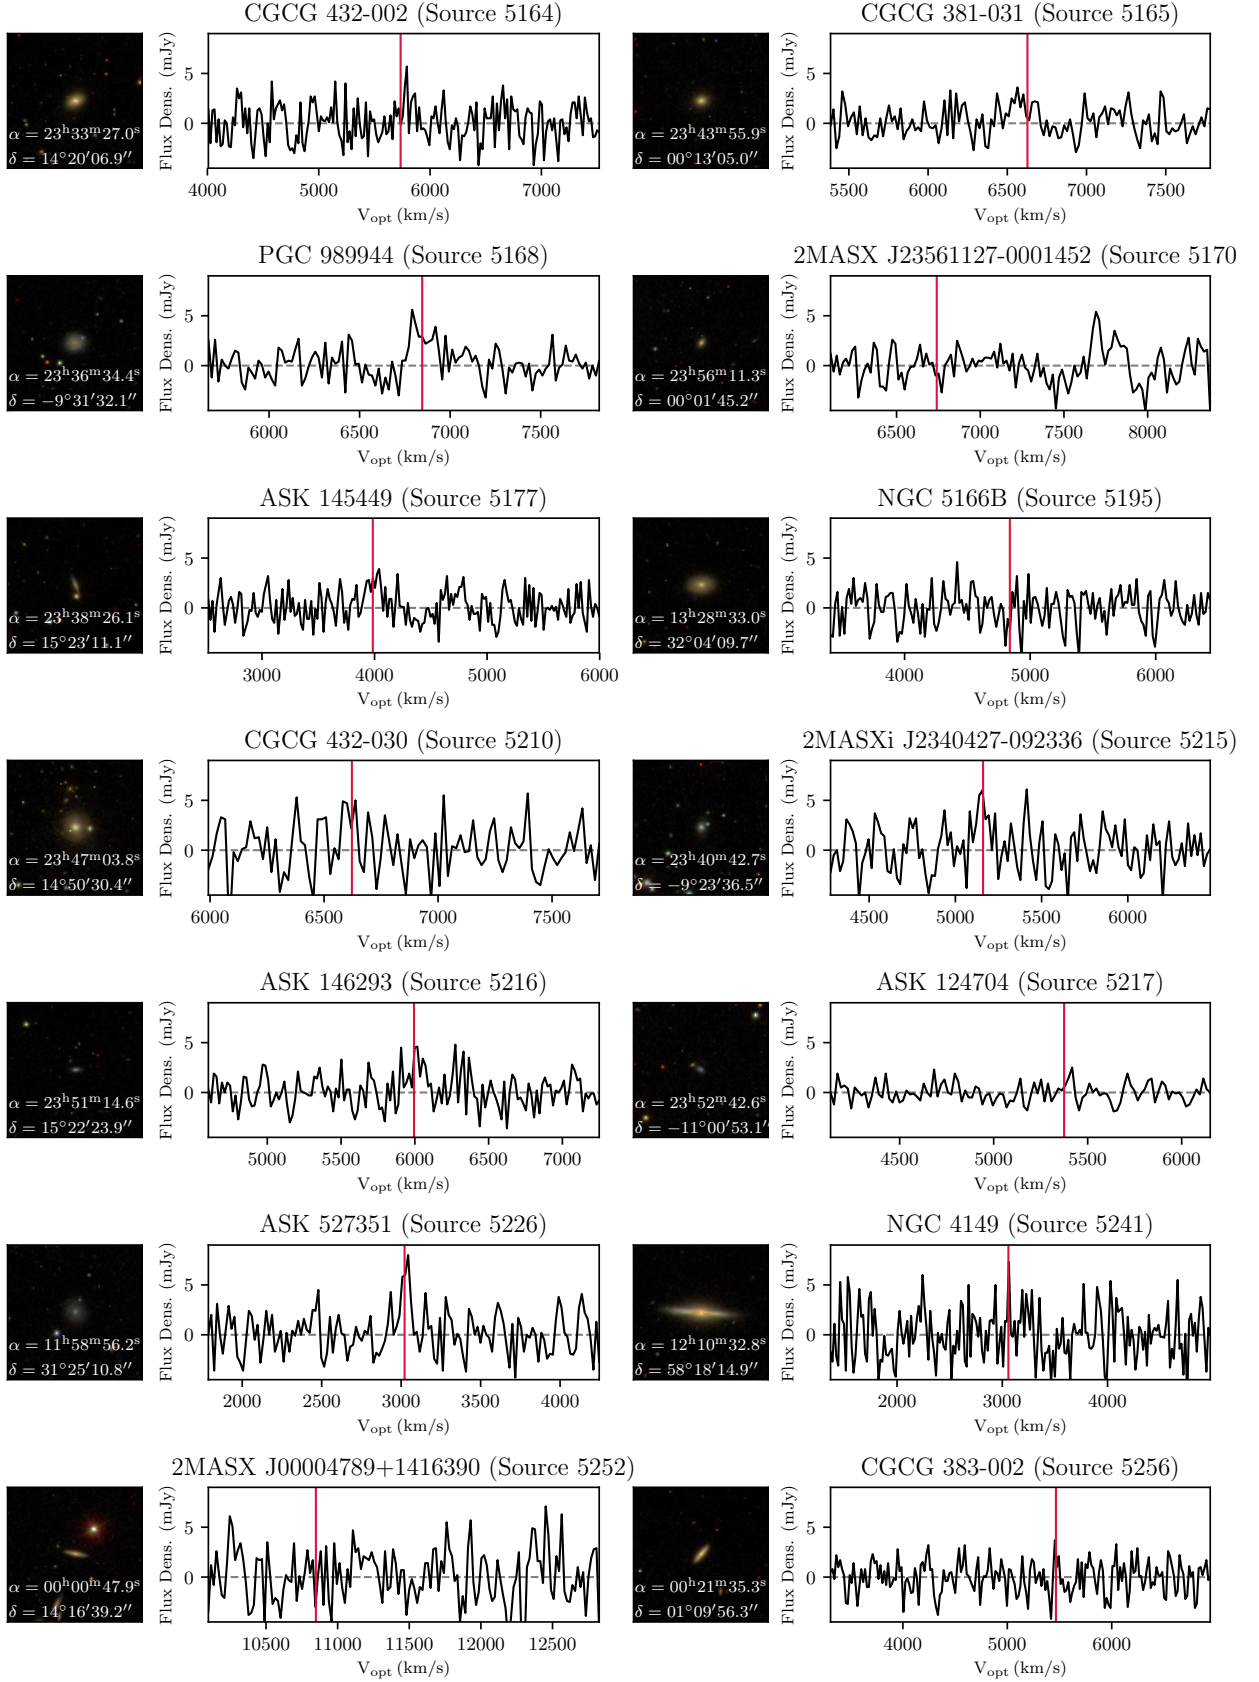

**Figure 1:** (continued) H I non-detected sample.

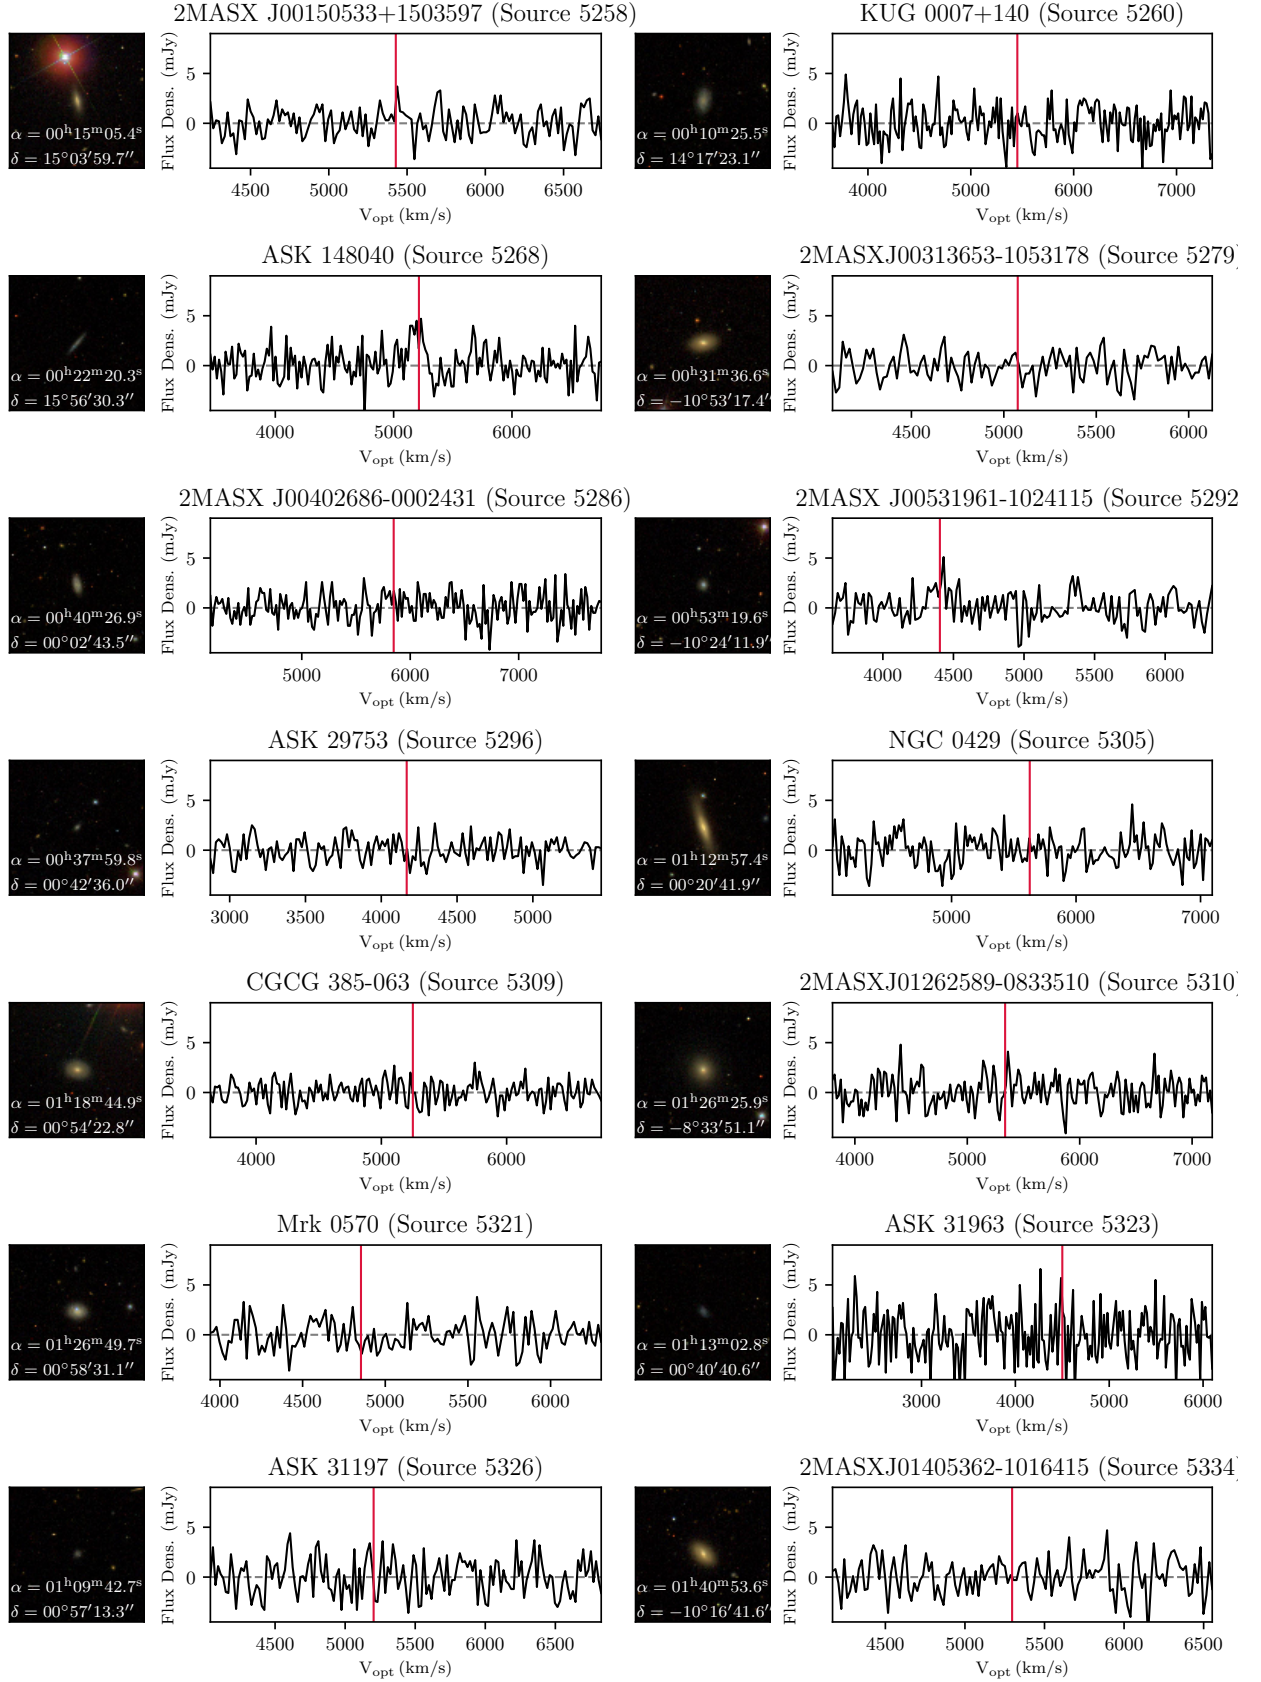

**Figure 1:** (continued) H I non-detected sample.

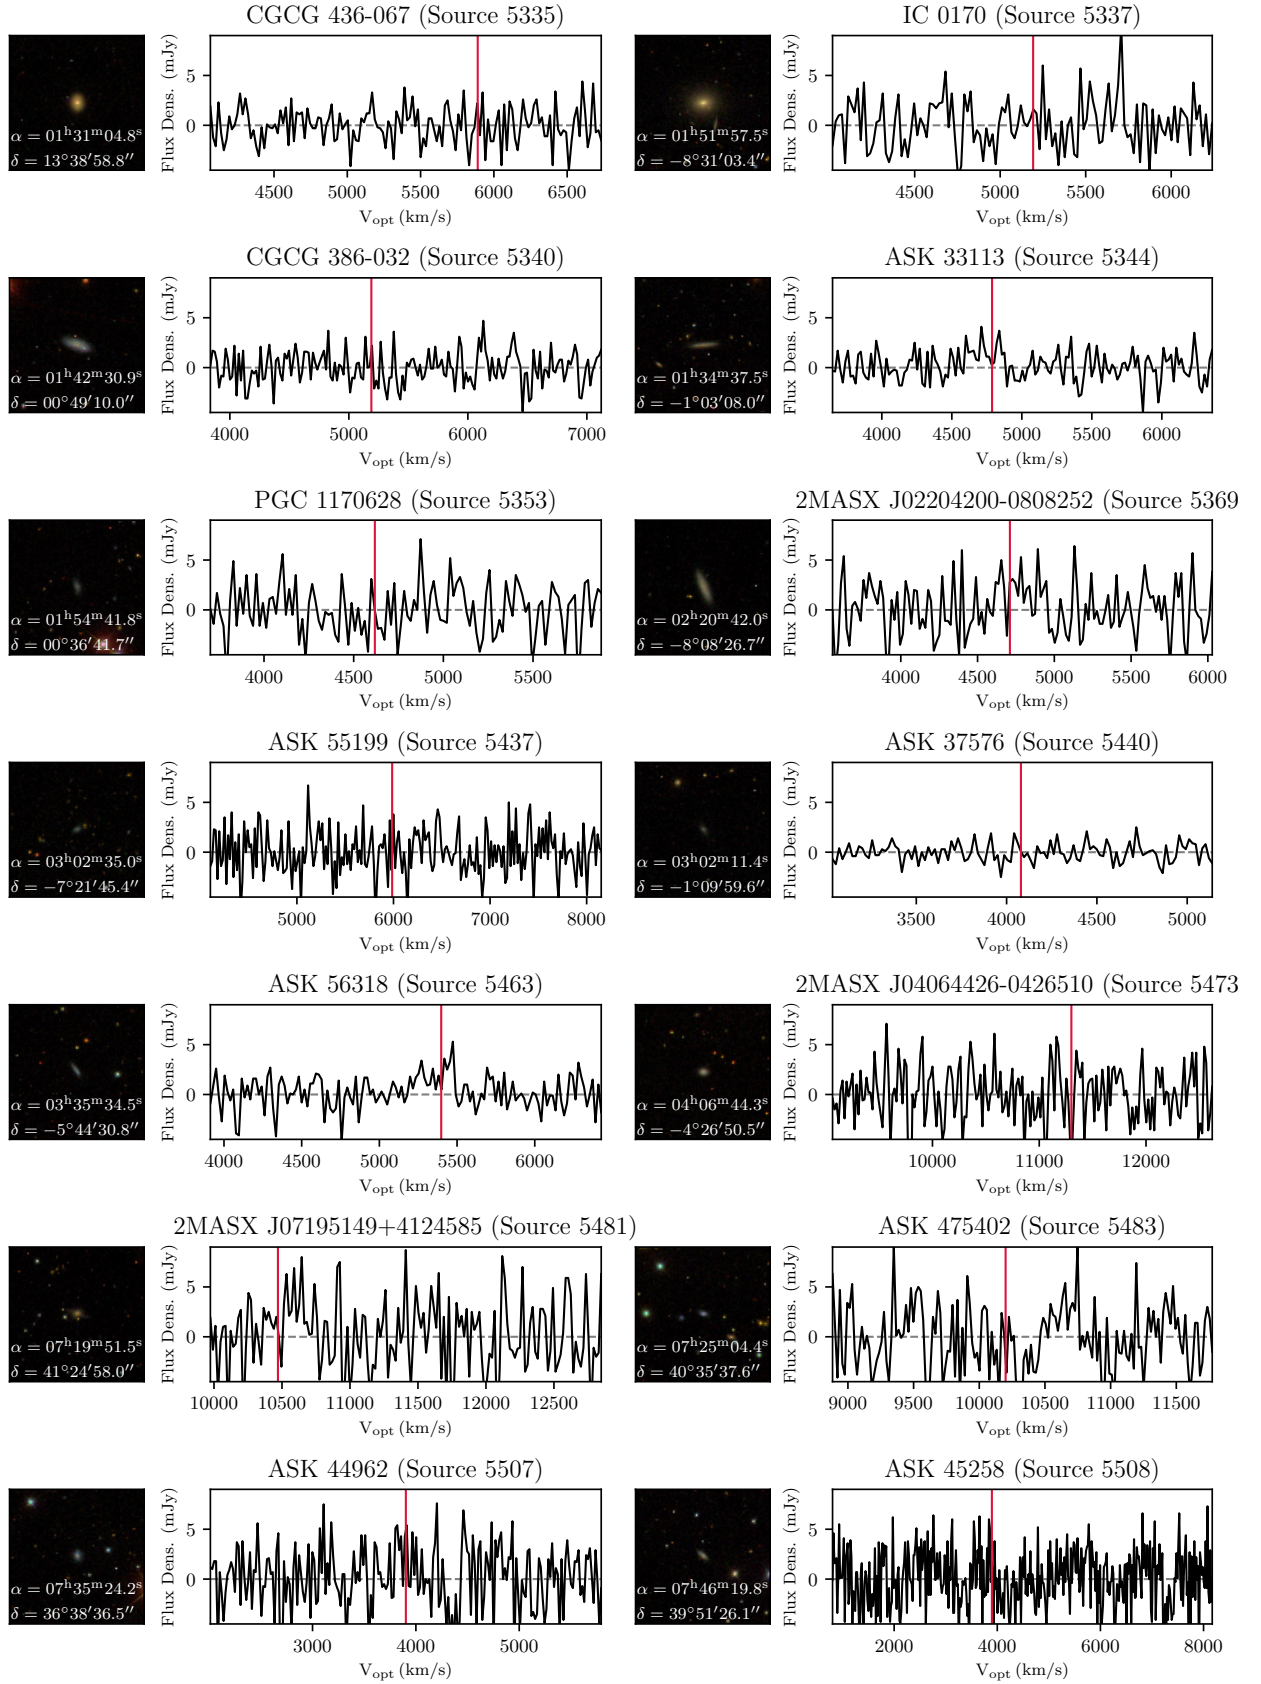

**Figure 1:** (continued) H I non-detected sample.



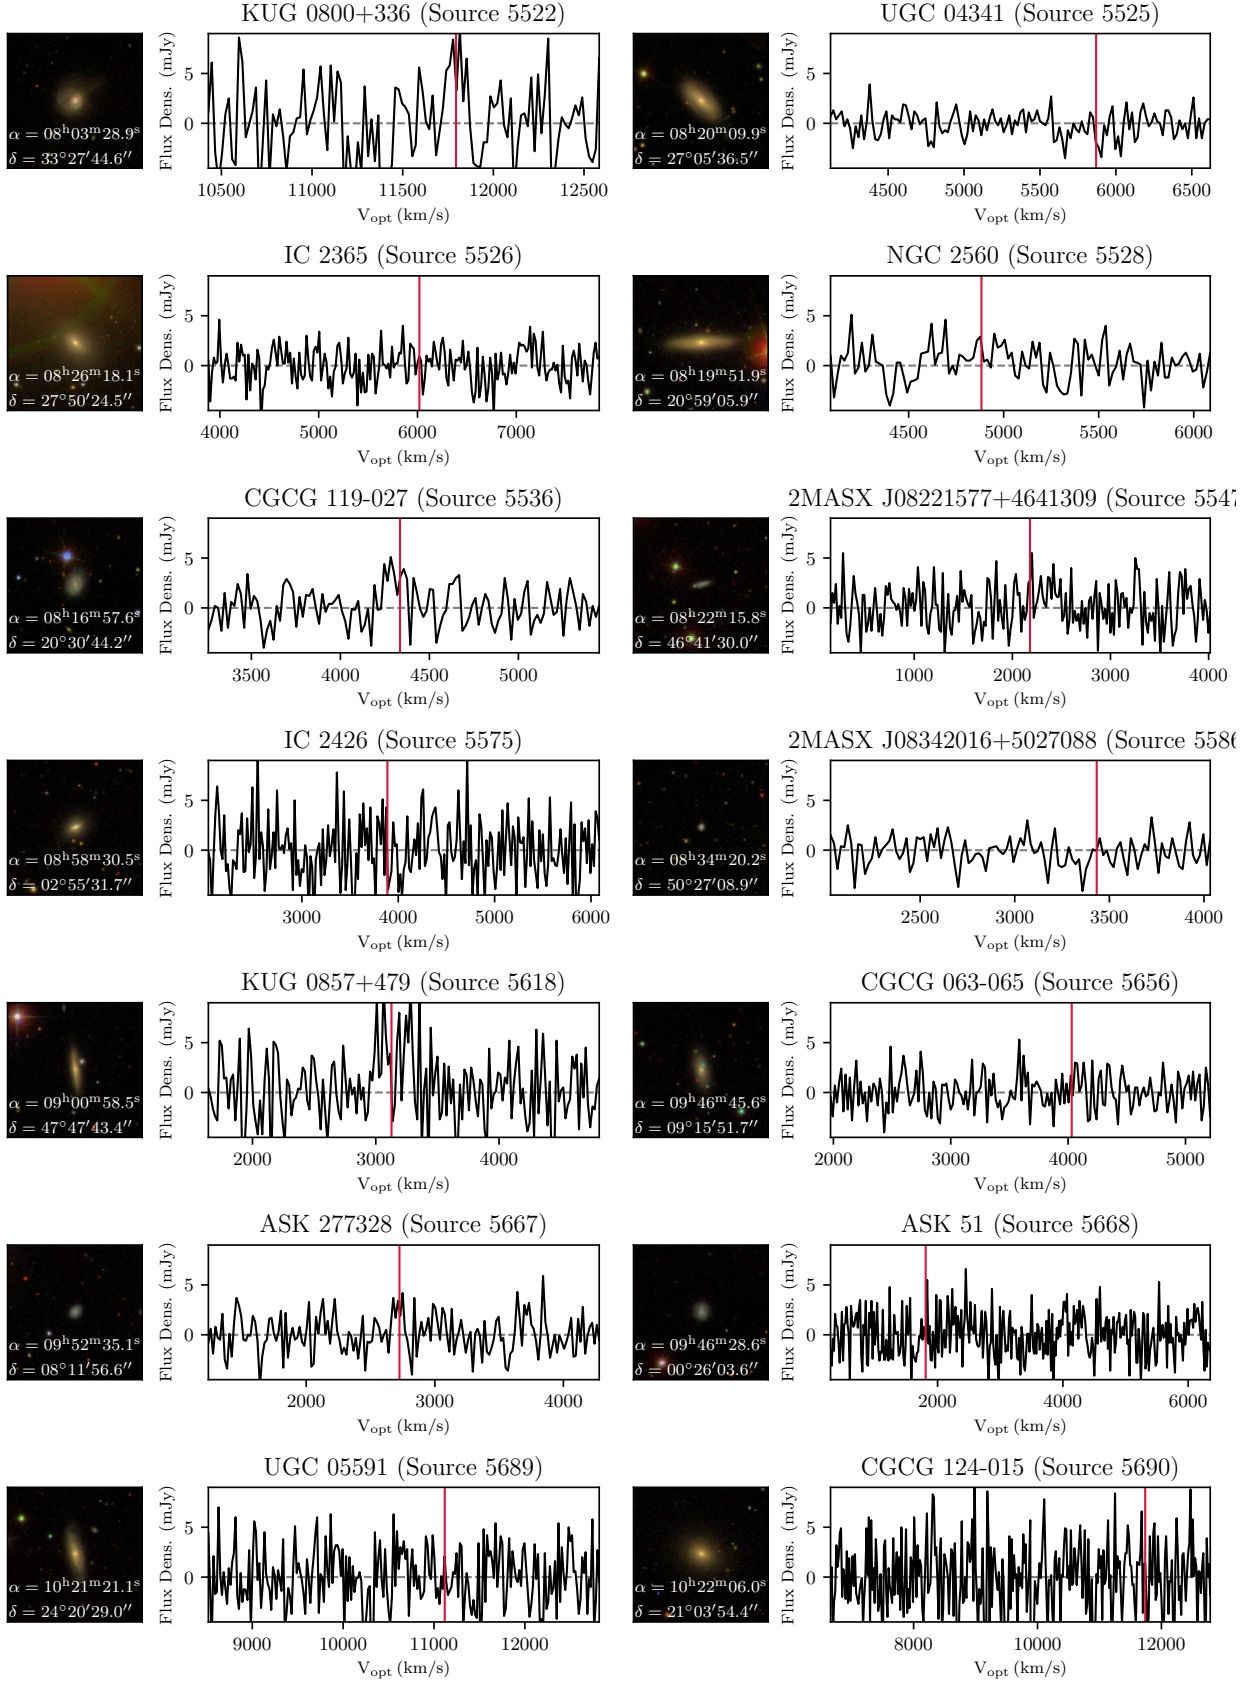

**Figure 1:** (continued) H I non-detected sample.

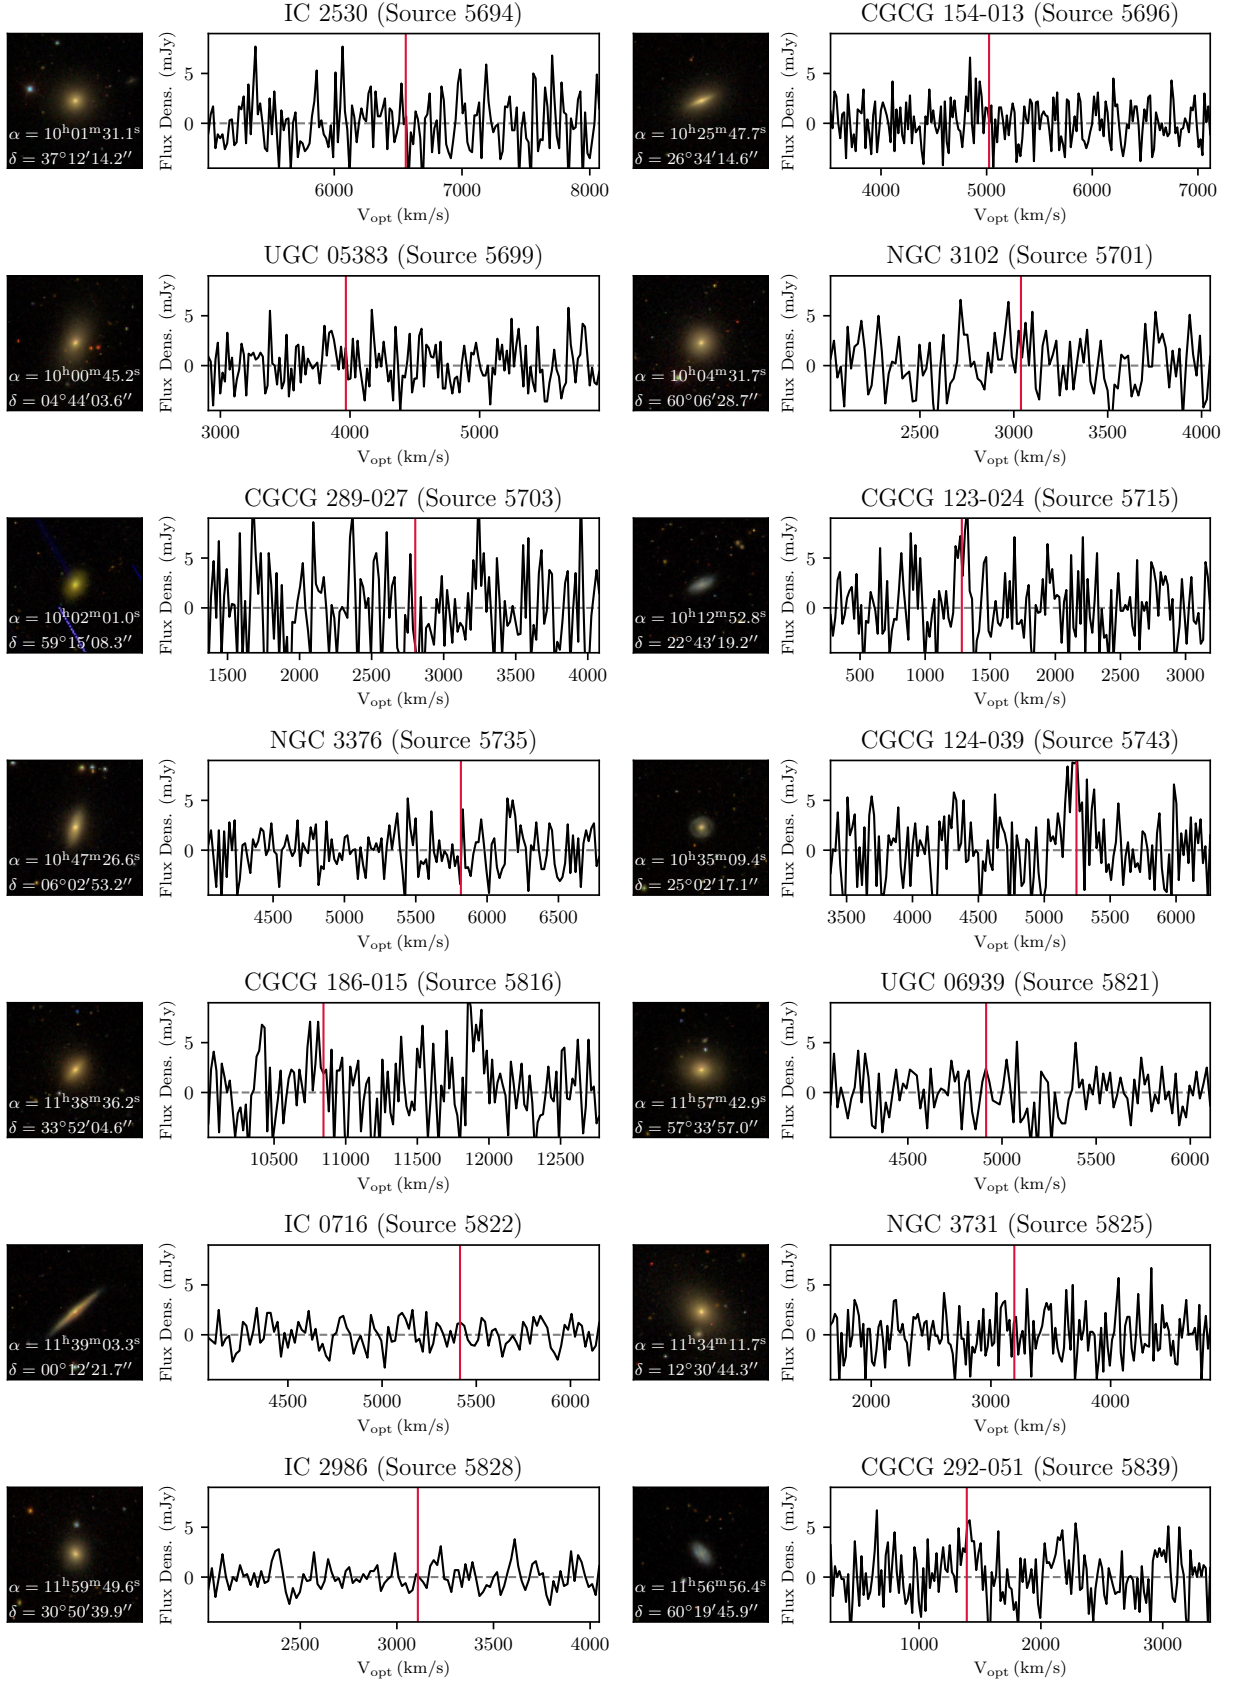

**Figure 1:** (continued) H I non-detected sample.

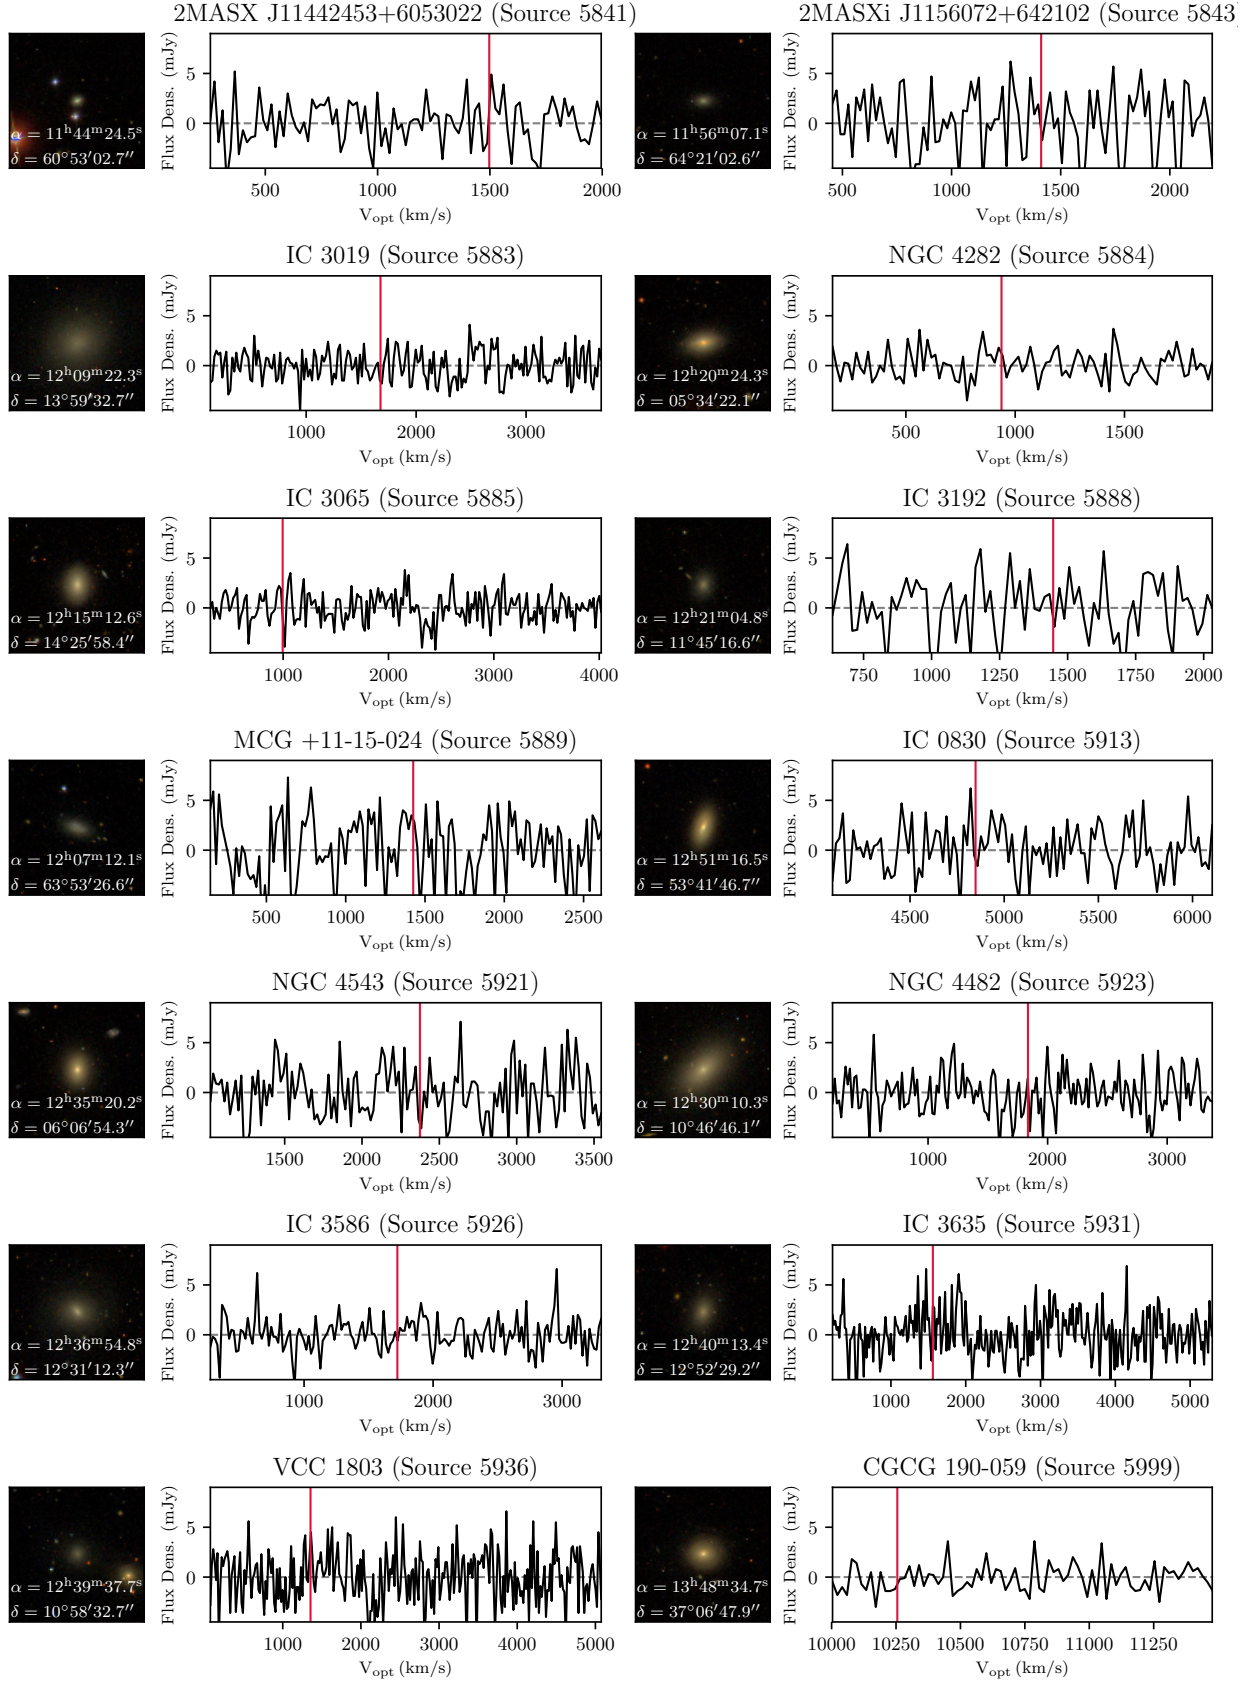

**Figure 1:** (continued) H I non-detected sample.

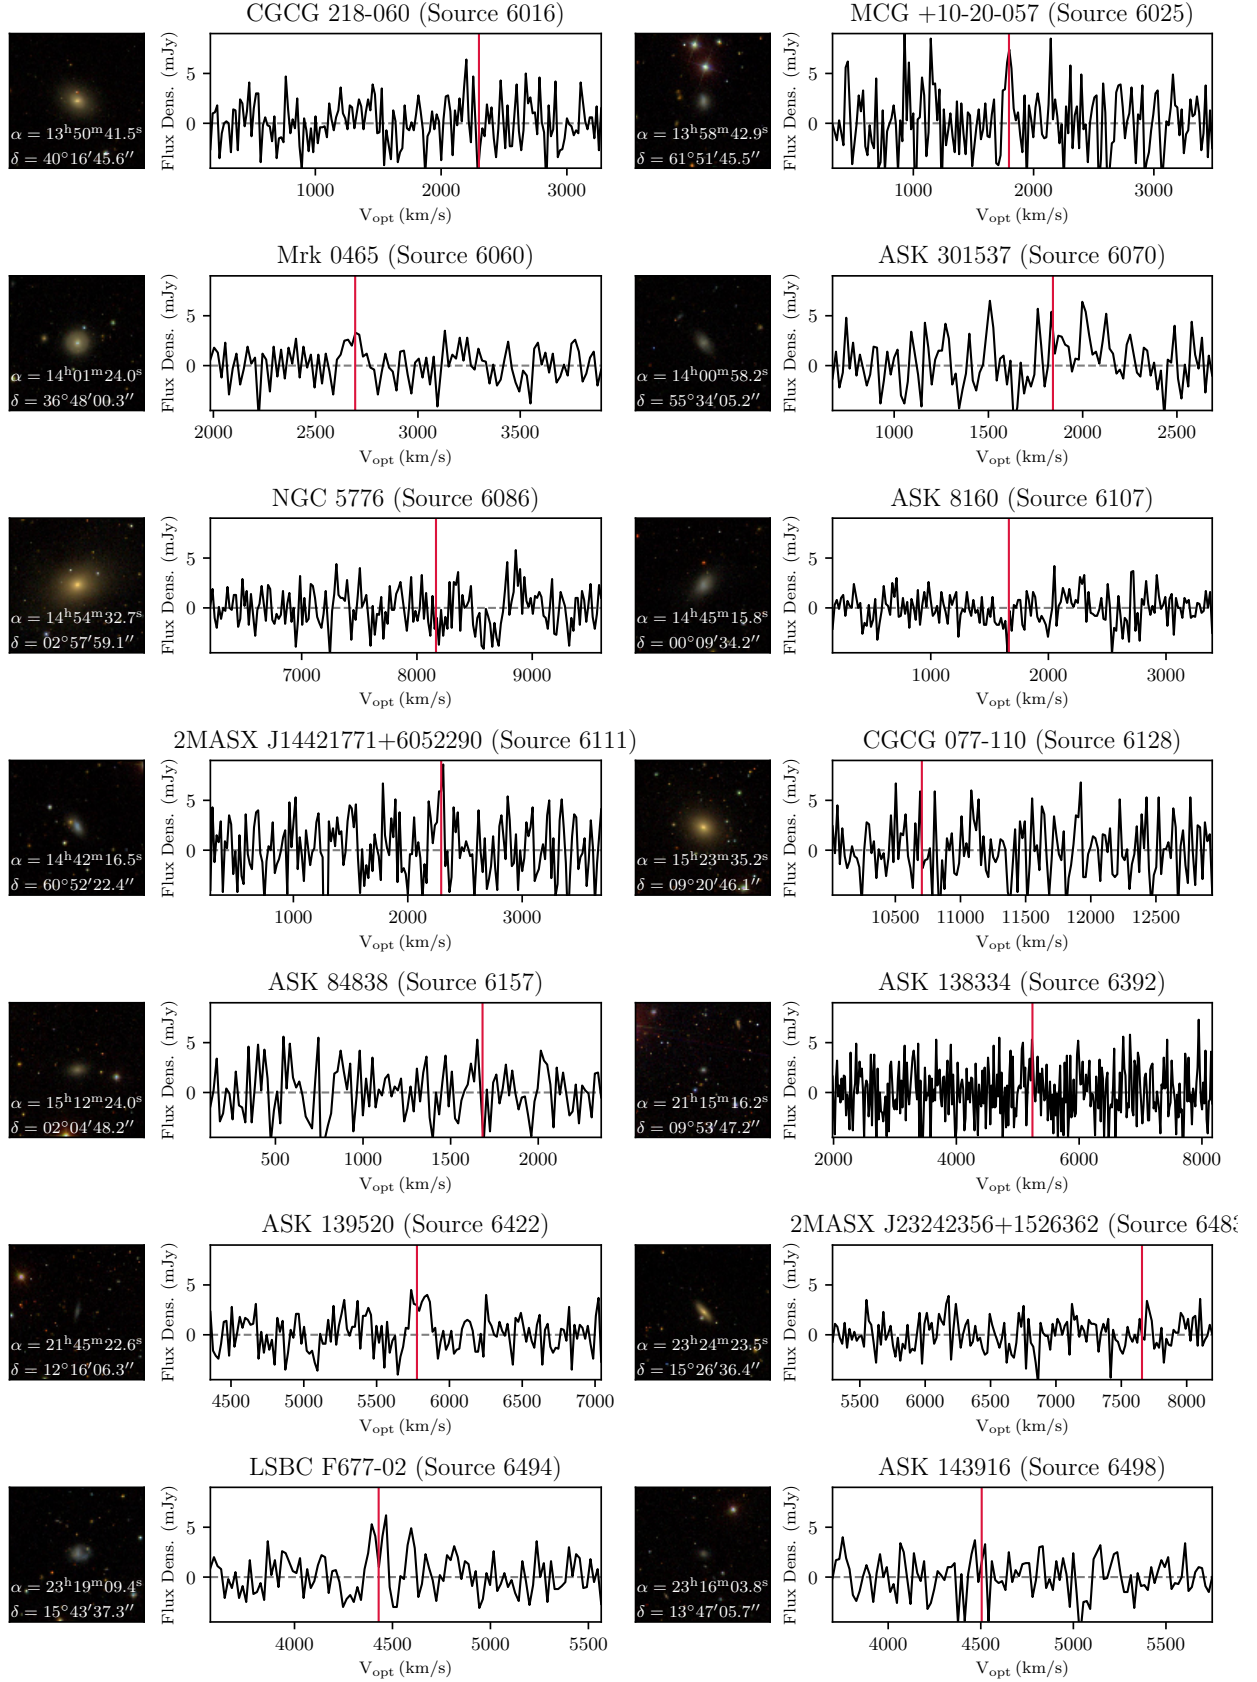

**Figure 1:** (continued) H I non-detected sample.



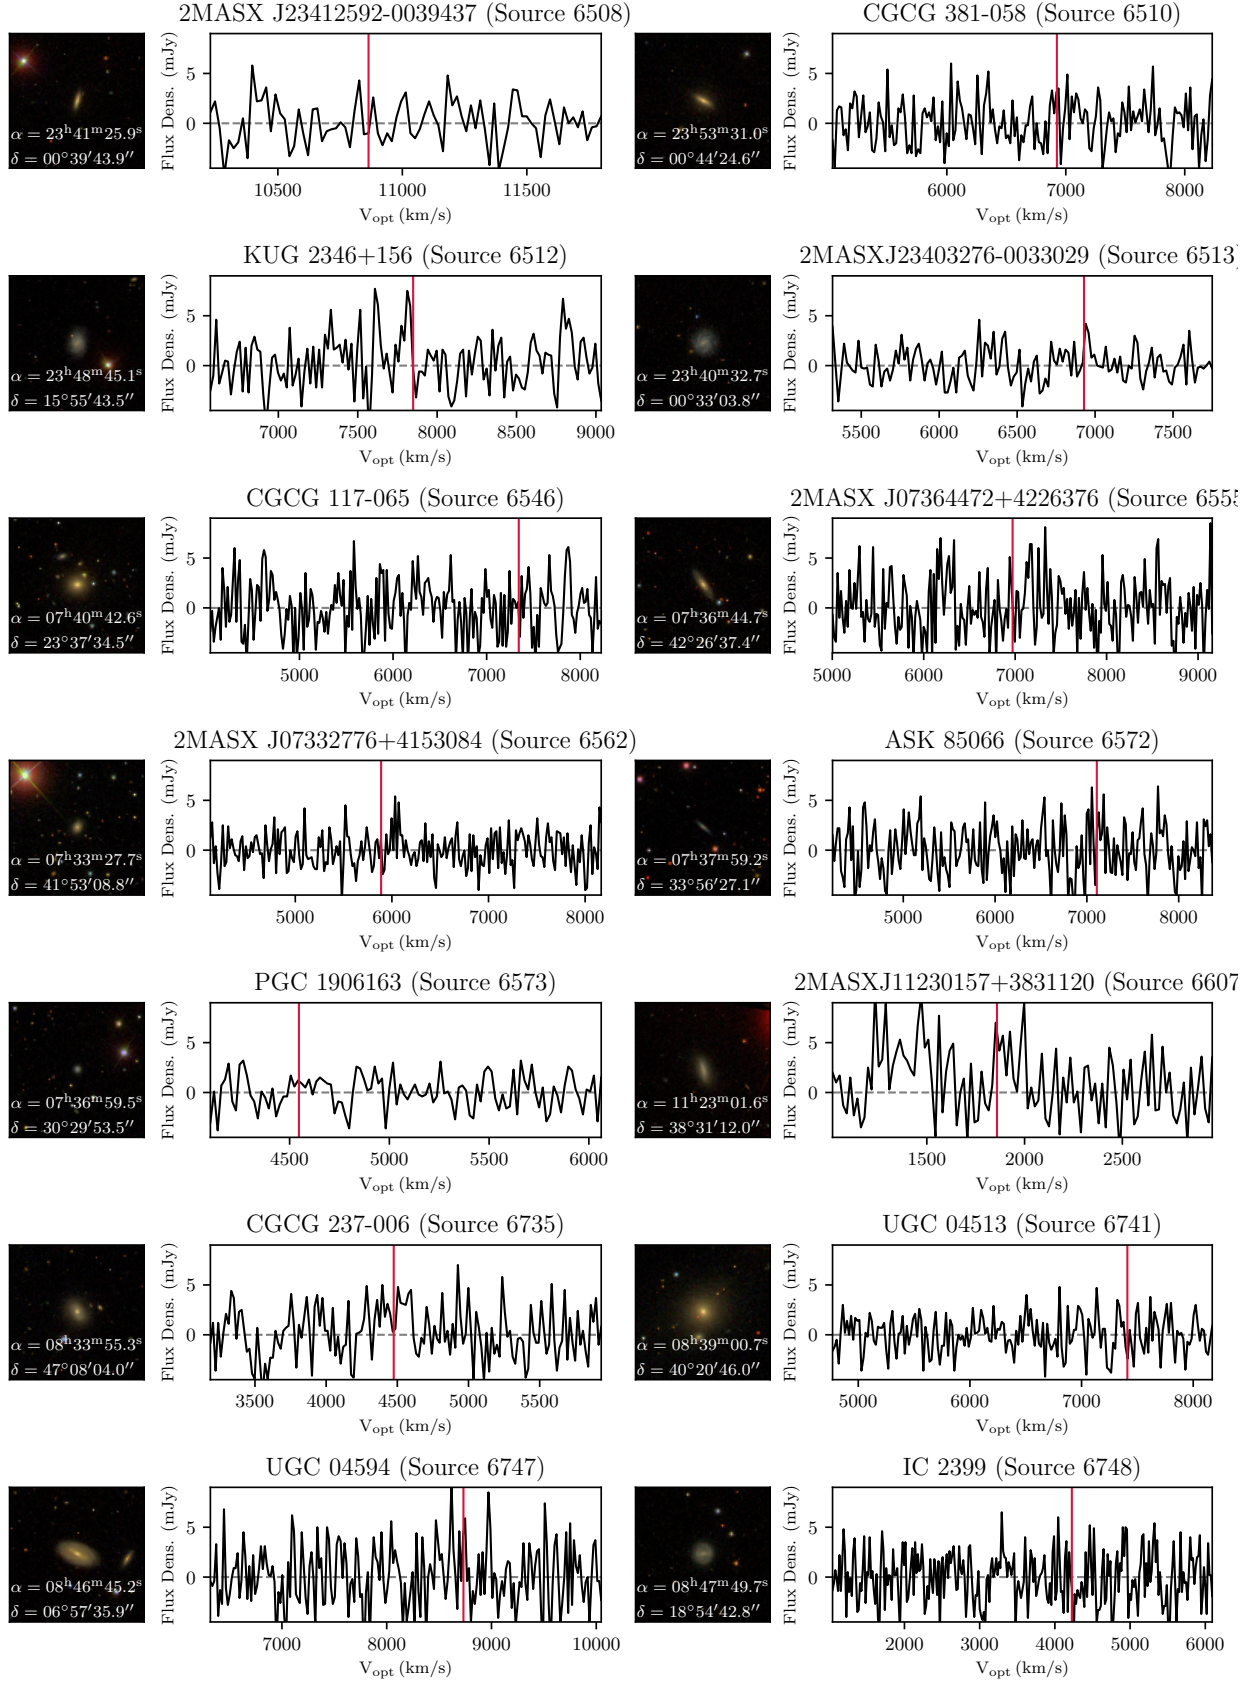

**Figure 1:** (continued) H I non-detected sample.

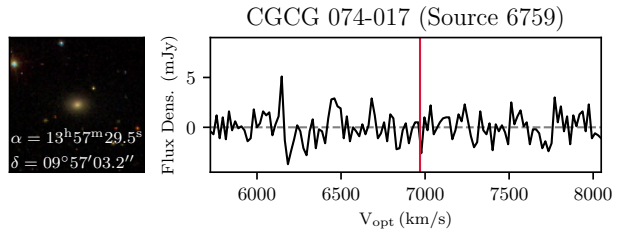

**Figure 1:** (continued) H I non-detected sample.
