# Supplementary material for: HISS, a new tool for H I stacking: application to NIBLES spectra
Source: arXiv:1908.00517 source file (2019-08-01)
Supplement: Supplementary file 2 [file crumbs_table.tex]

$1926$ & $11\, 23\, 18.84$ & $03\, 57\, 18.78$ & CGCG 039-161 & $1582 \pm 19 $ & $1.91$ & $-16.18$ & $8.23$\\
	$1954$ & $11\, 49\, 12.79$ & $-03\, 39\, 34.64$ & PGC 1068442 & $1572 \pm 3 $ & $1.57$ & $-15.78$ & $8.04$\\
	$2012$ & $12\, 19\, 21.12$ & $04\, 46\, 24.49$ & ASK 173829 & $2065 \pm 2 $ & $1.61$ & $-15.87$ & $8.09$\\
	$2244$ & $14\, 04\, 15.84$ & $04\, 06\, 43.85$ & UGC 08986 & $1239 \pm 3 $ & $2.19$ & $-17.79$ & $9.08$\\
	$2272$ & $14\, 25\, 08.99$ & $-01\, 06\, 48.52$ & CGCG 019-019 & $2643 \pm 3 $ & $2.11$ & $-17.94$ & $9.21$\\
	$2442$ & $15\, 17\, 29.45$ & $03\, 35\, 07.94$ & PGC 3124577 & $1882 \pm 2 $ & $1.62$ & $-15.69$ & $8.03$\\
	$2525$ & $09\, 35\, 44.04$ & $31\, 42\, 19.68$ & NGC 2918 & $6756 \pm 2 $ & $2.65$ & $-22.64$ & $11.28$\\
	$2533$ & $10\, 06\, 07.44$ & $47\, 15\, 45.53$ & NGC 3111 & $7437 \pm 2 $ & $2.68$ & $-22.52$ & $11.19$\\
	$2535$ & $14\, 30\, 25.58$ & $11\, 55\, 40.77$ & NGC 5644 & $7649 \pm 2 $ & $2.72$ & $-22.87$ & $11.33$\\
	$2541$ & $13\, 53\, 38.43$ & $36\, 08\, 02.57$ & NGC 5352 & $7956 \pm 3 $ & $2.81$ & $-22.64$ & $11.26$\\
	$2565$ & $00\, 35\, 59.83$ & $-10\, 07\, 18.07$ & NGC 0163 & $5917 \pm 4 $ & $2.70$ & $-22.05$ & $11.01$\\
	$2574$ & $11\, 00\, 35.40$ & $12\, 09\, 41.65$ & NGC 3491 & $6351 \pm 2 $ & $2.72$ & $-21.98$ & $11.06$\\
	$2589$ & $12\, 19\, 32.09$ & $49\, 48\, 56.71$ & UGC 07367 & $4093 \pm 2 $ & $2.60$ & $-21.45$ & $10.78$\\
	$2597$ & $12\, 19\, 32.59$ & $56\, 44\, 11.69$ & NGC 4271 & $4756 \pm 2 $ & $2.82$ & $-21.84$ & $10.93$\\
	$2606$ & $14\, 41\, 32.96$ & $38\, 51\, 04.95$ & UGC 09473 & $4669 \pm 2 $ & $2.17$ & $-21.54$ & $10.80$\\
	$2614$ & $12\, 12\, 17.27$ & $13\, 12\, 18.72$ & NGC 4168 & $2273 \pm 2 $ & $2.44$ & $-21.43$ & $10.63$\\
	$2615$ & $12\, 32\, 47.65$ & $63\, 56\, 21.18$ & NGC 4512 & $2516 \pm 1 $ & $2.72$ & $-20.75$ & $10.60$\\
	$2661$ & $10\, 36\, 38.44$ & $14\, 10\, 15.97$ & NGC 3300 & $3017 \pm 1 $ & $2.54$ & $-21.02$ & $10.53$\\
	$2675$ & $12\, 08\, 09.62$ & $10\, 22\, 43.96$ & NGC 4119 & $1651 \pm 2 $ & $2.28$ & $-19.74$ & $10.05$\\
	$2682$ & $12\, 27\, 13.34$ & $12\, 44\, 05.22$ & NGC 4425 & $1891 \pm 1 $ & $2.39$ & $-20.42$ & $10.22$\\
	$2688$ & $12\, 24\, 05.01$ & $11\, 13\, 05.04$ & NGC 4352 & $2083 \pm 1 $ & $2.36$ & $-20.12$ & $10.08$\\
	$2710$ & $12\, 27\, 02.54$ & $15\, 27\, 41.34$ & NGC 4421 & $1551 \pm 1 $ & $2.58$ & $-20.15$ & $10.04$\\
	$2715$ & $14\, 05\, 12.42$ & $55\, 44\, 30.67$ & NGC 5475 & $1647 \pm 1 $ & $2.54$ & $-19.58$ & $9.98$\\
	$2731$ & $12\, 37\, 48.38$ & $05\, 22\, 06.69$ & NGC 4580 & $1035 \pm 2 $ & $2.37$ & $-19.23$ & $9.75$\\
	$2742$ & $12\, 15\, 59.87$ & $66\, 13\, 51.00$ & NGC 4221 & $1314 \pm 1 $ & $2.51$ & $-19.48$ & $9.83$\\
	$2743$ & $10\, 12\, 41.25$ & $03\, 07\, 45.79$ & NGC 3156 & $1266 \pm 29 $ & $1.99$ & $-19.14$ & $9.42$\\
	$2744$ & $11\, 06\, 32.10$ & $11\, 23\, 07.51$ & NGC 3524 & $1357 \pm 1 $ & $2.36$ & $-19.08$ & $9.71$\\
	$2756$ & $11\, 08\, 40.38$ & $57\, 13\, 48.71$ & NGC 3530 & $1876 \pm 1 $ & $2.42$ & $-18.95$ & $9.69$\\
	$2769$ & $12\, 25\, 18.78$ & $64\, 56\, 00.52$ & NGC 4391 & $1320 \pm 1 $ & $2.52$ & $-18.73$ & $9.58$\\
	$2770$ & $13\, 00\, 10.57$ & $12\, 28\, 59.92$ & NGC 4880 & $1362 \pm 3 $ & $2.24$ & $-19.29$ & $9.51$\\
	$2775$ & $12\, 22\, 04.11$ & $12\, 47\, 14.95$ & NGC 4306 & $1520 \pm 3 $ & $2.21$ & $-18.70$ & $9.35$\\
	$2789$ & $11\, 21\, 24.99$ & $03\, 00\, 50.23$ & NGC 3643 & $1742 \pm 2 $ & $2.28$ & $-18.67$ & $9.53$\\
	$2790$ & $12\, 38\, 17.87$ & $13\, 06\, 35.64$ & NGC 4584 & $1715 \pm 3 $ & $2.01$ & $-18.96$ & $9.46$\\
	$2795$ & $12\, 41\, 59.35$ & $12\, 56\, 34.27$ & NGC 4620 & $1125 \pm 3 $ & $2.09$ & $-18.63$ & $9.24$\\
	$2798$ & $15\, 06\, 35.03$ & $02\, 00\, 18.38$ & NGC 5841 & $1256 \pm 1 $ & $2.34$ & $-18.19$ & $9.13$\\
	$2805$ & $12\, 48\, 55.36$ & $14\, 54\, 28.40$ & IC 3806 & $1401 \pm 5 $ & $2.14$ & $-18.21$ & $9.31$\\
	$2831$ & $12\, 32\, 14.21$ & $10\, 15\, 05.18$ & IC 3468 & $1300 \pm 4 $ & $2.18$ & $-18.52$ & $9.15$\\
	$2890$ & $12\, 11\, 07.76$ & $14\, 16\, 29.33$ & IC 3032 & $1184 \pm 5 $ & $2.02$ & $-16.83$ & $8.55$\\
	$2891$ & $13\, 55\, 38.75$ & $04\, 59\, 06.18$ & NGC 5360 & $1180 \pm 3 $ & $1.72$ & $-16.84$ & $8.32$\\
	$2899$ & $12\, 17\, 01.11$ & $09\, 24\, 27.19$ & IC 3097 & $1253 \pm 7 $ & $1.94$ & $-16.88$ & $8.63$\\
	$2906$ & $12\, 16\, 52.36$ & $14\, 30\, 52.50$ & IC 3096 & $1264 \pm 3 $ & $1.84$ & $-17.03$ & $8.57$\\
	$2910$ & $12\, 10\, 12.57$ & $64\, 45\, 38.33$ & MCG +11-15-032 & $1349 \pm 5 $ & $1.89$ & $-16.76$ & $8.44$\\
	$2914$ & $12\, 33\, 13.43$ & $09\, 23\, 50.50$ & IC 3487 & $1074 \pm 4 $ & $1.78$ & $-16.45$ & $8.34$\\
	$2915$ & $12\, 16\, 09.06$ & $12\, 41\, 28.68$ & IC 3081 & $1103 \pm 4 $ & $2.01$ & $-16.34$ & $8.50$\\
	$2961$ & $12\, 32\, 39.01$ & $10\, 05\, 31.46$ & VCC 1446 & $1196 \pm 13 $ & $2.00$ & $-15.83$ & $8.19$\\
	$2962$ & $12\, 12\, 18.99$ & $15\, 28\, 59.14$ & VCC 0050 & $1209 \pm 12 $ & $1.85$ & $-15.87$ & $8.13$\\
	$2979$ & $12\, 16\, 02.22$ & $46\, 43\, 58.32$ & MCG +08-22-086 & $1061 \pm 7 $ & $1.96$ & $-15.62$ & $8.04$\\
	$2984$ & $12\, 52\, 33.75$ & $-01\, 43\, 48.75$ & ASK 14845 & $1129 \pm 3 $ & $1.74$ & $-15.77$ & $8.04$\\
	$2985$ & $12\, 22\, 50.85$ & $13\, 35\, 34.31$ & VCC 0592 & $1102 \pm 8 $ & $2.09$ & $-15.43$ & $8.08$\\
	$2996$ & $12\, 24\, 05.26$ & $10\, 04\, 03.89$ & PGC 40315 & $1370 \pm 29 $ & $2.15$ & $-16.05$ & $8.13$\\
	$3306$ & $23\, 20\, 28.21$ & $15\, 04\, 20.91$ & 2MASX J23202822+1504211 & $3828 \pm 2 $ & $2.30$ & $-18.77$ & $9.57$\\
	$3346$ & $00\, 25\, 52.49$ & $-09\, 39\, 42.37$ & 2MASXJ00255209-0939420 & $5201 \pm 2 $ & $2.65$ & $-20.78$ & $10.54$\\
	$3348$ & $00\, 12\, 06.10$ & $00\, 24\, 54.76$ & IC 0003 & $5447 \pm 2 $ & $2.63$ & $-21.14$ & $10.61$\\
	$3371$ & $03\, 34\, 17.75$ & $-06\, 15\, 53.99$ & NGC 1361 & $5254 \pm 2 $ & $2.60$ & $-21.44$ & $10.73$\\
	$3381$ & $07\, 36\, 16.80$ & $33\, 07\, 21.76$ & IC 2201 & $4694 \pm 1 $ & $2.79$ & $-20.54$ & $10.59$\\
	$3387$ & $08\, 25\, 17.47$ & $03\, 56\, 00.90$ & CGCG 032-022 & $4169 \pm 2 $ & $2.45$ & $-20.26$ & $10.19$\\
	$3388$ & $04\, 06\, 14.72$ & $-05\, 39\, 06.84$ & IC 2031 & $4823 \pm 3 $ & $1.68$ & $-20.01$ & $10.05$\\
	$3406$ & $00\, 04\, 35.22$ & $00\, 50\, 54.98$ & 2MASX J00043518+0050549 & $6392 \pm 4 $ & $2.17$ & $-18.54$ & $9.57$\\
	$3407$ & $00\, 09\, 40.24$ & $-10\, 25\, 02.71$ & 2MASX J00094023-1025027 & $5415 \pm 2 $ & $1.46$ & $-18.43$ & $9.12$\\
	$3411$ & $00\, 13\, 45.42$ & $-09\, 56\, 03.67$ & ASK 126038 & $3822 \pm 2 $ & $1.38$ & $-16.79$ & $8.24$\\
	$3423$ & $00\, 51\, 49.41$ & $00\, 33\, 53.22$ & UM 283 & $4629 \pm 0 $ & $1.08$ & $-18.05$ & $8.53$\\
	$3434$ & $04\, 10\, 51.37$ & $-05\, 13\, 19.97$ & ASK 57849 & $4868 \pm 3 $ & $1.37$ & $-17.48$ & $8.39$\\
	$3439$ & $07\, 40\, 22.74$ & $23\, 16\, 29.95$ & UGC 03960 & $2255 \pm 2 $ & $2.31$ & $-19.36$ & $9.77$\\
	$3459$ & $08\, 47\, 21.99$ & $42\, 23\, 55.65$ & ASK 191682 & $2980 \pm 1 $ & $1.26$ & $-16.13$ & $8.03$\\
	$3461$ & $08\, 47\, 59.49$ & $19\, 02\, 56.44$ & PGC 1578852 & $3844 \pm 2 $ & $1.86$ & $-17.20$ & $8.50$\\
	$3478$ & $13\, 36\, 20.08$ & $38\, 06\, 53.60$ & ASK 508595 & $5157 \pm 2 $ & $1.40$ & $-17.37$ & $8.53$\\
	$3483$ & $13\, 39\, 03.16$ & $43\, 33\, 58.60$ & CGCG 218-031 & $2740 \pm 2 $ & $2.41$ & $-18.94$ & $9.71$\\
	$3491$ & $09\, 08\, 54.37$ & $01\, 25\, 57.21$ & CGCG 006-006 & $4918 \pm 3 $ & $1.68$ & $-19.00$ & $9.30$\\
	$3495$ & $14\, 13\, 21.79$ & $54\, 40\, 06.27$ & MCG +09-23-057 & $2059 \pm 8 $ & $1.70$ & $-16.58$ & $8.28$\\
	$3498$ & $14\, 19\, 29.09$ & $35\, 34\, 01.11$ & ASK 392553 & $3207 \pm 1 $ & $1.36$ & $-16.81$ & $8.39$\\
	$3506$ & $00\, 29\, 33.17$ & $-09\, 04\, 50.74$ & IC 0022 & $6049 \pm 2 $ & $2.53$ & $-21.22$ & $10.66$\\
	$3510$ & $00\, 15\, 00.08$ & $-11\, 08\, 03.79$ & ASK 125926 & $3351 \pm 2 $ & $1.27$ & $-16.03$ & $8.05$\\
	$3520$ & $13\, 52\, 53.20$ & $37\, 41\, 22.28$ & 2MASX J13525317+3741219 & $5317 \pm 2 $ & $2.55$ & $-20.18$ & $10.24$\\
	$3527$ & $13\, 56\, 55.58$ & $05\, 09\, 06.83$ & CGCG 046-013 & $1517 \pm 10 $ & $2.11$ & $-16.85$ & $8.60$\\
	$3542$ & $08\, 19\, 24.29$ & $21\, 00\, 12.82$ & 2MASX J08192430+2100125 & $3906 \pm 4 $ & $2.54$ & $-18.79$ & $9.67$\\
	$3546$ & $07\, 45\, 01.45$ & $43\, 55\, 52.36$ & 2MASX J07450145+4355525 & $3736 \pm 1 $ & $1.30$ & $-17.01$ & $8.43$\\
	$3556$ & $08\, 51\, 56.67$ & $16\, 56\, 41.32$ & UGC 04639 & $8549 \pm 2 $ & $2.70$ & $-22.44$ & $11.18$\\
	$3565$ & $09\, 14\, 13.07$ & $43\, 08\, 05.97$ & KUG 0910+433 & $4232 \pm 2 $ & $1.90$ & $-20.15$ & $10.09$\\
	$3572$ & $03\, 30\, 17.18$ & $00\, 55\, 12.71$ & CGCG 390-096 & $6412 \pm 2 $ & $2.75$ & $-21.50$ & $10.87$\\
	$3581$ & $03\, 37\, 10.37$ & $-05\, 35\, 05.09$ & 2MASX J03371039-0535055 & $8347 \pm 2 $ & $2.61$ & $-21.77$ & $10.90$\\
	$3622$ & $22\, 51\, 43.16$ & $00\, 24\, 54.98$ & 2MASX J22514319+0024547 & $7807 \pm 2 $ & $2.84$ & $-21.33$ & $10.84$\\
	$3650$ & $01\, 29\, 43.99$ & $-01\, 14\, 29.10$ & UGC 01072 & $5190 \pm 2 $ & $2.59$ & $-21.23$ & $10.61$\\
	$3654$ & $03\, 58\, 19.35$ & $-04\, 43\, 49.56$ & ASK 57478 & $5294 \pm 2 $ & $1.60$ & $-18.21$ & $8.93$\\
	$3663$ & $07\, 29\, 45.06$ & $43\, 44\, 45.15$ & ASK 476339 & $3183 \pm 4 $ & $1.65$ & $-15.76$ & $8.10$\\
	$3665$ & $07\, 22\, 46.74$ & $41\, 39\, 29.65$ & UGC 03818 & $7002 \pm 2 $ & $2.44$ & $-21.19$ & $10.67$\\
	$3666$ & $07\, 26\, 35.39$ & $43\, 17\, 46.85$ & UGC 03844 & $3130 \pm 2 $ & $2.70$ & $-20.57$ & $10.42$\\
	$3668$ & $07\, 24\, 33.15$ & $41\, 57\, 02.18$ & 2MASX J07243311+4157021 & $7960 \pm 3 $ & $2.30$ & $-19.49$ & $9.96$\\
	$3669$ & $07\, 24\, 19.58$ & $38\, 45\, 38.73$ & 2MASX J07241961+3845387 & $7244 \pm 2 $ & $2.46$ & $-19.19$ & $9.80$\\
	$3670$ & $07\, 21\, 00.79$ & $41\, 03\, 06.58$ & 2MASX J07210079+4103065 & $6903 \pm 2 $ & $1.43$ & $-18.69$ & $9.22$\\
	$3673$ & $07\, 27\, 28.08$ & $43\, 27\, 50.08$ & ASK 476000 & $6623 \pm 1 $ & $1.13$ & $-17.60$ & $8.70$\\
	$3691$ & $12\, 28\, 08.61$ & $12\, 05\, 35.85$ & IC 0794 & $1921 \pm 3 $ & $2.37$ & $-19.16$ & $9.64$\\
	$3698$ & $01\, 26\, 42.25$ & $-01\, 05\, 16.00$ & ASK 32676 & $4370 \pm 8 $ & $2.29$ & $-17.32$ & $9.19$\\
	$3706$ & $03\, 11\, 17.74$ & $-08\, 04\, 48.04$ & 2MASX J03111772-0804486 & $3978 \pm 1 $ & $1.26$ & $-17.96$ & $8.75$\\
	$3710$ & $14\, 01\, 57.67$ & $46\, 18\, 42.90$ & NGC 5439 & $1895 \pm 4 $ & $2.02$ & $-18.59$ & $9.42$\\
	$3711$ & $14\, 29\, 14.46$ & $44\, 41\, 56.37$ & CGCG 247-032 & $2409 \pm 2 $ & $2.48$ & $-18.94$ & $9.71$\\
	$3716$ & $11\, 52\, 24.07$ & $32\, 24\, 13.96$ & NGC 3935 & $3066 \pm 2 $ & $2.19$ & $-20.30$ & $10.22$\\
	$3721$ & $07\, 21\, 23.42$ & $41\, 41\, 59.03$ & ASK 475472 & $7001 \pm 2 $ & $1.05$ & $-17.45$ & $8.48$\\
	$3735$ & $00\, 19\, 47.33$ & $00\, 35\, 26.86$ & 2MASXJ00194732+0035273 & $5306 \pm 3 $ & $1.94$ & $-19.65$ & $9.75$\\
	$3762$ & $00\, 39\, 55.98$ & $-08\, 51\, 11.54$ & ASK 127226 & $4122 \pm 1 $ & $1.18$ & $-16.61$ & $8.26$\\
	$3779$ & $01\, 28\, 59.57$ & $00\, 33\, 42.93$ & UGC 01062 & $5464 \pm 2 $ & $2.60$ & $-21.76$ & $10.85$\\
	$3783$ & $01\, 13\, 41.83$ & $00\, 06\, 09.76$ & UGC 00771 & $5152 \pm 2 $ & $2.55$ & $-20.84$ & $10.54$\\
	$3784$ & $01\, 15\, 54.29$ & $13\, 21\, 12.05$ & CGCG 436-016 & $4184 \pm 2 $ & $2.59$ & $-20.14$ & $10.24$\\
	$3795$ & $00\, 25\, 17.31$ & $14\, 34\, 40.89$ & ASK 147884 & $5224 \pm 1 $ & $1.06$ & $-16.86$ & $8.11$\\
	$3801$ & $01\, 03\, 01.72$ & $-01\, 06\, 39.54$ & CGCG 384-061 & $5237 \pm 2 $ & $2.51$ & $-20.12$ & $10.21$\\
	$3805$ & $01\, 22\, 46.01$ & $00\, 25\, 35.09$ & 2MASX J01224599-0025343 & $5182 \pm 3 $ & $2.22$ & $-18.95$ & $9.61$\\
	$3808$ & $01\, 15\, 22.22$ & $00\, 09\, 30.44$ & 2MASX J01152220-0009299 & $5196 \pm 4 $ & $2.32$ & $-18.15$ & $9.30$\\
	$3813$ & $01\, 04\, 25.32$ & $-09\, 22\, 59.33$ & PGC 991736 & $4653 \pm 1 $ & $1.41$ & $-17.36$ & $8.51$\\
	$3832$ & $01\, 38\, 47.38$ & $01\, 04\, 18.45$ & UGC 01169 & $4964 \pm 2 $ & $3.14$ & $-20.34$ & $10.58$\\
	$3841$ & $01\, 48\, 53.13$ & $13\, 25\, 26.20$ & 2MASXi J0148531+132526 & $4659 \pm 2 $ & $2.17$ & $-18.29$ & $9.41$\\
	$3842$ & $01\, 49\, 53.83$ & $12\, 58\, 33.74$ & 2MASX J01495381+1258340 & $4691 \pm 6 $ & $2.48$ & $-18.14$ & $9.35$\\
	$3846$ & $01\, 55\, 16.26$ & $-08\, 51\, 15.39$ & KUG 0152-090 & $3950 \pm 2 $ & $1.56$ & $-17.30$ & $8.60$\\
	$3848$ & $01\, 55\, 59.75$ & $00\, 11\, 08.04$ & PGC 3111971 & $3637 \pm 1 $ & $1.16$ & $-17.01$ & $8.19$\\
	$3906$ & $02\, 31\, 41.35$ & $-09\, 18\, 01.60$ & NGC 0960 & $4867 \pm 1 $ & $2.81$ & $-20.85$ & $10.71$\\
	$3946$ & $03\, 20\, 40.80$ & $-07\, 23\, 39.89$ & NGC 1303 & $5461 \pm 1 $ & $2.41$ & $-21.33$ & $10.59$\\
	$3947$ & $03\, 17\, 48.53$ & $-07\, 37\, 00.65$ & NGC 1286 & $4312 \pm 1 $ & $2.51$ & $-20.80$ & $10.45$\\
	$3951$ & $03\, 17\, 06.67$ & $-06\, 30\, 07.76$ & 2MASX J03170667-0630082 & $4008 \pm 4 $ & $2.06$ & $-19.74$ & $9.91$\\
	$3956$ & $03\, 15\, 38.62$ & $-07\, 04\, 43.75$ & KUG 0313-072 & $3947 \pm 1 $ & $1.58$ & $-18.83$ & $9.24$\\
	$3986$ & $03\, 39\, 07.13$ & $-06\, 27\, 02.88$ & 2MASX J03390711-0627028 & $5381 \pm 4 $ & $2.16$ & $-20.03$ & $10.08$\\
	$3997$ & $03\, 38\, 04.15$ & $-05\, 21\, 09.07$ & ASK 56542 & $4019 \pm 1 $ & $1.48$ & $-17.25$ & $8.56$\\
	$4020$ & $04\, 12\, 11.55$ & $-04\, 52\, 27.14$ & ASK 57882 & $9047 \pm 4 $ & $1.39$ & $-18.88$ & $9.19$\\
	$4026$ & $04\, 01\, 33.54$ & $-06\, 20\, 12.46$ & PGC 1034032 & $5722 \pm 1 $ & $1.50$ & $-17.56$ & $8.77$\\
	$4030$ & $07\, 27\, 19.37$ & $44\, 25\, 38.37$ & 2MASX J07271936+4425388 & $9742 \pm 2 $ & $2.58$ & $-20.87$ & $10.89$\\
	$4031$ & $07\, 26\, 24.68$ & $43\, 02\, 54.78$ & ASK 475844 & $7583 \pm 2 $ & $1.70$ & $-18.64$ & $9.30$\\
	$4032$ & $07\, 26\, 20.04$ & $42\, 02\, 46.22$ & ASK 475860 & $7994 \pm 4 $ & $1.82$ & $-18.98$ & $9.21$\\
	$4033$ & $07\, 20\, 02.10$ & $41\, 08\, 11.21$ & ASK 475444 & $7026 \pm 4 $ & $1.50$ & $-17.37$ & $8.53$\\
	$4060$ & $07\, 41\, 54.78$ & $38\, 29\, 53.74$ & 2MASX J07415484+3829537 & $3507 \pm 1 $ & $1.06$ & $-17.27$ & $8.31$\\
	$4061$ & $07\, 44\, 05.51$ & $46\, 42\, 34.21$ & ASK 476552 & $3105 \pm 1 $ & $1.15$ & $-16.46$ & $8.00$\\
	$4088$ & $08\, 17\, 35.00$ & $20\, 54\, 11.06$ & NGC 2553 & $4670 \pm 1 $ & $2.61$ & $-21.18$ & $10.64$\\
	$4093$ & $08\, 18\, 08.76$ & $23\, 02\, 51.31$ & IC 2269 & $3980 \pm 2 $ & $3.01$ & $-19.38$ & $10.18$\\
	$4094$ & $08\, 19\, 32.11$ & $21\, 23\, 39.50$ & IC 2293 & $4090 \pm 3 $ & $1.89$ & $-20.00$ & $9.98$\\
	$4101$ & $08\, 05\, 47.84$ & $30\, 13\, 52.35$ & CGCG 148-111 & $2306 \pm 3 $ & $1.71$ & $-17.62$ & $9.17$\\
	$4106$ & $08\, 17\, 15.93$ & $24\, 53\, 56.81$ & 2MASXJ08171594+2453569 & $1898 \pm 7 $ & $2.17$ & $-16.08$ & $8.42$\\
	$4109$ & $08\, 23\, 24.07$ & $22\, 16\, 00.45$ & ASK 484591 & $2055 \pm 13 $ & $2.46$ & $-16.06$ & $8.31$\\
	$4110$ & $08\, 26\, 28.81$ & $26\, 04\, 29.10$ & ASK 364075 & $1968 \pm 17 $ & $2.05$ & $-15.75$ & $8.16$\\
	$4129$ & $08\, 37\, 26.59$ & $40\, 02\, 08.11$ & UGC 04498 & $7091 \pm 2 $ & $2.48$ & $-21.61$ & $10.81$\\
	$4151$ & $08\, 33\, 12.72$ & $39\, 30\, 49.82$ & ASK 191177 & $2026 \pm 1 $ & $1.27$ & $-16.29$ & $8.00$\\
	$4170$ & $09\, 14\, 34.33$ & $30\, 08\, 27.06$ & UGC 04869 & $6852 \pm 2 $ & $2.81$ & $-22.16$ & $11.17$\\
	$4175$ & $09\, 10\, 11.89$ & $50\, 24\, 04.75$ & NGC 2767 & $4925 \pm 2 $ & $2.79$ & $-20.98$ & $10.71$\\
	$4177$ & $09\, 01\, 28.62$ & $03\, 43\, 14.13$ & NGC 2729 & $3819 \pm 1 $ & $2.71$ & $-20.61$ & $10.44$\\
	$4184$ & $09\, 12\, 44.37$ & $34\, 55\, 32.04$ & NGC 2780 & $1954 \pm 2 $ & $1.91$ & $-18.84$ & $9.58$\\
	$4197$ & $09\, 14\, 48.80$ & $33\, 01\, 15.30$ & 2MASX J09144880+3301148 & $1819 \pm 2 $ & $1.26$ & $-16.59$ & $8.12$\\
	$4214$ & $09\, 39\, 34.69$ & $48\, 25\, 18.56$ & UGC 05145 & $7378 \pm 3 $ & $2.62$ & $-21.97$ & $11.21$\\
	$4222$ & $09\, 57\, 35.59$ & $45\, 13\, 47.69$ & UGC 05345 & $3696 \pm 2 $ & $2.53$ & $-20.18$ & $10.30$\\
	$4224$ & $09\, 46\, 48.95$ & $09\, 44\, 10.08$ & CGCG 063-066 & $2997 \pm 2 $ & $2.41$ & $-19.66$ & $9.95$\\
	$4225$ & $09\, 38\, 34.45$ & $08\, 53\, 16.44$ & 2MASX J09383447+0853159 & $3228 \pm 2 $ & $2.38$ & $-19.46$ & $9.95$\\
	$4229$ & $09\, 35\, 05.80$ & $09\, 38\, 57.22$ & 2MASX J09350578+0938566 & $3408 \pm 2 $ & $2.32$ & $-18.81$ & $9.61$\\
	$4231$ & $09\, 48\, 41.60$ & $59\, 15\, 39.59$ & 2MASX J09484156+5915394 & $2231 \pm 2 $ & $1.84$ & $-18.19$ & $9.31$\\
	$4271$ & $10\, 20\, 43.35$ & $65\, 10\, 19.61$ & UGC 05576 & $3288 \pm 2 $ & $2.43$ & $-20.14$ & $10.14$\\
	$4274$ & $10\, 12\, 48.57$ & $43\, 08\, 43.91$ & IC 0598 & $2245 \pm 1 $ & $2.26$ & $-19.76$ & $9.92$\\
	$4309$ & $10\, 37\, 37.91$ & $37\, 27\, 20.30$ & NGC 3304 & $6937 \pm 2 $ & $2.71$ & $-21.97$ & $11.11$\\
	$4316$ & $10\, 58\, 37.57$ & $09\, 03\, 01.62$ & UGC 06062 & $2623 \pm 2 $ & $2.59$ & $-19.98$ & $10.18$\\
	$4319$ & $10\, 35\, 04.85$ & $46\, 33\, 41.23$ & UGC 05744 & $3356 \pm 3 $ & $1.58$ & $-19.85$ & $9.66$\\
	$4374$ & $11\, 24\, 06.48$ & $38\, 51\, 23.09$ & 2MASX J11240641+3851226 & $1979 \pm 3 $ & $2.45$ & $-17.29$ & $9.03$\\
	$4407$ & $11\, 51\, 28.06$ & $35\, 26\, 03.72$ & UGC 06827 & $3095 \pm 2 $ & $2.47$ & $-20.18$ & $10.13$\\
	$4414$ & $11\, 51\, 13.43$ & $50\, 09\, 24.84$ & NGC 3922 & $930 \pm 3 $ & $2.21$ & $-18.20$ & $9.25$\\
	$4448$ & $12\, 05\, 59.46$ & $02\, 29\, 53.63$ & CGCG 041-039 & $6098 \pm 2 $ & $2.68$ & $-21.29$ & $10.96$\\
	$4458$ & $12\, 12\, 11.80$ & $13\, 14\, 47.46$ & NGC 4165 & $1868 \pm 4 $ & $2.07$ & $-18.87$ & $9.49$\\
	$4459$ & $12\, 11\, 02.73$ & $12\, 06\, 14.40$ & IC 0767 & $1877 \pm 2 $ & $2.05$ & $-18.82$ & $9.41$\\
	$4462$ & $12\, 08\, 55.08$ & $41\, 44\, 27.12$ & UGC 07129 & $925 \pm 2 $ & $1.85$ & $-17.43$ & $8.97$\\
	$4465$ & $12\, 22\, 19.53$ & $14\, 45\, 38.81$ & UGC 07436 & $982 \pm 4 $ & $2.29$ & $-17.13$ & $8.76$\\
	$4514$ & $12\, 51\, 41.53$ & $13\, 05\, 41.88$ & CGCG 071-059 & $1487 \pm 5 $ & $1.72$ & $-16.48$ & $8.30$\\
	$4516$ & $12\, 41\, 39.41$ & $12\, 14\, 50.61$ & IC 3663 & $927 \pm 10 $ & $1.99$ & $-15.90$ & $8.11$\\
	$4541$ & $13\, 08\, 42.15$ & $52\, 01\, 00.69$ & CGCG 271-017 & $4705 \pm 2 $ & $2.62$ & $-20.96$ & $10.63$\\
	$4542$ & $13\, 14\, 46.04$ & $53\, 49\, 13.27$ & CGCG 271-026 & $4711 \pm 2 $ & $2.61$ & $-20.77$ & $10.53$\\
	$4546$ & $13\, 17\, 07.56$ & $57\, 32\, 22.17$ & IC 0875 & $2760 \pm 2 $ & $2.40$ & $-20.10$ & $10.01$\\
	$4595$ & $13\, 56\, 58.06$ & $45\, 58\, 23.61$ & UGC 08876 & $2059 \pm 1 $ & $2.56$ & $-19.28$ & $9.88$\\
	$4598$ & $13\, 48\, 56.27$ & $59\, 50\, 08.64$ & UGC 08741 & $2019 \pm 6 $ & $2.00$ & $-18.70$ & $9.44$\\
	$4609$ & $13\, 53\, 19.84$ & $05\, 46\, 17.93$ & UGC 08799 & $1046 \pm 16 $ & $2.14$ & $-15.71$ & $8.26$\\
	$4634$ & $14\, 03\, 47.16$ & $35\, 44\, 30.04$ & UGC 08984 & $3805 \pm 1 $ & $2.58$ & $-20.61$ & $10.42$\\
	$4640$ & $14\, 07\, 39.28$ & $54\, 47\, 40.60$ & CGCG 272-032 & $2315 \pm 1 $ & $2.33$ & $-19.11$ & $9.68$\\
	$4644$ & $14\, 09\, 54.94$ & $56\, 49\, 21.36$ & CGCG 295-037 & $1790 \pm 4 $ & $2.17$ & $-17.85$ & $9.18$\\
	$4648$ & $14\, 04\, 42.99$ & $55\, 26\, 06.72$ & 2MASX J14044299+5526064 & $1537 \pm 2 $ & $1.86$ & $-16.96$ & $8.63$\\
	$4668$ & $14\, 57\, 11.25$ & $52\, 20\, 45.82$ & UGC 09629 & $7822 \pm 2 $ & $2.78$ & $-21.82$ & $11.05$\\
	$4680$ & $14\, 58\, 48.72$ & $02\, 01\, 24.62$ & CGCG 020-039 & $1804 \pm 1 $ & $2.31$ & $-18.60$ & $9.50$\\
	$4687$ & $14\, 48\, 58.97$ & $33\, 11\, 34.95$ & CGCG 193-002 & $1700 \pm 2 $ & $1.45$ & $-16.89$ & $8.33$\\
	$4696$ & $14\, 54\, 19.38$ & $38\, 48\, 29.91$ & CGCG 221-008 & $8685 \pm 3 $ & $2.75$ & $-21.76$ & $11.03$\\
	$4698$ & $14\, 31\, 49.74$ & $27\, 53\, 30.30$ & PGC 4553986 & $4415 \pm 4 $ & $1.76$ & $-16.91$ & $8.32$\\
	$4720$ & $15\, 11\, 48.38$ & $46\, 15\, 13.90$ & CGCG 249-011 & $5454 \pm 2 $ & $2.20$ & $-20.41$ & $10.31$\\
	$4728$ & $15\, 13\, 29.18$ & $58\, 30\, 33.56$ & Mrk 0847 & $2543 \pm 3 $ & $1.60$ & $-18.96$ & $9.41$\\
	$4732$ & $15\, 00\, 16.58$ & $02\, 18\, 02.57$ & CGCG 020-042 & $1818 \pm 3 $ & $1.98$ & $-17.72$ & $9.09$\\
	$4734$ & $15\, 01\, 03.11$ & $00\, 42\, 27.44$ & Mrk 1390 & $1724 \pm 3 $ & $1.77$ & $-17.08$ & $8.75$\\
	$4736$ & $15\, 12\, 31.74$ & $00\, 48\, 45.30$ & PGC 1176138 & $1844 \pm 4 $ & $1.67$ & $-16.76$ & $8.53$\\
	$4806$ & $16\, 02\, 16.34$ & $49\, 12\, 11.42$ & UGC 10150 & $6135 \pm 6 $ & $2.12$ & $-20.36$ & $10.16$\\
	$4808$ & $16\, 02\, 11.63$ & $07\, 05\, 09.97$ & CGCG 051-021 & $2654 \pm 2 $ & $2.24$ & $-19.45$ & $9.98$\\
	$4838$ & $16\, 58\, 50.69$ & $40\, 07\, 16.18$ & CGCG 225-021 & $8658 \pm 2 $ & $2.73$ & $-22.04$ & $11.06$\\
	$4846$ & $16\, 41\, 06.57$ & $46\, 00\, 14.63$ & IC 1226 & $5312 \pm 4 $ & $2.35$ & $-20.32$ & $10.26$\\
	$4855$ & $16\, 35\, 20.71$ & $17\, 45\, 55.19$ & Mrk 0886 & $2740 \pm 1 $ & $1.12$ & $-18.21$ & $8.94$\\
	$4861$ & $16\, 34\, 39.88$ & $46\, 57\, 37.26$ & 2MASXi J1634398+465736 & $2452 \pm 1 $ & $1.24$ & $-16.74$ & $8.26$\\
	$4898$ & $17\, 01\, 12.98$ & $60\, 15\, 05.25$ & Ark 514 & $3743 \pm 2 $ & $1.47$ & $-18.70$ & $9.02$\\
	$4908$ & $17\, 01\, 29.63$ & $22\, 43\, 52.46$ & ASK 406590 & $2820 \pm 1 $ & $2.22$ & $-15.79$ & $8.11$\\
	$4960$ & $20\, 54\, 12.19$ & $-05\, 11\, 31.60$ & 2MASX J20541219-0511314 & $6134 \pm 5 $ & $2.44$ & $-18.59$ & $9.63$\\
	$4989$ & $21\, 16\, 24.75$ & $10\, 16\, 24.07$ & CGCG 426-029 & $5175 \pm 2 $ & $2.29$ & $-20.22$ & $10.15$\\
	$4990$ & $21\, 04\, 51.97$ & $00\, 26\, 52.75$ & CGCG 374-042 & $4129 \pm 2 $ & $2.45$ & $-19.62$ & $9.95$\\
	$4997$ & $21\, 28\, 29.09$ & $10\, 04\, 52.52$ & 2MASX J21282910+1004527 & $4929 \pm 2 $ & $2.03$ & $-18.16$ & $9.10$\\
	$4999$ & $21\, 13\, 07.73$ & $01\, 13\, 47.13$ & 2MASX J21130776+0113480 & $4157 \pm 2 $ & $1.30$ & $-18.41$ & $8.97$\\
	$5004$ & $21\, 18\, 06.61$ & $-07\, 42\, 56.84$ & 2MASX J21180656-0742566 & $2516 \pm 2 $ & $1.41$ & $-16.62$ & $8.17$\\
	$5015$ & $21\, 31\, 37.56$ & $11\, 49\, 53.90$ & CGCG 426-062 & $8643 \pm 3 $ & $2.92$ & $-21.99$ & $11.15$\\
	$5020$ & $21\, 50\, 38.41$ & $13\, 17\, 17.48$ & CGCG 427-027 & $6045 \pm 2 $ & $2.59$ & $-21.61$ & $10.88$\\
	$5025$ & $21\, 50\, 27.56$ & $12\, 38\, 10.37$ & 2MASX J21502753+1238103 & $6507 \pm 2 $ & $2.48$ & $-19.53$ & $9.98$\\
	$5040$ & $21\, 52\, 22.47$ & $-01\, 10\, 15.96$ & ASK 21400 & $4770 \pm 1 $ & $1.15$ & $-16.83$ & $8.14$\\
	$5048$ & $22\, 01\, 41.64$ & $11\, 51\, 24.41$ & CGCG 428-014 & $8944 \pm 3 $ & $3.13$ & $-21.95$ & $11.33$\\
	$5061$ & $22\, 24\, 44.13$ & $12\, 21\, 40.68$ & 2MASX J22244417+1221410 & $5127 \pm 3 $ & $2.09$ & $-19.23$ & $9.80$\\
	$5063$ & $22\, 20\, 19.83$ & $-08\, 46\, 17.13$ & 2MASXi J2220198-084617 & $7288 \pm 1 $ & $1.11$ & $-18.81$ & $8.97$\\
	$5070$ & $22\, 04\, 08.80$ & $00\, 55\, 31.78$ & ASK 22153 & $4825 \pm 16 $ & $2.28$ & $-17.21$ & $8.66$\\
	$5096$ & $22\, 40\, 17.46$ & $14\, 29\, 56.90$ & 2MASX J22401742+1429556 & $6384 \pm 1 $ & $1.20$ & $-18.96$ & $9.20$\\
	$5105$ & $22\, 33\, 49.80$ & $00\, 28\, 58.47$ & ASK 23755 & $4642 \pm 1 $ & $1.09$ & $-17.02$ & $8.22$\\
	$5117$ & $23\, 18\, 08.39$ & $00\, 23\, 25.63$ & CGCG 380-023 & $8775 \pm 2 $ & $2.71$ & $-22.40$ & $11.17$\\
	$5118$ & $23\, 20\, 29.08$ & $-01\, 00\, 08.81$ & CGCG 380-035 & $9370 \pm 2 $ & $2.75$ & $-22.03$ & $11.08$\\
	$5120$ & $23\, 23\, 27.04$ & $14\, 19\, 33.09$ & CGCG 431-053 & $7651 \pm 2 $ & $2.78$ & $-21.40$ & $10.86$\\
	$5133$ & $23\, 04\, 04.16$ & $00\, 46\, 50.41$ & 2MASX J23040415+0046511 & $4903 \pm 3 $ & $1.80$ & $-18.56$ & $9.27$\\
	$5164$ & $23\, 33\, 27.02$ & $14\, 20\, 06.86$ & CGCG 432-002 & $5735 \pm 3 $ & $2.16$ & $-20.74$ & $10.37$\\
	$5165$ & $23\, 43\, 55.95$ & $00\, 13\, 05.01$ & CGCG 381-031 & $6627 \pm 1 $ & $2.48$ & $-20.28$ & $10.25$\\
	$5168$ & $23\, 36\, 34.41$ & $-09\, 31\, 32.06$ & PGC 989944 & $6845 \pm 4 $ & $1.86$ & $-19.87$ & $9.77$\\
	$5170$ & $23\, 56\, 11.28$ & $00\, 01\, 45.24$ & 2MASX J23561127-0001452 & $6739 \pm 4 $ & $2.52$ & $-19.07$ & $9.76$\\
	$5177$ & $23\, 38\, 26.05$ & $15\, 23\, 11.07$ & ASK 145449 & $3984 \pm 3 $ & $1.80$ & $-17.25$ & $8.78$\\
	$5195$ & $13\, 28\, 33.04$ & $32\, 04\, 09.73$ & NGC 5166B & $4838 \pm 3 $ & $2.40$ & $-19.96$ & $10.09$\\
	$5210$ & $23\, 47\, 03.79$ & $14\, 50\, 30.38$ & CGCG 432-030 & $6622 \pm 2 $ & $2.19$ & $-20.79$ & $10.39$\\
	$5215$ & $23\, 40\, 42.68$ & $-09\, 23\, 36.54$ & 2MASXi J2340427-092336 & $5160 \pm 2 $ & $1.25$ & $-18.71$ & $9.01$\\
	$5216$ & $23\, 51\, 14.64$ & $15\, 22\, 23.88$ & ASK 146293 & $5994 \pm 1 $ & $1.31$ & $-17.45$ & $8.55$\\
	$5217$ & $23\, 52\, 42.63$ & $-11\, 00\, 53.07$ & ASK 124704 & $5374 \pm 1 $ & $1.31$ & $-17.20$ & $8.38$\\
	$5226$ & $11\, 58\, 56.19$ & $31\, 25\, 10.84$ & ASK 527351 & $3021 \pm 4 $ & $1.45$ & $-17.20$ & $8.55$\\
	$5241$ & $12\, 10\, 32.83$ & $58\, 18\, 14.90$ & NGC 4149 & $3057 \pm 3 $ & $2.35$ & $-20.07$ & $10.37$\\
	$5252$ & $00\, 00\, 47.89$ & $14\, 16\, 39.17$ & 2MASX J00004789+1416390 & $10847 \pm 3 $ & $2.45$ & $-20.82$ & $10.71$\\
	$5256$ & $00\, 21\, 35.29$ & $01\, 09\, 56.33$ & CGCG 383-002 & $5465 \pm 1 $ & $2.45$ & $-20.01$ & $10.15$\\
	$5258$ & $00\, 15\, 05.37$ & $15\, 03\, 59.70$ & 2MASX J00150533+1503597 & $5428 \pm 2 $ & $2.13$ & $-19.86$ & $10.00$\\
	$5260$ & $00\, 10\, 25.49$ & $14\, 17\, 23.06$ & KUG 0007+140 & $5452 \pm 4 $ & $1.71$ & $-19.34$ & $9.50$\\
	$5268$ & $00\, 22\, 20.33$ & $15\, 56\, 30.30$ & ASK 148040 & $5213 \pm 2 $ & $1.34$ & $-17.74$ & $8.68$\\
	$5279$ & $00\, 31\, 36.55$ & $-10\, 53\, 17.43$ & 2MASXJ00313653-1053178 & $5075 \pm 2 $ & $2.56$ & $-20.52$ & $10.37$\\
	$5286$ & $00\, 40\, 26.90$ & $00\, 02\, 43.53$ & 2MASX J00402686-0002431 & $5847 \pm 2 $ & $1.68$ & $-19.11$ & $9.46$\\
	$5292$ & $00\, 53\, 19.64$ & $-10\, 24\, 11.85$ & 2MASX J00531961-1024115 & $4403 \pm 1 $ & $1.04$ & $-18.33$ & $8.80$\\
	$5296$ & $00\, 37\, 59.82$ & $00\, 42\, 35.95$ & ASK 29753 & $4167 \pm 1 $ & $1.44$ & $-16.69$ & $8.39$\\
	$5305$ & $01\, 12\, 57.42$ & $00\, 20\, 41.94$ & NGC 0429 & $5628 \pm 2 $ & $2.66$ & $-21.28$ & $10.76$\\
	$5309$ & $01\, 18\, 44.86$ & $00\, 54\, 22.80$ & CGCG 385-063 & $5251 \pm 3 $ & $2.52$ & $-20.08$ & $10.09$\\
	$5310$ & $01\, 26\, 25.91$ & $-08\, 33\, 51.12$ & 2MASXJ01262589-0833510 & $5336 \pm 1 $ & $2.35$ & $-20.50$ & $10.18$\\
	$5321$ & $01\, 26\, 49.69$ & $00\, 58\, 31.08$ & Mrk 0570 & $4853 \pm 3 $ & $1.68$ & $-19.27$ & $8.91$\\
	$5323$ & $01\, 13\, 02.84$ & $00\, 40\, 40.62$ & ASK 31963 & $4500 \pm 2 $ & $1.20$ & $-16.71$ & $8.59$\\
	$5326$ & $01\, 09\, 42.67$ & $00\, 57\, 13.29$ & ASK 31197 & $5203 \pm 3 $ & $1.48$ & $-16.83$ & $8.24$\\
	$5334$ & $01\, 40\, 53.63$ & $-10\, 16\, 41.56$ & 2MASXJ01405362-1016415 & $5296 \pm 1 $ & $2.57$ & $-20.75$ & $10.50$\\
	$5335$ & $01\, 31\, 04.76$ & $13\, 38\, 58.79$ & CGCG 436-067 & $5889 \pm 2 $ & $2.76$ & $-20.40$ & $10.49$\\
	$5337$ & $01\, 51\, 57.52$ & $-08\, 31\, 03.44$ & IC 0170 & $5192 \pm 2 $ & $2.49$ & $-20.45$ & $10.31$\\
	$5340$ & $01\, 42\, 30.89$ & $00\, 49\, 10.03$ & CGCG 386-032 & $5189 \pm 2 $ & $1.58$ & $-19.35$ & $9.43$\\
	$5344$ & $01\, 34\, 37.53$ & $-01\, 03\, 08.03$ & ASK 33113 & $4787 \pm 7 $ & $1.89$ & $-17.99$ & $9.25$\\
	$5353$ & $01\, 54\, 41.85$ & $00\, 36\, 41.71$ & PGC 1170628 & $4618 \pm 5 $ & $1.50$ & $-16.79$ & $8.24$\\
	$5369$ & $02\, 20\, 42.04$ & $-08\, 08\, 26.66$ & 2MASX J02204200-0808252 & $4710 \pm 3 $ & $1.77$ & $-18.94$ & $9.44$\\
	$5437$ & $03\, 02\, 35.01$ & $-07\, 21\, 45.38$ & ASK 55199 & $5986 \pm 3 $ & $1.21$ & $-16.96$ & $8.29$\\
	$5440$ & $03\, 02\, 11.39$ & $-01\, 09\, 59.60$ & ASK 37576 & $4079 \pm 2 $ & $1.40$ & $-16.36$ & $8.13$\\
	$5463$ & $03\, 35\, 34.54$ & $-05\, 44\, 30.75$ & ASK 56318 & $5398 \pm 1 $ & $1.18$ & $-17.48$ & $8.44$\\
	$5473$ & $04\, 06\, 44.26$ & $-04\, 26\, 50.54$ & 2MASX J04064426-0426510 & $11300 \pm 2 $ & $1.40$ & $-19.98$ & $9.69$\\
	$5481$ & $07\, 19\, 51.50$ & $41\, 24\, 58.04$ & 2MASX J07195149+4124585 & $10470 \pm 6 $ & $2.31$ & $-19.70$ & $10.05$\\
	$5483$ & $07\, 25\, 04.45$ & $40\, 35\, 37.61$ & ASK 475402 & $10200 \pm 1 $ & $0.96$ & $-18.91$ & $8.84$\\
	$5507$ & $07\, 35\, 24.17$ & $36\, 38\, 36.47$ & ASK 44962 & $3902 \pm 1 $ & $1.08$ & $-17.11$ & $8.23$\\
	$5508$ & $07\, 46\, 19.80$ & $39\, 51\, 26.07$ & ASK 45258 & $3895 \pm 2 $ & $1.56$ & $-17.09$ & $8.57$\\
	$5522$ & $08\, 03\, 28.94$ & $33\, 27\, 44.59$ & KUG 0800+336 & $11794 \pm 2 $ & $1.74$ & $-22.64$ & $11.17$\\
	$5525$ & $08\, 20\, 09.90$ & $27\, 05\, 36.51$ & UGC 04341 & $5869 \pm 2 $ & $2.64$ & $-21.54$ & $10.92$\\
	$5526$ & $08\, 26\, 18.06$ & $27\, 50\, 24.47$ & IC 2365 & $6019 \pm 1 $ & $2.55$ & $-21.66$ & $10.77$\\
	$5528$ & $08\, 19\, 51.89$ & $20\, 59\, 05.90$ & NGC 2560 & $4883 \pm 2 $ & $2.65$ & $-21.37$ & $10.78$\\
	$5536$ & $08\, 16\, 57.57$ & $20\, 30\, 44.19$ & CGCG 119-027 & $4334 \pm 4 $ & $1.81$ & $-19.39$ & $9.62$\\
	$5547$ & $08\, 22\, 15.81$ & $46\, 41\, 30.00$ & 2MASX J08221577+4641309 & $2179 \pm 1 $ & $1.41$ & $-16.36$ & $8.26$\\
	$5575$ & $08\, 58\, 30.48$ & $02\, 55\, 31.74$ & IC 2426 & $3887 \pm 1 $ & $2.34$ & $-19.75$ & $9.96$\\
	$5586$ & $08\, 34\, 20.18$ & $50\, 27\, 08.94$ & 2MASX J08342016+5027088 & $3433 \pm 2 $ & $1.61$ & $-17.13$ & $8.63$\\
	$5618$ & $09\, 00\, 58.50$ & $47\, 47\, 43.36$ & KUG 0857+479 & $3127 \pm 2 $ & $2.41$ & $-19.29$ & $9.99$\\
	$5656$ & $09\, 46\, 45.58$ & $09\, 15\, 51.71$ & CGCG 063-065 & $4030 \pm 2 $ & $2.53$ & $-19.34$ & $9.85$\\
	$5667$ & $09\, 52\, 35.11$ & $08\, 11\, 56.62$ & ASK 277328 & $2725 \pm 3 $ & $1.35$ & $-17.32$ & $8.53$\\
	$5668$ & $09\, 46\, 28.57$ & $00\, 26\, 03.56$ & ASK 51 & $1810 \pm 1 $ & $1.45$ & $-16.92$ & $8.34$\\
	$5689$ & $10\, 21\, 21.12$ & $24\, 20\, 29.04$ & UGC 05591 & $11118 \pm 2 $ & $2.71$ & $-22.33$ & $11.21$\\
	$5690$ & $10\, 22\, 06.03$ & $21\, 03\, 54.37$ & CGCG 124-015 & $11738 \pm 3 $ & $2.77$ & $-22.63$ & $11.33$\\
	$5694$ & $10\, 01\, 31.06$ & $37\, 12\, 14.20$ & IC 2530 & $6559 \pm 2 $ & $2.64$ & $-21.55$ & $10.76$\\
	$5696$ & $10\, 25\, 47.70$ & $26\, 34\, 14.63$ & CGCG 154-013 & $5023 \pm 2 $ & $2.56$ & $-21.12$ & $10.62$\\
	$5699$ & $10\, 00\, 45.21$ & $04\, 44\, 03.56$ & UGC 05383 & $3968 \pm 2 $ & $2.64$ & $-20.20$ & $10.33$\\
	$5701$ & $10\, 04\, 31.75$ & $60\, 06\, 28.71$ & NGC 3102 & $3038 \pm 2 $ & $2.44$ & $-20.01$ & $10.15$\\
	$5703$ & $10\, 02\, 00.95$ & $59\, 15\, 08.32$ & CGCG 289-027 & $2802 \pm 4 $ & $2.09$ & $-19.12$ & $9.60$\\
	$5715$ & $10\, 12\, 52.79$ & $22\, 43\, 19.22$ & CGCG 123-024 & $1281 \pm 3 $ & $1.51$ & $-16.49$ & $8.16$\\
	$5735$ & $10\, 47\, 26.58$ & $06\, 02\, 53.24$ & NGC 3376 & $5816 \pm 2 $ & $2.72$ & $-21.42$ & $10.76$\\
	$5743$ & $10\, 35\, 09.41$ & $25\, 02\, 17.11$ & CGCG 124-039 & $5244 \pm 2 $ & $2.29$ & $-20.00$ & $10.02$\\
	$5816$ & $11\, 38\, 36.24$ & $33\, 52\, 04.62$ & CGCG 186-015 & $10844 \pm 3 $ & $2.87$ & $-22.59$ & $11.37$\\
	$5821$ & $11\, 57\, 42.90$ & $57\, 33\, 57.00$ & UGC 06939 & $4915 \pm 2 $ & $2.56$ & $-21.20$ & $10.63$\\
	$5822$ & $11\, 39\, 03.33$ & $00\, 12\, 21.67$ & IC 0716 & $5413 \pm 2 $ & $2.59$ & $-20.79$ & $10.68$\\
	$5825$ & $11\, 34\, 11.68$ & $12\, 30\, 44.33$ & NGC 3731 & $3195 \pm 2 $ & $2.62$ & $-20.35$ & $10.31$\\
	$5828$ & $11\, 59\, 49.61$ & $30\, 50\, 39.92$ & IC 2986 & $3108 \pm 2 $ & $2.46$ & $-19.65$ & $10.00$\\
	$5839$ & $11\, 56\, 56.36$ & $60\, 19\, 45.89$ & CGCG 292-051 & $1391 \pm 2 $ & $1.33$ & $-16.76$ & $8.40$\\
	$5841$ & $11\, 44\, 24.49$ & $60\, 53\, 02.67$ & 2MASX J11442453+6053022 & $1497 \pm 1 $ & $1.45$ & $-16.42$ & $8.41$\\
	$5843$ & $11\, 56\, 07.08$ & $64\, 21\, 02.64$ & 2MASXi J1156072+642102 & $1410 \pm 1 $ & $1.77$ & $-16.34$ & $8.14$\\
	$5883$ & $12\, 09\, 22.26$ & $13\, 59\, 32.74$ & IC 3019 & $1675 \pm 14 $ & $2.17$ & $-18.16$ & $9.07$\\
	$5884$ & $12\, 20\, 24.30$ & $05\, 34\, 22.14$ & NGC 4282 & $937 \pm 3 $ & $2.50$ & $-17.14$ & $9.11$\\
	$5885$ & $12\, 15\, 12.56$ & $14\, 25\, 58.37$ & IC 3065 & $995 \pm 3 $ & $2.09$ & $-17.39$ & $8.94$\\
	$5888$ & $12\, 21\, 04.81$ & $11\, 45\, 16.56$ & IC 3192 & $1446 \pm 11 $ & $2.03$ & $-16.33$ & $8.41$\\
	$5889$ & $12\, 07\, 12.13$ & $63\, 53\, 26.64$ & MCG +11-15-024 & $1425 \pm 3 $ & $1.81$ & $-16.43$ & $8.39$\\
	$5913$ & $12\, 51\, 16.52$ & $53\, 41\, 46.66$ & IC 0830 & $4847 \pm 2 $ & $2.56$ & $-21.30$ & $10.67$\\
	$5921$ & $12\, 35\, 20.23$ & $06\, 06\, 54.33$ & NGC 4543 & $2374 \pm 1 $ & $2.41$ & $-19.48$ & $9.87$\\
	$5923$ & $12\, 30\, 10.32$ & $10\, 46\, 46.12$ & NGC 4482 & $1835 \pm 3 $ & $2.10$ & $-19.42$ & $9.57$\\
	$5926$ & $12\, 36\, 54.85$ & $12\, 31\, 12.27$ & IC 3586 & $1723 \pm 4 $ & $2.00$ & $-18.55$ & $9.17$\\
	$5931$ & $12\, 40\, 13.38$ & $12\, 52\, 29.19$ & IC 3635 & $1560 \pm 8 $ & $2.26$ & $-16.87$ & $8.69$\\
	$5936$ & $12\, 39\, 37.71$ & $10\, 58\, 32.68$ & VCC 1803 & $1355 \pm 21 $ & $2.48$ & $-15.88$ & $8.24$\\
	$5999$ & $13\, 48\, 34.66$ & $37\, 06\, 47.91$ & CGCG 190-059 & $10255 \pm 2 $ & $2.54$ & $-22.49$ & $11.11$\\
	$6016$ & $13\, 50\, 41.47$ & $40\, 16\, 45.63$ & CGCG 218-060 & $2300 \pm 2 $ & $2.57$ & $-18.66$ & $9.62$\\
	$6025$ & $13\, 58\, 42.89$ & $61\, 51\, 45.53$ & MCG +10-20-057 & $1795 \pm 2 $ & $1.51$ & $-16.24$ & $8.16$\\
	$6060$ & $14\, 01\, 24.02$ & $36\, 48\, 00.32$ & Mrk 0465 & $2693 \pm 2 $ & $1.75$ & $-18.99$ & $9.39$\\
	$6070$ & $14\, 00\, 58.24$ & $55\, 34\, 05.19$ & ASK 301537 & $1842 \pm 10 $ & $1.68$ & $-16.23$ & $8.22$\\
	$6086$ & $14\, 54\, 32.75$ & $02\, 57\, 59.13$ & NGC 5776 & $8165 \pm 3 $ & $2.74$ & $-22.65$ & $11.22$\\
	$6107$ & $14\, 45\, 15.84$ & $00\, 09\, 34.17$ & ASK 8160 & $1664 \pm 4 $ & $1.60$ & $-16.87$ & $8.40$\\
	$6111$ & $14\, 42\, 16.49$ & $60\, 52\, 22.36$ & 2MASX J14421771+6052290 & $2292 \pm 2 $ & $1.15$ & $-16.87$ & $8.33$\\
	$6128$ & $15\, 23\, 35.25$ & $09\, 20\, 46.14$ & CGCG 077-110 & $10703 \pm 2 $ & $2.69$ & $-22.45$ & $11.22$\\
	$6157$ & $15\, 12\, 24.05$ & $02\, 04\, 48.23$ & ASK 84838 & $1682 \pm 10 $ & $2.00$ & $-16.04$ & $8.32$\\
	$6392$ & $21\, 15\, 16.19$ & $09\, 53\, 47.21$ & ASK 138334 & $5239 \pm 1 $ & $0.97$ & $-17.38$ & $8.38$\\
	$6422$ & $21\, 45\, 22.59$ & $12\, 16\, 06.34$ & ASK 139520 & $5777 \pm 4 $ & $1.35$ & $-17.12$ & $8.21$\\
	$6483$ & $23\, 24\, 23.54$ & $15\, 26\, 36.37$ & 2MASX J23242356+1526362 & $7658 \pm 2 $ & $2.59$ & $-20.49$ & $10.41$\\
	$6494$ & $23\, 19\, 09.42$ & $15\, 43\, 37.30$ & LSBC F677-02 & $4429 \pm 1 $ & $1.31$ & $-18.26$ & $8.82$\\
	$6498$ & $23\, 16\, 03.79$ & $13\, 47\, 05.74$ & ASK 143916 & $4504 \pm 6 $ & $1.63$ & $-16.81$ & $8.38$\\
	$6508$ & $23\, 41\, 25.92$ & $00\, 39\, 43.89$ & 2MASX J23412592-0039437 & $10864 \pm 2 $ & $2.77$ & $-20.93$ & $10.68$\\
	$6510$ & $23\, 53\, 31.01$ & $00\, 44\, 24.61$ & CGCG 381-058 & $6925 \pm 3 $ & $2.72$ & $-20.51$ & $10.57$\\
	$6512$ & $23\, 48\, 45.08$ & $15\, 55\, 43.45$ & KUG 2346+156 & $7848 \pm 10 $ & $1.73$ & $-20.20$ & $9.93$\\
	$6513$ & $23\, 40\, 32.70$ & $00\, 33\, 03.84$ & 2MASXJ23403276-0033029 & $6928 \pm 3 $ & $1.52$ & $-20.07$ & $9.57$\\
	$6546$ & $07\, 40\, 42.64$ & $23\, 37\, 34.47$ & CGCG 117-065 & $7343 \pm 2 $ & $2.76$ & $-21.17$ & $10.76$\\
	$6555$ & $07\, 36\, 44.69$ & $42\, 26\, 37.39$ & 2MASX J07364472+4226376 & $6971 \pm 2 $ & $2.51$ & $-20.21$ & $10.31$\\
	$6562$ & $07\, 33\, 27.72$ & $41\, 53\, 08.78$ & 2MASX J07332776+4153084 & $5888 \pm 2 $ & $2.30$ & $-19.35$ & $9.82$\\
	$6572$ & $07\, 37\, 59.17$ & $33\, 56\, 27.05$ & ASK 85066 & $7108 \pm 2 $ & $1.62$ & $-17.83$ & $8.87$\\
	$6573$ & $07\, 36\, 59.47$ & $30\, 29\, 53.49$ & PGC 1906163 & $4546 \pm 2 $ & $1.35$ & $-17.25$ & $8.54$\\
	$6607$ & $11\, 23\, 01.61$ & $38\, 31\, 11.97$ & 2MASXJ11230157+3831120 & $1858 \pm 3 $ & $2.07$ & $-17.05$ & $8.70$\\
	$6735$ & $08\, 33\, 55.25$ & $47\, 08\, 03.99$ & CGCG 237-006 & $4474 \pm 2 $ & $2.25$ & $-19.67$ & $9.95$\\
	$6741$ & $08\, 39\, 00.68$ & $40\, 20\, 45.98$ & UGC 04513 & $7410 \pm 2 $ & $2.74$ & $-21.74$ & $10.88$\\
	$6747$ & $08\, 46\, 45.23$ & $06\, 57\, 35.86$ & UGC 04594 & $8732 \pm 3 $ & $2.60$ & $-21.91$ & $11.01$\\
	$6748$ & $08\, 47\, 49.73$ & $18\, 54\, 42.83$ & IC 2399 & $4225 \pm 7 $ & $1.98$ & $-18.87$ & $9.44$\\
	$6759$ & $13\, 57\, 29.53$ & $09\, 57\, 03.24$ & CGCG 074-017 & $6969 \pm 2 $ & $2.39$ & $-20.53$ & $10.29$\\
